# Supplementary material for: Incentivizing Compliance with Algorithmic Instruments
Source: arXiv:2107.10093 source file (2021-07-28)
Supplement: Supplementary file 1 [file appendix-two-arms-two-types.tex]

\section{Omitted Proofs}
\subsection{Sampling Stage}
In this section, we prove that the sampling stage algorithm (Algorithm~\ref{alg:sampling-two-types}) in the two-arm two-type setting in Section~\ref{sec:sampling-two-arms-two-types} is BIC for a given type $i$. Before demonstrating this, recall that a type $i$, the event:
\begin{equation}
    \xi_i = \left\{ \frac{1}{L_1}\sum_{t = 1}^{L_1} y^1_t + \frac{1}{2} + \Upsilon + \sigma_\epsilon \sqrt{\frac{2\log(1/\delta)}{L_1}} < \mu^2_i \right\},
\end{equation}
with probability at least $1-\delta$ for confidence $\delta > 0$. Now, recall Lemma~\ref{lemma:bic-sampling-two-arms}:
\bicsamplingtwoarms*
\begin{proof} Let $\displaystyle G_{L_1} := \E_{\cP_i}[\theta^2 - \theta^1|S_{1, L_1}]$. It is sufficient to show that $\displaystyle \E_{\cP_i}[G_{L_1}|z_t = \e_2]\Prob_{\cP_i}[z_t = \e_2] \geq 0$ (by \eqref{claim:bic-equiv}).
\begin{claim}
\label{claim:bic-equiv}
Assume that we have $\displaystyle \E_{\cP_i}[\theta^2 - \theta^1|z_t = \e_2]\Prob_{\cP_i}[z_t = \e_2] \geq 0$. Then we also have $\displaystyle \E_{\cP_i}[\theta^1 - \theta^2|z_t = \e_1]\Prob_{\cP_i}[z_t = \e_1] \geq 0$.
\end{claim}
\begin{proof}
Algorithm~\ref{alg:sampling-two-types} is designed in a way such that we always have $\Prob_{\cP_i}[z_t = \e_2] > 0$.\\
Similarly, assume that we also recommend arm 1 with some positive probability: $\Prob_{\cP_i}[z_t = \e_1] > 0$. Assume that the expected difference in mean rewards $\displaystyle \E_{\cP_i}[\theta^2 - \theta^1]\leq 0$. Then, we have:
\begin{align*}
    0 &\geq \E_{\cP_i}[\theta^2 - \theta^1] \\
    &= \E_{\cP_i}[\theta^2 - \theta^1|z_t = \e_2]\Prob_{\cP_i}[z_t = \e_2] + \E_{\cP_i}[\theta^2 - \theta^1|z_t = \e_1]\Prob_{\cP_i}[z_t = \e_1]
\end{align*}
Since, by assumption, the product $\displaystyle \E_{\cP_i}[\theta^2 - \theta^1|z_t = \e_2]\Prob[z_t=\e_2] \geq 0$, it must be that the product 
\[\E_{\cP_i}[\theta^2 - \theta^1|z_t = \e_1]\Prob_{\cP_i}[z_t = \e_1] \leq 0.\] 
Reversing the order of operands, we have that
$\E_{\cP_i}[\theta^1 - \theta^2|z_t = \e_1]\Prob_{\cP_i}[z_t = \e_1] \geq 0.$
\end{proof}
Note that we have 
\begin{align*}
&\quad	\E_{\cP_i}[G_{L_1} | z_t = \e_2] \Prob_{\cP_i}[z_t = \e_2] \\
	&= \E_{\cP_i}[G_{L_1} |z_t = \e_2 \ \& \ p_t \in P-Q]\Prob_{\cP_i}[z_t = \e_2 \ \& \ p_t \in P-Q] \\
	& \hspace{.4cm} + \E_{\cP_i}[G_{L_1}|z_t = \e_2 \ \& \ p_t \in Q]\Prob_{\cP_i}[z_t = \e_2 \ \& \ p_t \in Q]\\
	&= \E_{\cP_i}[G_{L_1} | \xi_2]\Prob_{\cP_i}[\xi_i]\left(1 - \frac{1}{\rho} \right) + \E_{\cP_i}[G_{L_1}|z_t = \e_2 \ \& \ p_t \in Q]\Prob_{\cP_i}[z_t = \e_2 \ \& \ p_t \in Q]\\
	&= \E_{\cP_i}[G_{L_1} | \xi_i]\Prob_{\cP_i}[\xi_i]\left(1 - \frac{1}{\rho} \right) + \E_{\cP_i}[G_{L_1}|p_t\in Q]\Prob_{\cP_i}[p_t \in Q], \ \ \text{(by definition $p_t\in Q \Rightarrow z_t=\e_2$)}\\
	&= \E_{\cP_i}[G_{L_1} | \xi_i]\Prob_{\cP_i}[\xi_i]\left(1 - \frac{1}{\rho} \right) + \E_{\cP_i}[\theta^2 - \theta^1 | p_t\in Q]\Prob_{\cP_i}[p_t \in Q] \ \ \text{(by Law of Total Expectation)}\\
	&= \E_{\cP_i}[G_{L_1} | \xi_i]\Prob_{\cP_i}[\xi_i]\left(1 - \frac{1}{\rho} \right) + \E_{\cP_i}[\theta^2 - \theta^1]\Prob_{\cP_i}[p_t \in Q] \\
	&= \E_{\cP_i}[G_{L_1} | \xi_i]\Prob_{\cP_i}[\xi_i]\left(1 - \frac{1}{\rho} \right) + (\mu_i^2 - \mu_i^1)\Prob_{\cP_i}[p_t \in Q]\\
	&= \E_{\cP_i}[G_{L_1} | \xi_i]\Prob_{\cP_i}[\xi_i]\left(1 - \frac{1}{\rho} \right) + \frac{1}{\rho}(\mu_i^2 - \mu_i^1)
\end{align*}
For the algorithm to be BIC for type $i$, we need to pick $\rho$:
\begin{align}
	\E_{\cP_i}[G_{L_1} | \xi_i]\Prob_{\cP_i}[\xi_i]\left(1 - \frac{1}{\rho} \right) + \frac{1}{\rho}(\mu_i^2 - \mu_i^1) &\geq 0 \nonumber\\
	\E_{\cP_i}[G_{L_1} | \xi_i]\Prob_{\cP_i}[\xi_i] - \frac{1}{\rho}\E_{\cP_i}[G_{L_1}|\xi_i] \Prob_{\cP_i}[\xi_i] + \frac{1}{\rho}(\mu_i^2 - \mu_i^1) &\geq 0 \nonumber\\
	\rho\E_{\cP_i}[G_{L_1}|\xi_i]\Prob_{\cP_i}[\xi_i] &\geq \E_{\cP_i}[G_{L_1} | \xi_i]\Prob_{\cP_i}[\xi_i] - (\mu_i^2 - \mu_i^1) \nonumber\\
	\rho &\geq 1 + \frac{\mu_i^1 - \mu_i^2}{\E_{\cP_i}[G_{L_1} | \xi_i]\Prob_{\cP_i}[\xi_i]} 
	\label{eq:L-condition}
\end{align}

This comes down to finding a lower bound on the denominator of the expression above. First, we define a clean event $C'$ where the average error $\frac{1}{L_1}\sum_{i=1}^{L_1} \epsilon_i$ is bounded (following Corollary \ref{thm:high-prob-unbounded-chernoff}):
\begin{equation}
     C' := \left \{ \bigg\vert\frac{1}{L_1} \sum_{i=1}^{L_1} \epsilon_i \bigg\vert \leq \sigma_\epsilon \sqrt{\frac{2\log(1/\delta)}{L_1}} \right \}.
\end{equation}
The event $C'$ occurs with probability at least $1 - \delta$ for $\displaystyle \delta < \delta' := \frac{\Prob_{\cP_i}[\xi_i]}{8}$.

We have 
\begin{align}
    \E_{\cP_i}[G_{L_1} | \xi_i] \Prob_{\cP_i}[\xi_i] &= \E_{\cP_i}[G_{L_1} | \xi_i, C'] \Prob_{\cP_i}[\xi_i, C'] + \E_{\cP_i}[G_{L_1} | \xi_i, \neg C'] \Prob_{\cP_i}[\xi_i, \neg C'] \nonumber\\
    &\geq \E_{\cP_i}[G_{L_1} | \xi_i, C'] \Prob_{\cP_i}[\xi_i, C'] - \delta \tag{since $G_{L_1} \geq -1$ and $\Prob_{\cP_i}[\neg C']<\delta$} \nonumber\\
    &= \E_{\cP_i}[G_{L_1} | \xi_i, C'] (\Prob_{\cP_i}[\xi_i] - \Prob_{\cP_i}[\xi_i, \neg C']) - \delta \nonumber\\
    &\geq \E_{\cP_i}[G_{L_1} | \xi_i, C'] (\Prob_{\cP_i}[\xi_i] - \Prob_{\cP_i}[\neg C']) - \delta \nonumber\\
    &\geq \E_{\cP_i}[G_{L_1} | \xi_i, C'] (\Prob_{\cP_i}[\xi_i] - \delta) - \delta \nonumber\\
    &= \E_{\cP_i}[G_{L_1} | \xi_i, C'] \Prob_{\cP_i}[\xi_i] - \delta(1 + \E_{\cP_i}[G_{L_1} | \xi_i, C']) \nonumber\\
    &\geq \E_{\cP_i}[G_{L_1} | \xi_i, C'] \Prob_{\cP_i}[\xi_i] - 2\delta \label{eq:sampling-two-arm-clean-event}
\end{align}

This comes down to finding a lower bound on the denominator of the expression above. We can reduce the dependency of the denominator to a single prior-dependent constant $\Prob_{\cP_i}[\xi_i]$ if we lower bound the prior-dependent expected value $\E_{\cP_i}[G_{L_1} | \xi_i]$. That way, assuming we know the prior and can calculate the probability of event $\xi_i$, we can pick an appropriate $\rho$ to satisfy the BIC condition for all agents of type $i$. Remember that event $\xi_i = \{ \bar{y}^1_{L_1} + C < \mu^2_i\}$ where $C = \Upsilon + \sigma_{\epsilon}\sqrt{\frac{2\log(1/\delta)}{L_1}} + \frac{1}{2}$ and $\displaystyle G_{L_1} := \E_{\cP_i}[\theta^2 - \theta^1|S_{1, L_1}]$. Then, the expected value
\begin{align}
    \E_{\cP_i}[G_{L_1} | \xi_i, C'] 
    &= \E_{\cP_i}[\E_{\cP_i}[\theta^2 - \theta^1|S_{1, L_1}] | \xi_i, C'] \nonumber\\
    &= \mu_i^2 - \E_{\cP_i}\left[\theta^1 \middle| \Upsilon + \sigma_{\epsilon}\sqrt{\frac{2\log(1/\delta)}{L_1}} + \frac{1}{2}  + \bar{y}^1_{L_1}< \mu_i^2, C'\right] \nonumber\\
    &= \mu_i^2 - \E_{\cP_i}\left[\theta^1 \middle| \Upsilon + \sigma_{\epsilon}\sqrt{\frac{2\log(1/\delta)}{L_1}} + \frac{1}{2}  +  \frac{1}{L_1}\sum_{t=1}^{L_1} y_t^1< \mu_i^2, C'\right] \nonumber\\
    &= \mu_i^2 - \E_{\cP_i}\left[\theta^1 \middle| \Upsilon + \sigma_{\epsilon}\sqrt{\frac{2\log(1/\delta)}{L_1}} + \frac{1}{2}  + \frac{1}{L_1}\sum_{t=1}^{L_1} \theta^1 + g(u_t) + \epsilon_t  < \mu_i^2, C'\right] \nonumber\\
    &= \mu_i^2 - \E_{\cP_i}\left[\theta^1 \middle| \theta^1 + \Upsilon + \sigma_{\epsilon}\sqrt{\frac{2\log(1/\delta)}{L_1}} + \frac{1}{2} + \frac{1}{L_1}\sum_{t=1}^{L_1} g(u_t) + \epsilon_t  < \mu_i^2, C'\right] \nonumber\\
    &> \mu_i^2 - \E_{\cP_i}\left[\theta^1 \middle| \theta^1 + \Upsilon + \sigma_{\epsilon}\sqrt{\frac{2\log(1/\delta)}{L_1}} + \frac{1}{2} - \Upsilon - \sigma_{\epsilon}\sqrt{\frac{2\log(1/\delta)}{L_1}} < \mu_i^2\right] \tag{since $g(u_t) > -\Upsilon$ and $\frac{1}{L_1}\sum_{t=1}^{L_1}\epsilon_t > -\sigma_\epsilon \sqrt{\frac{2\log(1/\delta)}{L_1}}$ by event $C'$} \nonumber\\
    &> \mu_i^2 - \E_{\cP_i}\left[\theta^1 \middle| \theta^1 + \frac{1}{2} < \mu_i^2\right] \nonumber\\
    &> \frac{1}{2} 
    \label{eq:sampling-stage-two-arm-gap}
\end{align}
Hence, the lower bound on the denominator is
\begin{align}
    \E_{\cP_i}[G_{L_1} | \xi_i] \Prob_{\cP_i}[\xi_i] &\geq \E_{\cP_i}[G_{L_1} | \xi_i, C']\Prob_{\cP_i}[\xi_i] - 2\delta \tag{by Equation \ref{eq:sampling-two-arm-clean-event}}\\
    &> \frac{1}{2}\Prob_{\cP_i}[\xi_i] - 2\delta \tag{by Equation \ref{eq:sampling-stage-two-arm-gap}}\\
    &= \frac{1}{4}\Prob_{\cP_i}[\xi_i] + \frac{1}{4}\Prob_{\cP_i}[\xi_i] - 2\delta \\ 
    &= 2\delta' + \frac{\Prob_{\cP_i}[\xi_i]}{4} - 2\delta\tag{since $\delta' = \frac{1}{8} \Prob_{\cP_i}[\xi_i]$}\\
    &\geq \frac{\Prob_{\cP_i}[\xi_i]}{4} \tag{since $\delta < \delta'$}
\end{align}
Hence, we can pick :
\begin{align*}
    \rho &\geq 1 + \frac{4(\mu_i^1 - \mu_i^2)}{\Prob_{\cP_i}[\xi_i]}
\end{align*}
to satisfy the BIC condition for all agents of type $i$.
\end{proof}

\subsection{Racing Stage}
We recall \cref{lemma:racing-bic-two-types}:
\racingbictwotypes*

\begin{proof}
Let $\displaystyle G := \theta^2 - \theta^1$ and $\hat{G}_q := \hat{\theta}^2_q - \hat{\theta}^1_q$. Let 
\[s_q := 192\sqrt{\frac{\log(3T/\delta) + 3\log(2T(2+\Upsilon^2))}{q}}\] be the decision threshold for each phase $q \geq L_1$ in Algorithm~\ref{alg:racing-two-types}. Assume that after the elimination, at every iteration a sample of the eliminated arm is also drawn, but not revealed to the agent.\\
We define the event $\cC_1$ as the accuracy guarantee of $\hat{\theta}$ such that:
\begin{equation}
\label{eq:event-C-1}
    \cC_1 := \left\{ \forall q \geq L_1: |G - \hat{G}_q| < s_q \right\}
\end{equation}
where $L_1$ is the number of samples of each arm after running the sampling stage.\\
Let $X^2_q$ be the number of arm 2 samples in phase $q$. We also define event $\cC_2$ where there is at least one sample of arm 2 in each phase:
\begin{equation}
\label{eq:event-C-2}
    \cC_2 := \left\{\forall q: X^2_q \geq 1 \right\}
\end{equation}
Recall that half of the population is of type 1 and the other half is of type 2, and $h$ is the number of types a single arm is recommended during a single phase. Then, if Algorithm~\ref{alg:racing-two-types} is BIC for all agents of type 2, we have $X^2_q \sim B(h,1/2)$. Hence, we have
\begin{equation}
    \Prob[X^2_q \geq 1] = 1 - \left(\frac{1}{2}\right)^h = \delta'.
\end{equation}

Let $\tau \in (0, 1)$. Fix phase $q \geq L_1$, and some agent $t$ in this phase. In order to prove that Algorithm~\ref{alg:racing-two-types} is BIC for all agents of type 2, we want to show that 
\begin{equation}
    \label{eq:racing-bic-arm2}
    \E_{\cP_2}[G\vert z_p = \e_2]\Prob_{\cP_2}[z_p = \e_2] \geq 0.
\end{equation}

Note that, by assumption, the parameter
\begin{align*}
    h &\geq \frac{\log\left(\frac{3\tau\Prob_{\cP_2}[G\geq\tau]+4}{4\tau\Prob_{\cP_2}[G\geq\tau]+4}\right)}{\log(1-p_2)}\\
    \Rightarrow \left(\frac{1}{2}
    \right)^h 
    &\geq \frac{3\tau\Prob_{\cP_2}[G\geq\tau]+4}{4\tau\Prob_{\cP_2}[G\geq\tau]+4}\\
    \Rightarrow \delta' = 1 - \left(\frac{1}{2}\right)^h 
    &\leq \frac{\tau\Prob_{\cP_2}[G\geq\tau]}{4\tau\Prob_{\cP_2}[G\geq\tau]+4}.
\end{align*}

From Corollary ~\eqref{cor:finite-sample}, with probability $\delta>0$ we have that
\begin{equation*}
    \Prob[\neg \cC_1 \vert G] \leq \delta
\end{equation*} 

Define event $\cC$ such that
\begin{equation}
\label{eq:event-C}
    \cC := \left\{ \forall q \geq L_1: \cC_1 \  \& \ \cC_2 \right\}
\end{equation}

Using union bound, we have
\begin{align}
    \Prob[\neg \cC \vert G] &\leq \Prob[\neg \cC_1 \vert G] + \Prob[\neg \cC_2 \vert G]\\
    &\leq \delta + \delta' \nonumber\\
    &\leq \delta_{\tau} + \delta' \nonumber \\
    &\leq \frac{\tau\Prob_{\cP_2}[G\geq\tau]}{4\tau\Prob_{\cP_2}[G\geq\tau]+4} + \frac{\tau\Prob_{\cP_2}[G\geq\tau]}{4\tau\Prob_{\cP_2}[G\geq\tau]+4} \nonumber \\
    &= \frac{\tau\Prob_{\cP_2}[G\geq\tau]}{2\tau\Prob_{\cP_2}[G\geq\tau]+2} \label{eq:delta'}
\end{align}
Therefore, since $G\geq -1$, we have: 
\begin{align*}
\label{eq:racing-bic}
    \E_{\cP_2}[G|z_p = \e_2]\Prob_{\cP_2}[z_p = \e_2] &= \E_{\cP_2}[G|z_p = \e_2, \cC]\Prob_{\cP_2}[z_p = 2, \cC] + \E_{\cP_2}[G|z_p = \e_2, \neg C]\Prob_{\cP_2}[z_p = \e_2, \neg C]\\
    &\geq \E_{\cP_2}[G|z_p = \e_2, \cC]\Prob_{\cP_2}[z_p = \e_2, \cC] - \frac{\tau\Prob_{\cP_2}[G\geq\tau]}{2\tau\Prob_{\cP_2}[G\geq\tau]+2} 
\end{align*}
We want to upper bound the first term. This can be done by splitting it into four cases based on the value of $G$. We have:

\begin{equation} 
    \begin{split}
    \E_{\cP_2}[G | z_p = \e_2, \cC]\Prob_{\cP_2}[z_p = \e_2, \cC] = 
    &\E_{\cP_2}[G | z_p = \e_2, \cC, G \geq \tau]\Prob_{\cP_2}[z_p= \e_2, \cC, G \geq \tau] \\
    &\ + \E_{\cP_2}[G | z_p = \e_2, \cC, 0 \leq G < \tau]\Prob_{\cP_2}[z_p = \e_2, \cC, 0 \leq G < \tau] \\
    &\ + \E_{\cP_2}[G | z_p = \e_2, \cC, -2s_q < G < 0]\Prob_{\cP_2}[z_p = \e_2, \cC, -2s_q < G < 0] \\
    &\ + \E_{\cP_2}[G | z_p = \e_2, \cC, G \leq -2s_q]\Prob_{\cP_2}[z_p = \e_2, \cC, G \leq -2s_q] \label{eq:racing-bic-cases}
    \end{split}
\end{equation}

Observe that, by definition of $s_q$, we have:
\begin{align*}
    2s_q &\leq 2s_{L_1}
    = \frac{384\sqrt{\log(3T/\delta) + 3\log(2T(2+\Upsilon^2))} \ \tau \Prob_{\cP_2}[G \geq \tau] }{768\sqrt{(\log(3T/\delta) + 3\log(2T(2+\Upsilon^2)))}}\\
    &= \frac{\tau \Prob_{\cP_2}[G \geq \tau]}{2}\\
    &\leq \tau
\end{align*}

Conditional on $\cC$, the empirical estimate $\hat{G}_q > G - s_q \geq 2s_q$. Hence, when we have $G \geq \tau \geq 2s_q$, then $G=\theta^2 - \theta^1 \geq 2s_q$ and arm 1 must have already been eliminated at phase $q \geq L_1$. This implies that the probability $\Prob_{\cP_2}[z_p = \e_2, \cC, G\geq \tau] = \Prob_{\cP_2}[\cC, G\geq \tau]$. Similarly, when we have $G \leq -2s_q$, then $\theta^2 - \theta^1 \leq -2s_q$ and arm 2 must have already been eliminated at phase $q \geq L_1$. Hence, arm 2 could not be recommended in that case and the probability $\Prob_{\cP_2}[z_p = \e_2, \cC, G\leq-2s_q] = 0$.\\
We can then rewrite equation~\eqref{eq:racing-bic-cases} as
\begin{align*}
    \E_{\cP_2}[G | z_p = \e_2, \cC]\Prob_{\cP_2}[z_p = \e_2 ,\cC] \geq &\E_{\cP_2}[G | z_p = \e_2, \cC, G \geq \tau]\Prob_{\cP_2}[z_p= \e_2, \cC, G \geq \tau]\\
    &+ \E_{\cP_2}[G | z_p = \e_2, \cC, 0 \leq G < \tau]\Prob_{\cP_2}[z_p = \e_2, \cC, 0 \leq G < \tau]\\
    &+ \E_{\cP_2}[G | z_p = \e_2, \cC, -2s_q < G < 0]\Prob_{\cP_2}[z_p = \e_2, \cC, -2s_q < G < 0]\\
    \geq &\tau \Prob_{\cP_2}[\cC, G \geq \tau] + 0\cdot \Prob_{\cP_2}[\cC, 0 \leq G < \tau] -2s_q \Prob_{\cP_2}[z_p = \e_2, \cC, -2s_q<G<0]\\
    \geq &\tau \Prob_{\cP_2}[\cC, G \geq \tau] - 2s_q\\
    \geq &\tau \Prob_{\cP_2}[\cC, G \geq \tau] - \frac{\tau \Prob_{\cP_2}[G \geq \tau]}{2}\\
    \geq &\tau \Prob_{\cP_2}[\cC | G \geq \tau] \Prob_{\cP_2}[G \geq \tau] - \frac{\tau \Prob_{\cP_2}[G \geq \tau]}{2}\\
    \geq &\tau (1 - (\delta + \delta')) \Prob_{\cP_2}[G \geq \tau] - \frac{\tau \Prob_{\cP_2}[G \geq \tau]}{2}\\
    = & \left(\frac{1}{2} - (\delta + \delta') \right) \tau \Prob_{\cP_2}[G \geq \tau]\\
    \geq & \left(\frac{1}{2} - \frac{\frac{1}{2} \tau \Prob_{\cP_2}[G \geq \tau]}{\tau \Prob_{\cP_2}[G \geq \tau] + 1} \right) \tau \Prob_{\cP_2}[G \geq \tau] \tag{by Equation~\eqref{eq:delta'}}\\
    = & \frac{1}{2} \left(\frac{\tau \Prob_{\cP_2}[G\geq \tau] + 1 - \tau \Prob_{\cP_2}[G\geq \tau]}{\tau \Prob_{\cP_2}[G\geq \tau] + 1} \right)\tau \Prob_{\cP_2}[G\geq \tau]\\
    = & \frac{1}{2} \left(\frac{\tau \Prob_{\cP_2}[G\geq \tau]}{\tau \Prob_{\cP_2}[G\geq \tau] + 1} \right)
\end{align*}
Hence, we have 
\begin{align*}
    \E_{\cP_2}[G|z_p = \e_2]\Prob_{\cP_2}[z_p = \e_2] &\geq \E[G|z_p = \e_2, \cC]\Prob_{\cP_2}[z_p = \e_2, \cC] - \frac{\tau\Prob_{\cP_2}[G\geq\tau]}{2\tau\Prob_{\cP_2}[G\geq\tau]+2} \\
    &\geq \frac{\tau\Prob_{\cP_2}[G\geq\tau]}{2\tau\Prob_{\cP_2}[G\geq\tau]+2}  -  \frac{\tau\Prob_{\cP_2}[G\geq\tau]}{2\tau\Prob_{\cP_2}[G\geq\tau]+2} \\
    &= 0
\end{align*}
Therefore, Algorithm~\ref{alg:racing-two-types} fulfills equation~\eqref{eq:racing-bic-arm2} and is BIC for all agents of type 2.
\end{proof}

%%%%%%%%%%%%%%%%%%%%%%%%%%%%%%%%%%%%%%%%%%%%%%
%%%%%%%%%%%%%%%%%%%%%%%%%%%%%%%%%%%%%%%%%%%%%%
\bigskip

We recall Lemma~\ref{lemma:racing-bic-two-types-type-1}:
\racingbictwotypestypeone*

\begin{proof}
After collecting more samples of arm 2 in the first part of the racing stage, we can also convince agents of type 1 to follow our recommendations for arm 2 in the second part of the racing stage.
Let $\displaystyle G := \theta^2 - \theta^1$ and $\hat{G}_q := \hat{\theta}^2_q - \hat{\theta}^1_q$. Let 
\[s_q := 192\sqrt{\frac{\log(3T/\delta) + 3\log(2T(2+\Upsilon^2))}{q}}\] be the decision threshold for each phase $q \geq L_1$ in Algorithm~\ref{alg:racing-two-types}. Assume that after the elimination, at every iteration a sample of the eliminated arm is also drawn, but not revealed to the agent.\\
We define the event $\cC$ as the accuracy guarantee of $\hat{\theta}$ such that:
\begin{equation}
\label{eq:event-C}
    \cC := \left\{ \forall q \geq L_1: |G - \hat{G}_q| < s_q \right\}
\end{equation}
where $L_1$ is the number of samples of each arm after running the sampling stage.\\
Let $\tau \in (0, 1)$. Fix phase $q \geq L_1$, and some agent $t$ in this phase. In order to prove that Algorithm~\ref{alg:racing-two-types} is BIC for agents of type 1, we want to show that 
\begin{equation}
    \label{eq:racing-bic-arm2}
    \E_{\cP_1}[G\vert z_p = \e_2]\Prob_{\cP_1}[z_p = \e_2] \geq 0.
\end{equation}
From Corollary ~\eqref{cor:finite-sample}, with probability $\delta$ we have that
\begin{equation*}
    \Prob[\neg \cC \vert G] \leq \delta
\end{equation*} 
Therefore, since $G\geq -1$, we have: 
\begin{align*}
\label{eq:racing-bic}
    \E_{\cP_1}[G|z_p = \e_2]\Prob_{\cP_1}[z_p = \e_2] &= \E_{\cP_1}[G|z_p = \e_2, \cC]\Prob_{\cP_1}[z_p = \e_2, \cC] + \E_{\cP_1}[G|z_p = \e_2, \neg C]\Prob_{\cP_1}[z_p = \e_2, \neg C]\\
    &\geq \E_{\cP_1}[G|z_p = \e_2, \cC]\Prob_{\cP_1}[z_p = \e_2, \cC] - \delta
\end{align*}
We want to lower bound the first term. This can be done by splitting it into four cases based on the value of $G$. We have:

\begin{equation} 
    \begin{split}
    \E_{\cP_1}[G | z_p = \e_2, \cC]\Prob_{\cP_1}[z_p = \e_2, \cC] = 
    &\E_{\cP_1}[G | z_p = \e_2, \cC, G \geq \tau]\Prob_{\cP_1}[z_p= \e_2, \cC, G \geq \tau] \\
    &\ + \E_{\cP_1}[G | z_p = \e_2, \cC, 0 \leq G < \tau]\Prob_{\cP_1}[z_p = \e_2, \cC, 0 \leq G < \tau] \\
    &\ + \E_{\cP_1}[G | z_p = \e_2, \cC, -2s_q < G < 0]\Prob_{\cP_1}[z_p = \e_2, \cC, -2s_q < G < 0] \\
    &\ + \E_{\cP_1}[G | z_p = \e_2, \cC, G \leq -2s_q]\Prob_{\cP_1}[z_p = \e_2, \cC, G \leq -2s_q] \label{eq:racing-bic-cases}
    \end{split}
\end{equation}

Observe that, by definition of $s_q$, we have:
\begin{align*}
    2s_q &\leq 2s_{L_1}
    = \frac{384\sqrt{\log(3T/\delta) + 3\log(2T(2+\Upsilon^2))} \ \tau \Prob_{\cP_1}[G \geq \tau] }{768\sqrt{(\log(2T/\delta) + 3\log(2T(2+\Upsilon^2)))} \ }\\
    &= \frac{\tau \Prob_{\cP_1}[G \geq \tau]}{2}\\
    &\leq \tau
\end{align*}

Conditional on $\cC$, the empirical estimate $\hat{G}_q > G - s_q \geq 2s_q$. Hence, when we have $G \geq \tau \geq 2s_q$, then $G=\theta^2 - \theta^1 \geq 2s_q$ and arm 1 must have already been eliminated at phase $q \geq L_1$. This implies that the probability $\Prob_{\cP_1}[z_p = \e_2, \cC, G\geq \tau] = \Prob_{\cP_1}[\cC, G\geq \tau]$. Similarly, when we have $G \leq -2s_q$, then $\theta^2 - \theta^1 \leq -2s_q$ and arm 2 must have already been eliminated at phase $q \geq L_1$. Hence, arm 2 could not be recommended in that case and the probability $\Prob_{\cP_1}[z_p = \e_2, \cC, G\leq-2s_q] = 0$.\\
We can then rewrite equation~\eqref{eq:racing-bic-cases} as
\begin{align*}
    \E_{\cP_1}[G | z_p = \e_2, \cC]\Prob_{\cP_1}[z_p = \e_2 ,\cC] \geq &\E_{\cP_1}[G | z_p = \e_2, \cC, G \geq \tau]\Prob_{\cP_1}[z_p= \e_2, \cC, G \geq \tau]\\
    &+ \E_{\cP_1}[G | z_p = \e_2, \cC, 0 \leq G < \tau]\Prob_{\cP_1}[z_p = \e_2, \cC, 0 \leq G < \tau]\\
    &+ \E_{\cP_1}[G | z_p = \e_2, \cC, -2s_q < G < 0]\Prob_{\cP_1}[z_p = \e_2, \cC, -2s_q < G < 0]\\
    \geq &\tau \Prob_{\cP_1}[\cC, G \geq \tau] + 0\cdot \Prob_{\cP_1}[\cC, 0 \leq G < \tau] -2s_q \Prob_{\cP_1}[z_p = \e_2, \cC, -2s_q<G<0]\\
    \geq &\tau \Prob_{\cP_1}[\cC, G \geq \tau] - 2s_q\\
    \geq &\tau \Prob_{\cP_1}[\cC, G \geq \tau] - \frac{\tau \Prob_{\cP_1}[G \geq \tau]}{2}\\
    \geq &\tau \Prob_{\cP_1}[\cC | G \geq \tau] \Prob_{\cP_1}[G \geq \tau] - \frac{\tau \Prob_{\cP_1}[G \geq \tau]}{2}\\
    \geq &\tau (1 - \delta) \Prob_{\cP_1}[G \geq \tau] - \frac{\tau \Prob_{\cP_1}[G \geq \tau]}{2}\\
    = & \left(\frac{1}{2} - \delta \right) \tau \Prob_{\cP_1}[G \geq \tau]\\
    \geq & \left(\frac{1}{2} - \delta \right) \tau \Prob_{\cP_1}[G \geq \tau]\\
    = & \left(\frac{1}{2} - \frac{\frac{1}{2} \tau \Prob_{\cP_1}[G \geq \tau]}{\tau \Prob_{\cP_1}[G \geq \tau] + 1} \right) \tau \Prob_{\cP_1}[G \geq \tau]\\
    = & \frac{1}{2} \left(\frac{\tau \Prob_{\cP_1}[G\geq \tau] + 1 - \tau \Prob_{\cP_1}[G\geq \tau]}{\tau \Prob_{\cP_1}[G\geq \tau] + 1} \right)\tau \Prob_{\cP_1}[G\geq \tau]\\
    = & \frac{1}{2} \left(\frac{\tau \Prob_{\cP_1}[G\geq \tau]}{\tau \Prob_{\cP_1}[G\geq \tau] + 1} \right)\\
    = & \ \delta_\tau \\
    \geq & \ \delta .
\end{align*}
Hence, we have 
\begin{align*}
    \E_{\cP_1}[G|z_p = \e_2]\Prob_{\cP_1}[z_p = \e_2] &\geq \E[G|z_p = \e_2, \cC]\Prob_{\cP_1}[z_p = \e_2, \cC] - \delta\\
    &\geq \delta -  \delta \\
    &= 0
\end{align*}
Therefore, the second stage of Algorithm~\ref{alg:racing-two-types} fulfills equation~\eqref{eq:racing-bic-arm2} and is BIC for agents of type 1. 

Note that we restrict the priors of type 1 and type 2 such that $\delta_\tau^1 < \delta_\tau^2$. Then, with the same constant $\tau$, the BIC conditions for agents of type 2 is also satisfied, and we achieve a fully BIC algorithm.
\end{proof}

%%%%%%%%%%%%%%%%%%%%%%%%%%%%%%%%%%%%%%%%%%%%%%
%%%%%%%%%%%%%%%%%%%%%%%%%%%%%%%%%%%%%%%%%%%%%%

\subsection{Regret}
We recall \cref{lemma:ex-post-2-arm}:
\regrettwoarms*

\begin{proof}
From Theorem~\eqref{thm:finite-sample}, the \textit{clean event} $\cC_1$ happens with probability at least $1 - \delta$ for some $\delta \in (0,1)$. Hence, the probability of $\neg \cC_1$ is at most $\delta$. The probability of not getting an arm 2 sample in each phase, $\neg \cC_2$ is $\delta'$. Hence, the expected ex-post regret conditional on $\neg \cC$ is at most $T (\delta + \delta)'$.\\
Assume that $\cC$ holds. Let $\Delta = |\theta^1 - \theta^2|$. Observe that since $\cC$ holds, we have $\Delta \leq |\hat{G}_q| + s_q$ where $s_q$ is the decision threshold of phase $q$. Before the stopping criteria is invoked, we also have $|\hat{G}_q| \leq s_q$. 
%This, combined with the fact that the number of recommendations $m$ equals the number of arms $k$, gives us that the empirical estimate $\hat{\Gamma}_t$ is the $m$-dimensional identity matrix at any round $t$. Thus, the minimum singular value $\sigma_{\min}(\hat{\Gamma}_t) = 1$. Then, during each iteration of the main loop, we have:
% \begin{align}
%     \Delta \leq 2 s_q &= 384\sqrt{\frac{\log(3T/\delta) + 3\log(2T(2+\Upsilon^2))}{q}}
%     \label{eq:delta-bound}
% \end{align}
Hence, we have: 
\begin{align*}
     \Delta \leq 2 s_q &= 384\sqrt{\frac{\log(3T/\delta) + 3\log(2T(2+\Upsilon^2))}{q}}\\
     \Rightarrow \frac{\Delta}{384\sqrt{\log(3T/\delta) + 3\log(2T(2+\Upsilon^2))}} &\leq \frac{1}{\sqrt{q}}\\
     \Rightarrow q &\leq \frac{147456 (\log(3T/\delta) + 3\log(2T(2+\Upsilon^2)))}{\Delta^2}
\end{align*}
Therefore, the main loop must end by phase $q = \frac{147456 (\log(3T/\delta) + 3\log(2T(2+\Upsilon^2)))}{\Delta^2}$.\\
During the racing stage, each phase we give out $2h$ recommendations for the two arms sequentially, so each arm gets recommended $h$ times. If arm 1 is indeed the best arm, then on average, the regret for each phase is $0.5h \Delta$. If arm 2 is the best arm, then on average, the regret for each phase is $1.5 h \Delta$. Conditional on event $\cC$, the arm $a^*$ at the end of the racing stage is the best arm so no more regret is collected after the racing stage is finished.\\
Then, if arm 1 is the best arm, the total accumulated regret for the racing stage is 
\begin{equation}
\label{eq:regret-arm-1}
    R_2(T) \leq \frac{73728h (\log(3T/\delta) + 3\log(2T(2+\Upsilon^2)))}{\Delta}
\end{equation}
On the other hand, if arm 2 is the best arm, the total accumulated regret for the racing stage is 
\begin{equation}
\label{eq:regret-arm-2}
    R_2(T) \leq \frac{221184h (\log(3T/\delta) + 3\log(2T(2+\Upsilon^2)))}{\Delta}
\end{equation}
Observe that the ex-post regret for each round $t$ of the entire algorithm (both the sampling stage and the racing stage) is at most that of the racing stage plus $\Delta$ per each round of the sampling stage. Alternatively, we can also upper bound the regret by $\Delta$ per each round of the algorithm. Therefore, we can derive the ex-post regret for the entire algorithm:
If arm 1 is the best arm, then the total regret of both
\cref{alg:sampling-two-types} and \cref{alg:racing-two-types} is:
\begin{align}
    R(T) &\leq \min \left \{L_1 \Delta + \frac{73728h (\log(3T/\delta) + 3\log(2T(2+\Upsilon^2)))}{\Delta}, T\Delta \right \}\\
    &\leq L_1 + O(\sqrt{T\log(T/\delta)}) 
\end{align}
If arm 2 is the best arm, then the total regret of both
\cref{alg:sampling-two-types} and \cref{alg:racing-two-types} is:
\begin{align}
    R(T) &\leq \min \left \{L_1 \rho \Delta + \frac{221184h (\log(3T/\delta) + 3\log(2T(2+\Upsilon^2)))}{\Delta}, T\Delta \right \}\\
    &\leq L_1 \rho + O(\sqrt{T\log(T/\delta)}) 
\end{align}
\end{proof}

%%%%%%%%%%%%%%%%%%%%%%%%%%%%%%%%%%%%%%%%%%%%%%
%%%%%%%%%%%% Expected Regret %%%%%%%%%%%%%%%%%
%%%%%%%%%%%%%%%%%%%%%%%%%%%%%%%%%%%%%%%%%%%%%%

We recall Lemma~\ref{lemma:expected-regret-two-arms}:
\expectedregrettwoarms*

\begin{proof}
From Theorem~\eqref{thm:finite-sample}, we have the probability that the \textit{clean event} $\cC_1$ happens is at least $1 - \delta$ for some $\delta \in (0,1)$. Hence, the probability of $\neg \cC_1$ is at most $\delta$. The probability of not getting an arm 2 sample in each phase, $\neg \cC_2$ is $\delta'$. Hence, The expected ex-post regret conditional on $\neg \cC$ is at most $T (\delta + \delta)'$.\\
Now, we can set parameters $\delta,\ L_1,$ and  $\rho$ in terms of the time horizon $T$, in order to obtain an expected regret bound strictly relative to $T$. First, we set $\delta = 1/T^2$. Thus, for arbitrary constants $\tau$ and $\Prob[G \geq \tau]$, we may set $T$ sufficiently large such that 
\[\delta + \delta'\leq \delta_{\tau} + \delta' = \frac{\tau \Prob[G \geq \tau]}{2\left( \tau \Prob[G \geq \tau] + 1 \right)}.\] 
    
Next, recall that $L_1$, the length of each phase in Stage 1, is lower-bounded by
\begin{align*}
    L_1 \geq \frac{589824(\log(3T/\delta) + 3\log(2T(2+\Upsilon^2)))}{\tau^2 (\Prob_{\cP_2}[G \geq \tau]^2)} = \frac{589824(\log(2T^3) + 3 \log(2T(2 + \Upsilon^2)))}{\tau^2 \Prob_{\cP_2}[G \geq \tau]^2}
\end{align*}
We can set $L_1 = \sqrt{T}$. Thus, for arbitrary constants $m$ and $c_1$, we can always find $T$ sufficiently large such that $L_1 \geq \frac{589824(\log(3T/\delta) + 3\log(2T(2+\Upsilon^2)))}{\tau^2 (\Prob_{\cP_2}[G \geq \tau]^2)}$.

Lastly, we set $\rho = \sqrt{\log(T)}$. Thus, for arbitrary constants $\mu^1_2, \mu^2_2, \Upsilon, \sigma_{\epsilon}$ and $\Prob[\xi_i]$, we may set $T$ sufficiently large such that 
\[ \rho \geq 1 + \frac{4(\mu^1_2 - \mu^2_2)}{\Prob[\xi_2]}\]

Therefore, the expected regret of our entire algorithm is:
\begin{align*}
    \E_{\cP_2}[R(T)] &= \E[R(T)|\neg \cC]\Prob[\neg \cC] + \E[R(T)|\cC]\Prob[\cC] \\
    &\leq T(\delta + \delta') + \left((L_1 + L_1\rho) + O(\sqrt{T\log(T)} \right)\\
    &= \frac{1}{T} + \left(\sqrt{T} + \sqrt{\log(T)}\sqrt{T} \right) + O\left( \sqrt{T\log(T)} \right)\\
    &= \frac{1}{T} + O\left( \sqrt{T\log(T)} \right) + O\left(\sqrt{T\log(T)} \right)\\
    &= O\left(\sqrt{T\log(T)} \right)
\end{align*}
\end{proof}

%%%%%%%%%%%%%%%%%%%%%%%%%%%%%%%%%%%%%%%%%%%%%%
%%%%%%%%%%% Type-Specific Regret %%%%%%%%%%%%%
%%%%%%%%%%%%%%%%%%%%%%%%%%%%%%%%%%%%%%%%%%%%%%

We recall Lemma~\ref{lemma:type-specific-two-arm}:
\typespecifictwoarms*

\begin{proof}
The regret of our algorithm, as given by Lemma~\eqref{lemma:ex-post-2-arm} is 
\begin{equation}
\label{eq:ex-post-2-arm}
    R(T) \leq L_1 (\rho + 1) + O(\sqrt{T\log(T/\delta)}) 
\end{equation}
where $L_1$ is the number of arm 2 samples collected in the sampling stage, $\rho$ is the number of phases in the sampling stage and $\delta$ is the accuracy guarantee of our estimate $\hat{\theta}$.\\
Let $L_{1,1}$ be the number of samples needed to make agents of type 1 follow our recommendation for arm 2. Half of the population is agents of type 1 and the other half is agents of type 2. We can derive type-specific regret for each type of agents using our algorithm conditioned on which arm is the best arm overall.
\begin{enumerate}
    \item If arm 1 is the best arm overall:\\
    Type 1 regret: Since agents of type 1 only take arm 1 until the algorithm has collected at least $L_{1,1}$ samples of arm 2, they accumulate no regret throughout the sampling stage and the first part of the racing stage when the algorithm is only BIC for agents of type 2. Hence, the regret for type 1 is then just the regret accumulated in the second part of the racing stage. 
    \begin{align}
        R_1 &\leq 0.5(2hq - L_{1,1} + L_1)\Delta \\
        &\leq O(\log(T/\delta))
    \end{align}
    Type 2 regret: Since our algorithms guarantee that agents of type 2 will always follow our recommendation, the regret of agents of type 2 is derived similar to the ex-post regret in Lemma~\eqref{lemma:ex-post-2-arm}
    \begin{equation}
        R_2 \leq 0.5L_1 + O(\sqrt{T\log(T/\delta)})    
    \end{equation}
    \item If arm 2 is the best arm overall:\\
    Type 1 regret: Since agents of type 1 only start taking our recommendation for arm 2 during the second part of the racing stage, the regret of type 1 is then the regret accumulated by all agents of type 1 in the sampling stage, the first part of the racing stage and the regret accumulated after agents of type 1 start taking our recommendation for arm 2. 
    \begin{align}
        R_1 &\leq 0.5(L_1 \rho + L_{1,1} - L_1)\Delta + O(\sqrt{T\log(T/\delta)})\\
        &\leq 0.5L_1 \rho + O(\log(T/\delta)) + O(\sqrt{T\log(T/\delta)})
    \end{align}
    Type 2 regret: Similar to the case where arm 1 is the best arm overall, the regret for agents of type 2 can be derived from the ex-post regret in Lemma~\eqref{lemma:ex-post-2-arm}
    \begin{align}
        R_2 \leq 0.5 L_1 \rho + O(\sqrt{T\log(T/\delta)})
    \end{align}
\end{enumerate}
\end{proof}

%%%%%%%%%%%%%%%%%%%%%%%%%%%%%%%%%%%%%%%%%%%%%%
%%%%%%%%%%%%%%%%%%%%%%%%%%%%%%%%%%%%%%%%%%%%%%

We recall Remark~\ref{remark:regret-comparison-2-arm}
\regretcomparisontwoarms*

\begin{proof}
We can derive these type-specific regret for an algorithm that is fully incentive-compatible, where we want every agent to follow our recommendations throughout the algorithm. To make agents of type 1 comply with our recommendations, we need to run the sampling stage until we have collected at least $L_{1,1}$ samples of arm 2 with a smaller exploration probability $\rho'$, where 
\begin{equation}
    \rho' \geq 1 + \frac{4(\mu_1^1 - \mu_2^1)}{\Prob[\xi_1]}
\end{equation}
Hence, the ex-post regret of the fully incentive-compatible is 
\begin{equation}
    R_{BIC}(T) \leq L_{1,1} (\rho' + 1) + O(\sqrt{T\log(T/\delta)})
\end{equation}
The type-specific regret for the fully incentive-compatible bandit algorithm is the proportion of agents of each type times the total accumulated regret since all agents follow our recommendations in the algorithm, which can be summarized as follows (for confidence $\delta>0$):

\begin{table}[ht]
\begin{tabular}{|l|l|}
\hline
Best arm/Type & Type-specific Regret \\ \hline
Arm 1: Type 1 &$\frac{294912(\log(3T/\delta) + 3\log(2T(2+\Upsilon^2)))}{\tau^2 (\Prob_{\cP_1}[G \geq \tau]^2)}+O(\sqrt{T\log(T/\delta)})$                      \\ \hline
Arm 1: Type 2 & $\frac{294912(\log(3T/\delta) + 3\log(2T(2+\Upsilon^2)))}{\tau^2 (\Prob_{\cP_1}[G \geq \tau]^2)} +O(\sqrt{T\log(T/\delta)})$                     \\ \hline
Arm 2: Type 1 & $\frac{294912(\log(3T/\delta) + 3\log(2T(2+\Upsilon^2)))}{\tau^2 (\Prob_{\cP_1}[G \geq \tau]^2)}\left( 1 + \frac{4(\mu_1^1 - \mu_2^1)}{\Prob[\xi_1]} \right) + O(\sqrt{T\log(T/\delta)})$                     \\ \hline
Arm 2: Type 2 & $\frac{294912(\log(3T/\delta) + 3\log(2T(2+\Upsilon^2)))}{\tau^2 (\Prob_{\cP_1}[G \geq \tau]^2)} \left( 1 + \frac{4(\mu_1^1 - \mu_2^1)}{\Prob[\xi_1]}\right) + O(\sqrt{T\log(T/\delta)})$                     \\ \hline
\end{tabular}
\caption{Type-Specific Regret for Two Arms \& Two Types with Fully BIC Algorithm}
\label{tab:type-specific-regret-fully-bic}
\end{table}
\ls{Need to put these regrets in terms of a common prior-dependent constant between the fully-BIC algorithm and our algorithm, to make it clear that our algorithm outperforms the full-BIC one in certain situations. Show the fully-BIC algorithm can have linear regret and our algorithm has sublinear regret depending on prior-dependent constants}

Compare the type-specific regret bounds of our algorithm (see Table~\ref{tab:type-specific-regret-heterogeneous}) versus the fully incentive-compatible algorithm (see Table~\ref{tab:type-specific-regret-fully-bic}). On the face of it, these regret bounds do not seem to differ asymptotically. However, the main advantage of our algorithm compared to the fully incentive-compatible algorithm is the shorter sampling stage. 
Since agents of type 1 heavily prefer arm 1 to arm 2, for a constant $\tau \in (0,1)$, it is harder for agents of type 1 to believe that arm 2 is better than arm 1 by some amount $\tau$ compared to agents of type 2. Thus, we have $\Prob_{\cP_1}[\theta^2 - \theta^1 > \tau] < \Prob_{\cP_2}[\theta^2 - \theta^1 > \tau]$. Hence, we have $L_{1,1} > L_1$ and the number of arm 2 samples needed to convince agents of type 2 is much smaller than that for agents of type 1. Similarly, we have that we have $\rho' > \rho$. This is because:
\begin{enumerate}[label=(\arabic*)]
    \item agents of type 1 has stronger preference for arm 1 compared to agents of type 2, i.e. $\mu^1_1 - \mu^2_1 > \mu^1_2 - \mu^2_2$; and
    \item the probability that arm 1 is doing so badly in the opening phase of the sampling stage that arm 2 can look better by comparison is smaller for agents of type 1 compared to agents of type 2, i.e. $\Prob[\xi_1] < \Prob[\xi_2]$.
\end{enumerate}
Overall, the sampling stage of our algorithm is shorter than that of the fully incentive-compatible algorithm. In fact, the minimum length of sampling stage of the fully-incentive compatible algorithm can be increased arbitrarily, depending on the prior of type 1. In the worst-case, the sampling stage must be so large that the fully-incentive compatible algorithm does not achieve sublinear regret. By contrast, our algorithm may still achieve sublinear regret in these cases.
\ls{Double-check this.} This advantage can be shown in an explicit example using Gaussian prior reward.
\end{proof}

\subsection{Gaussian Example}
We recall Example~\ref{ex:gaussian}:
\gaussian*

\begin{proof}
We analyze this example for the sampling stage and the racing stage separately. 
\begin{itemize}
    \item The sampling stage:\\
    Suppose that, in the sampling stage, an agent of type 1 is recommended arm 2. This means that either $\E_{\cP_2}[\theta^2 - \theta^1 | z_t = e_2] \geq 0$ or the agent is in the exploration set Q. Since the agent knows that they are not type 2 and knows that the prior is over the prior of type 2, the recommendation is not enough to make them take arm 2:
    \begin{equation}
        \E_{\cP_1}[\theta^2 - \theta^1 | z_t = e_2] < 0.
    \end{equation}
    Let $\xi_2$ denote the event where the mean reward $\bar{y}^1_t$ of arm 1 from phase 1 is much smaller than the prior mean reward $\mu^2_2$, i.e.
    \begin{equation}
        \xi_2 := \left\{ \E_{\cP_2}[\theta^1 | y^1_1, \dots, y^1_{L_1}] < \mu^2_2 \right\}.
    \end{equation}
    Now, suppose that an agent of type 2 is recommended arm 2. They know that this either means that event $\xi_2$ has happened and $\E_{\cP_2}[\theta^2 - \theta^1 | z_t = e_2] \geq 0$ or that the agent is in the exploration group $Q$. They know that the social planner has chosen some exploration probability $\rho$ such that 
    \begin{equation}
        \rho \geq 1 + \frac{4(\mu_2^1 - \mu_2^2)}{\Prob_{\cP_i}[\xi_i]}.
    \end{equation}
    
   The social planner needs to calculate the probability of event $\xi_2$, i.e.
    \begin{equation}
        \Prob_{\cP_2}[\xi_2] = \Prob_{\cP_2}[\E_{\cP_2}[\theta^1 | y^1_1, \dots, y^1_{L_1}] < \mu^2_2].
    \end{equation}
    In the worst case, the confounding term $g(u_t) = -\Upsilon$ for all $L_1$ rounds of phase 1. Assume this worst case, the reward for pulling arm 1 is 
    \begin{align}
        y^1_t = \theta^1 - \Upsilon + \epsilon_t
    \end{align}
    Let $\hat{y}^1_t = y^1_t + \Upsilon = \theta^1 + \epsilon^1_t$. In this case, the expected posterior 
    \begin{equation}
        \E_{\cP_2}[\theta^1|y^1_1, \dots, y^1_{L_1}] = \E_{\cP_2}[\theta^1|\hat{y}^1_1, \dots, \hat{y}^1_{L_1}]
    \end{equation}
    Under this assumption, the error $\epsilon_t \sim \cN(0, \rho_{1.2}^2)$ and $\theta^1 = \mu^1_2 + \zeta^1_2$ for $\zeta^1_2 \sim \cN(0, \sigma^2_{1,2})$. Thus, the reward $\hat{y}^1_t \sim \cN(\theta^1, \rho^2_{1,2})$ and the expected posterior 
    \begin{equation}
        \E_{\cP_2}[\theta^1|\hat{y}^1_1, \dots, \hat{y}^1_{L_1}] \sim \cN\left(\mu^1_2,\ \sigma^2_{1,2}\frac{L_1 \sigma^2_{1,2}}{\rho^2_{1,2} + L_1 \sigma^2_{1,2}}\right)
    \end{equation}
    Let the z-score $\zeta^2 := (\mu^2_2 - \mu^1_2)\left(\sigma^2_{1,2}\frac{L_1 \sigma^2_{1,2}}{\rho^2_{1,2} + L_1 \sigma^2_{1,2}}\right)^{-1/2}$. Then, we have
    \begin{align}
        \Prob_{\cP_2}[\E_{\cP_2}[\theta^1|\hat{y}^1_1, \dots, \hat{y}^1_{L_1}] \leq \mu^2_2] = \phi(\zeta^2) = \int_{-\infty}^{\zeta^2} \frac{1}{\sqrt{2\pi}} \exp\left(\frac{-1}{2}u^2\right) du.
    \end{align}
    Furthermore, for any sequence of samples $y^1_1, \dots, y^1_{L_1}$ from phase 1, the expected posterior 
    \begin{equation}
        \E_{\cP_2}[\theta^1|y^1_1, \dots, y^1_{L_1}] \leq \E_{\cP_2}[\theta^1|\hat{y}^1_1, \dots, \hat{y}^1_{L_1}].
    \end{equation}
    Hence, 
    \begin{align*}
        \Prob[\xi_2] &= \Prob_{\cP_1}[\E_{\cP_1}[\theta^1| y^1_1, \dots, y^1_{L_1}] \leq \mu^2_2] \geq \Prob_{\cP_1}[\E_{\cP_1}[\theta^1|\hat{y}^1_1, \dots, \hat{y}^1_{L_1}] \leq \mu^2_2]\\
        &= \int_{-\infty}^{\zeta^2} \frac{1}{\sqrt{2\pi}} \exp\left(\frac{-1}{2}u^2\right) du.
    \end{align*}
    \item The racing stage:
    In the first racing stage, only agents of type 2 comply with our recommendation for arm 2. Hence, when an agent of type 1 receives a recommendation for arm 2, this recommendation is not enough to convince them to follow our recommendation for arm 2. Hence, we have 
    \begin{equation}
        \E_{\cP_1}[\theta^2 - \theta^1 | z_t = e_2] = \E_{\cP_1}[\theta^2 - \theta^1] < 0.
    \end{equation}
    When an agent of type 2 receives a recommendation for arm 2, they would think that either arm 2 is definitely the best arm or the two arms are still racing against each other. Agents of type 2 know that the racing stage only starts when the social planner has collected sufficient samples of arm 2 in the sampling stage:
    \begin{equation}
        L_1 \geq \frac{589824(\log(3T/\delta) + 3\log(2T(2+\Upsilon^2)))}{\tau^2 (\Prob_{\cP_2}[\theta^2 - \theta^1 \geq \tau]^2)}
    \end{equation}
    and 
    \begin{equation}
        \delta < \delta_{\tau, 2} = \frac{\tau \Prob_{\cP_2}[\theta^2 - \theta^1 > \tau]}{2\tau \Prob_{\cP_2}[\theta^2 - \theta^1 > \tau] + 2}
    \end{equation}
    The constant that the social planner needs to calculate is then $\tau \Prob_{\cP_2}[\theta^2 - \theta^1 > \tau]$ for some fixed constant $\tau \in (0,1)$.\\
    Assume that we have Gaussian priors. Hence, we have 
    \begin{equation}
        \theta^2 - \theta^1 \sim \cN(\mu^2_2 - \mu^1_2, \sigma^2_{1.2} + \sigma^2_{2,2})
    \end{equation}
    Let $\zeta_2 = \frac{\mu^2_2 - \mu^1_2 - \tau}{\sqrt{\sigma^2_{1,2} + \sigma^2_{1,2}}}$. Then, 
    \begin{align}
        \Prob_{\cP_2}[\theta^2 - \theta^1 > \tau] &= 1 - \Prob_{\cP_2}[\theta^2 - \theta^1 < \tau]\\
        &= 1 - \phi(\zeta_2)\\
        &= \int^\infty_{\zeta_2} \frac{1}{\sqrt{2\pi}} \exp\left(\frac{-1}{2} u^2\right) du
    \end{align}
    During the first racing stage, the algorithm collects more samples of arm 2, until we have enough samples to also make agents of type 1 comply with our recommendation for arm 2.\\
    When an agent of type 1 receives a recommendation for arm 2 during the second racing stage, they know that the number of arm 2 samples is at least
    \begin{equation}
        L_{1,1} \geq \frac{589824(\log(3T/\delta) + 3\log(2T(2+\Upsilon^2)))}{\tau^2 (\Prob_{\cP_1}[\theta^2 - \theta^1 \geq \tau]^2)}
    \end{equation}
    Similar to the first racing stage, the social planner also needs to calculate the prior-dependent constant $\tau (\Prob_{\cP_1}[\theta^2 - \theta^1 \geq \tau]$.\\
    We have 
    \begin{equation}
        \theta^2 - \theta^1 \sim \cN(\mu^2_1 - \mu^1_1, \sigma^2_{1,1} + \sigma^2_{2,1})
    \end{equation}
    Let $\zeta_1 = \frac{\mu^2_1 - \mu^1_1 - \tau}{\sqrt{\sigma^2_{1,1} + \sigma^2_{2,1}}}$. Then, 
    \begin{align}
        \Prob_{\cP_1}[\theta^2 - \theta^1 > \tau] &= 1 - \Prob_{\cP_1}[\theta^2 - \theta^2 < \tau]\\
        &= 1 - \phi(\zeta_1)\\
        &= \int^\infty_{\zeta_1} \frac{1}{\sqrt{2\pi}} \exp\left(\frac{-1}{2} u^2\right) du
    \end{align}
    Also, we have 
    \begin{equation}
        \delta < \delta_{\tau, 1} =  \frac{\tau \Prob_{\cP_1}[\theta^2 - \theta^1 > \tau]}{2\tau \Prob_{\cP_1}[\theta^2 - \theta^1 > \tau] + 2}
    \end{equation}
    When an agent of type 2 receives a recommendation for arm 2, they would still comply since there are sufficient samples of arm 2 collected by the social planner (similar to the first racing stage).\\
    Since agents of type 1 prefer arm 1 more compared to agents of type 2, for a fixed constant $\tau \in (0,1)$, we have $\tau \Prob_{\cP_1}[\theta^2 - \theta^1 > \tau] < \tau\Prob_{\cP_2}[\theta^2 - \theta^1 > \tau]$. Hence, 
    \begin{equation}
        \delta_{\tau, 1} =  \frac{\tau \Prob_{\cP_1}[\theta^2 - \theta^1 > \tau]}{2\tau \Prob_{\cP_1}[\theta^2 - \theta^1 > \tau] + 2} < \frac{\tau \Prob_{\cP_2}[\theta^2 - \theta^1 > \tau]}{2\tau \Prob_{\cP_2}[\theta^2 - \theta^1 > \tau] + 2} = \delta_{\tau,2}
    \end{equation}
    Therefore, the social planner can pick $\delta < \delta_{\tau,1} < \delta_{\tau,2}$ in the second racing stage and satisfies both types' incentive-compatibility requirement.\\ 
    If we want to have a fully incentive-compatible algorithm in both the sampling stage and the racing stage, then we would need to collect at least $L_{1,1}$ samples of arm 2 in the samplings stage with the exploration probability $1/\rho'$ where 
    \begin{equation}
        \rho' \geq 1 + \frac{4(\mu_1^1 - \mu_1^2)}{\Prob[\xi_1]}
    \end{equation}
    Similar to how we derive the probability of $\xi_2$, we have the expected posterior 
    \begin{equation}
        \E_{\cP_1}[\theta^1|\hat{y}^1_1, \dots, \hat{y}^1_{L_1}] \sim \cN\left(\mu^1_1,\ \sigma^2_{1,1}\frac{L_1 \sigma^2_{1,1}}{\rho^2_{1,1} + L_1 \sigma^2_{1,1}}\right)
    \end{equation}
    Let the z-score $\zeta^1 := (\mu^2_1 - \mu^1_1)\left(\sigma^2_{1,1}\frac{L_1 \sigma^2_{1,1}}{\rho^2_{1,1} + L_1 \sigma^2_{1,1}}\right)^{-1/2}$. Then, we have
    \begin{equation}
        \Prob_{\cP_1}[\E_{\cP_1}[\theta^1|\hat{y}^1_1, \dots, \hat{y}^1_{L_1}] \leq \mu^2_1] = \phi(\zeta^1) = \int_{-\infty}^{\zeta^1} \frac{1}{\sqrt{2\pi}} \exp\left(\frac{-1}{2}u^2\right) du
    \end{equation}
    Since $\mu^2_1 - \mu^1_1 < \mu^2_2 - \mu^2_1$, we have $\zeta_1 < \zeta_2$ and hence $\Prob[\xi_1] < \Prob[\xi_2]$. Therefore, the number of phases in the sampling stage needed to convince agents of type 1 $\rho' > \rho$ and we would need to run the sampling stage for longer if we want to make agents of type 1 also comply to our arm 2 recommendation. 
\end{itemize}

An extreme instance of type 1's prior could lead to a scenario where it is impossible to make the algorithm incentive-compatible for agents of type 1 within the time horizon $T$. Suppose we have $\Prob_{\cP_1}[\theta^2 - \theta^1 > \tau] < \frac{1}{\sqrt{T}}$ for some $\tau \in (0, 1)$, then the number of arm 2 samples needed to make agents of type 1 comply in the racing stage is:
\begin{align*}
    L_{1,1} &\geq \frac{589824(\log(3T/\delta) + 3\log(2T(2+\Upsilon^2)))}{\tau^2 \left(\frac{1}{T} \right)}\\
    &= O(T)
\end{align*}
Hence, a fully incentive-compatible algorithm would not finish the sampling stage before the time horizon is up. Therefore, the regret accumulated for each type of agents would be linear.\\
On the other hand, our algorithm only relies on agents of type 2 to take our recommendation during the sampling stage and the racing stage. Hence, if we have $\frac{1}{\sqrt{\log(T)}} > \Prob_{\cP_2}[\theta^2 - \theta^1 > \tau] > \frac{1}{\sqrt{T}} > \Prob_{\cP_1}[\theta^2 - \theta^1 > \tau]$, then the number of arm 2 samples needed to make agents of type 2 comply in the racing stage is:
\begin{align*}
    L_1 &\geq \frac{589824(\log(3T/\delta) + 3\log(2T(2+\Upsilon^2)))}{\tau^2 (\Prob_{\cP_2}[\theta^2 - \theta^1 \geq \tau]^2)}\\
    &= O(\log(T))
\end{align*}  
Also, if we have the probability that for agents of type 2, the sample average of arm 1 in the first phase of the sampling stage is sufficiently smaller than the prior-mean reward of arm 2, ($\Prob[\xi_2]$) is larger than $\frac{1}{\sqrt{\log(T)}}$, then the number of phases in the sampling stage is:
\begin{align*}
    \rho &> 1 + \frac{4(\mu^1_2 - \mu^2_2)}{\Prob[\xi_2]}\\
    &= O(\sqrt{\log(T)})
\end{align*}
Then, we would still achieve sub-linear regret for each type with our algorithm, while a fully incentive-compatible algorithm would stay in the sampling stage and achieve linear regret:
\begin{table}[ht!]
\centering
    \begin{tabular}{c|c|c|c|}
        \multicolumn{2}{c}{} & \multicolumn{2}{c}{Type}\\\cline{3-4}
         \multicolumn{1}{c}{} &  & Type 1 & Type 2 \\\cline{2-4}
         Best Arm & Arm 1 & $O(\log(T/\delta))$ & $O(\log(T))+O(\log(T/\delta))$ \\\cline{2-4}
         & Arm 2 & $O(\log(T)^{3/2}) + O(\sqrt{T\log(T/\delta)})$ & $O(\log(T)^{3/2}) + O(\sqrt{T\log(T/\delta)})$ \\\cline{2-4}
    \end{tabular}
    \caption{Example: Type-Specific Regret for Two Arms \& Two Types with Partially-BIC Algorithm}
    \label{tab:type-specific-regret-example}
\end{table}
\\
\ls{We can modify the sampling stage prior dependent constants for type 1 to decrease the minimum exploration probability of type 1 so that the minimum length of the sampling stage for the fully-BIC algorithm is arbitrarily large. At the same time, the racing stage prior-dependent constants for type 1 can still allow our algorithm to let type 1 be BIC in the second racing stage. This would make the regret sublinear for our algorithm for both types, while the regret is linear for the fully-BIC algorithm.}

\end{proof}
