# Supplementary material for: Incentivizing Compliance with Algorithmic Instruments
Source: arXiv:2107.10093 source file (2021-07-28)
Supplement: Supplementary file 2 [file appendix.tex]

\newpage
\appendix
\section{IV Estimator Proof}
\subsection{Model}

The equations central to our model are expressed as such:

\begin{equation}
\left\{ \begin{array}{l}
            y_i = \langle \theta, x_i\rangle + g(u_i) + \epsilon_i\\
            x_i = f(u_i, z_i)
        \end{array}
\right.
\end{equation}
Here $y_i$ is the reward, given by treatment $x_i$, treatment effect $\theta$, zero-mean noise $\epsilon_i$, and unobserved confounding variable $g(u_i)$, which itself is a function of type $u_i$ for the agent in sample $i$. The treatment $x_i$ is given by instrument $z_i$ and unknown selection function $f(z_i, u_i)$. Our goal is to consistently estimate the treatment effect $\theta$. This is complicated by the unobserved confounding variable $g(u_i)$ and its correlation to the treatment $x_i$.

 We model a linear relationship between $x_i$ and $z_i$ by introducing a population mean choice matrix $\Gamma$ (as expressed in equation~\eqref{eq:gamma}). We can rewrite our equation modeling $x_i$ as such:
\begin{align*} 
    x_i 
    = \Gamma^\intercal z_i - \left(\Gamma^\intercal z_i - f(u_i, z_i) \right) 
    &= \Gamma^\intercal z_i + \eta_i\\
    &= \hat{\Gamma}^\intercal z_i + \left(\Gamma^\intercal z_i -  \hat{\Gamma}^\intercal z_i \right) + \eta_i,
\end{align*}
    where $\eta_i = f(u_i, z_i)-\Gamma^\intercal z_i$ and $\hat{\Gamma}$ is an empirical estimate of $\Gamma$ (see equation~\eqref{eq:gammahat}). Now $y_i$ is given as such:
\begin{align} 
    y_i &= \theta^\intercal \left( \hat{\Gamma}^\intercal z_i + \left(\Gamma^\intercal z_i -  \hat{\Gamma}^\intercal z_i \right) + \eta_i \right) + g(u_i) + \epsilon_i\\
    &= \beta^\intercal z_i + \nu_i + \theta^\intercal \eta_i + g(u_i) + \epsilon_i\\
    &= \beta^\intercal z_i + \E[g(u)]\cdot\mathbf{1} + \gamma_i + \nu_i \\
    &= (\beta^*)^\intercal \tilde{z}_i + \gamma_i + \nu_i \label{eq:y}
\end{align}
where $\beta = \hat{\Gamma} \theta$ and $\gamma_i = \theta^\intercal \eta_i + g(u_i) - \E[g(u)] + \epsilon_i$ and $\nu_i = \theta^\intercal (\Gamma - \hat{\Gamma})^\intercal z_i$ and $\beta^* = (\beta, \E[g(u)])$ and $\tilde{z}_i = (z_i, 1)$.\\

\subsection{Finite Sample Analysis} 
Given $n \in \mathbbm{R}$ samples $(z, X, y)_n$, we would like to bound the difference between the predicted exogenous mean treatment effect, denoted $\hat{\theta}_n$, and the true exogenous mean treatment effect $\theta$, i.e. we want to bound $\norm{\hat{\theta}_n -\theta}_2.$

\begin{theorem}
\label{thm:finite-sample}
    Given a sample set $(z_i, x_i, y_i)_n$, which contains $n$ samples of instrument $z$, treatment $X$, and reward $y$, we bound the difference between the true mean treatment effect $\theta$ and the mean treatment effect $\hat{\theta}_n$ derived via IV regression over $(z_i, x_i, y_i)_n$. Let $k$ be the number of arms and $\Upsilon$ be an upper bound on the confounding term $g(u_t)$. Suppose among the $n$ observations $p$ is the proportion of agents that follow our recommendations. For some confidence $\delta>0$, with probability at least $1 - \delta$:
    \begin{align*}
    \norm{\hat{\theta}_n - \theta}_2 
    \leq \frac{4\sqrt{\lambda (k + \Upsilon^2)} + 16\sqrt{2\log\left(3/\delta\right) + (k+1)\log\left( 1 + \frac{2n}{\lambda(k+1)}\right)}}{p\sqrt{2n_{\min}}}.
    \end{align*}
\end{theorem}

\begin{corollary}
\label{cor:finite-sample}
Given a sample set $(z_i, x_i, y_i)_n$, which contains $n$ samples of instrument $z$, treatment $X$, and reward $y$, we bound the difference between the true mean treatment effect $\theta$ and the mean treatment effect $\hat{\theta}_n$ derived via IV regression over $(z_i, x_i, y_i)_n$. Let $k$ be the number of arms and $\Upsilon$ be a upper bound on the confounding term $g(u_t)$. Suppose among the $n$ observations $p$ is the proportion of agents that follow our recommendations. For some confidence $\delta>0$, with probability at least $1 - \delta$:
    \begin{align*}
    \norm{\hat{\theta}_n - \theta}_2 
    \leq \frac{12\sqrt{2\log\left(3/\delta\right) + (k+1)\log (2n(k + \Upsilon^2))}}{p\sqrt{2n_{\min}}}.
    \end{align*}
\end{corollary}

We can estimate $\hat{\theta}_n$ via a generalization of Two-Stages Least Squares (2SLS). In this method, we let $\beta'=\Gamma\theta$. We get an empirical estimate of $\Gamma$, denoted $\hat{\Gamma}$, as in equation~\eqref{eq:gammahat}. Then, we get an estimate for $\beta=\hat{\Gamma}\theta$, denoted $\hat{\beta}_n$, via ridge regression.\\

From here, we can calculate $\hat{\theta}_n = \hat{\Gamma}_n^{-1} \hat{\beta}_n.$ Thus, we express the bound $\norm{\hat{\theta}_n -\theta}_2$ as such: 
\begin{align*}
    \norm{\hat{\theta}_n - \theta}_2
    &= \norm{\hat{\Gamma}_n^{-1}\hat{\beta}_n  - \hat{\Gamma}_n^{-1}\beta }_2\\
    &= \norm{\hat{\Gamma}_n^{-1} \left(\hat{\beta}_n  - \beta\right) }_2\\
    &\leq \norm{\hat{\Gamma}_n^{-1}}_2 \norm{\hat{\beta}_n  - \beta}_2\\
    &= \sigma_{\max}\left\{\hat{\Gamma}_n^{-1}\right\} \norm{\hat{\beta}_n  - \beta}_2\\
    &= \frac{1}{\sigma_{\min}\left\{\hat{\Gamma}_n\right\}} \norm{\hat{\beta}_n  - \beta}_2,\\
\end{align*}
where $\sigma_{\max}$ and $\sigma_{\min}$ are the maximum and minimum singular values of a matrix, respectively and $\hat{\Gamma}_n$ is full rank.\\

Thus, we need to find two bounds in order to upper bound $\norm{\hat{\theta}_n-\theta}_2$:
\begin{enumerate}
    \item find a lower bound for $\sigma_{\min} \{ \hat{\Gamma}\}$ (given by \cref{lemma:sigma-min-bound}); and
    \item find an upper bound for $\left|\left| \hat{\beta}_n - \beta \right|\right|_2$ (given by \cref{thm:beta-bound}).
\end{enumerate}

\begin{lemma}\label{lemma:sigma-min-bound}(Lower bound for $\sigma_{\min}(\hat{\Gamma})$ in the two arm case for two types of agents) For a bandit algorithm with two types of agents and two arms, where $p_1$ of the population is agent of type 1, $p_2$ of the population is agent of type 2, at round $t \geq \frac{12}{p_2}\log(1/\delta)$, with probability at least $1 - \delta$, 
\begin{equation}
    \sigma_{\min}(\hat{\Gamma}) \geq \frac{\sqrt{2}}{4}p_2
\end{equation}
\end{lemma}

\begin{proof}
In our algorithm, we guarantee that agents of type 2 will always follow our recommendations. On the other hand, agents of type 1 will always pick arm 1 during the sampling stage and the first racing stage. Let the actual proportion of agents showing up being type 1 and type 2 are $\hat{p}_1$ and $\hat{p}_2$, respectively. We have 
\begin{equation}
    \hat{\Gamma} = \hat{p}_1\begin{pmatrix}
       1 & 0\\
       1 & 0
    \end{pmatrix} + \hat{p}_2\begin{pmatrix}
       1 & 0\\
       0 & 1
    \end{pmatrix} = \hat{p}\begin{pmatrix}
       1 & 0\\
       1 & 0
    \end{pmatrix} + \hat{p}_2 I
\end{equation}
Hence, we have the outer product
\begin{align*}
    \hat{\Gamma} \hat{\Gamma}^\intercal  &=  
    (\hat{p}_1\begin{pmatrix}
       1 & 0\\
       1 & 0
    \end{pmatrix} + \hat{p}_2 I) (\hat{p}_1\begin{pmatrix}
       1 & 0\\
       1 & 0
    \end{pmatrix} + \hat{p}_2 I)^\intercal\\
    &= \hat{p}_1^2 \begin{pmatrix}
        1 & 1\\
        1 & 1
    \end{pmatrix} + \hat{p}_2^2 I + \hat{p}_1 \hat{p}_2 \begin{pmatrix}
        1 & 0\\
        1 & 0
    \end{pmatrix} + \hat{p}_1 \hat{p}_2 \begin{pmatrix}
        1 & 1\\
        0 & 0
    \end{pmatrix}\\
    &= \begin{pmatrix}
        \hat{p}_1^2 + 2 \hat{p}_1\hat{p}_2 + \hat{p}_2^2 & \hat{p}_1 \hat{p}_2 + \hat{p}_1^2\\
        \hat{p}_1\hat{p}_2 + \hat{p}_1^2 & \hat{p}_1^2 + \hat{p}_2^2
    \end{pmatrix}
\end{align*}
Thus, the minimum singular value of $\hat{\Gamma}$ is 
\begin{align*}
    \sigma_{\min}(\hat{\Gamma}) &= \sqrt{\lambda_{\min}(\hat{\Gamma} \hat{\Gamma}^\intercal)}\\
    &= \sqrt{\hat{p}_1^2 + \hat{p}_1 \hat{p}_2 + \hat{p}_2^2 - \hat{p}_1\sqrt{\hat{p}_1^2 + 2 \hat{p}_1\hat{p}_2 + 2 \hat{p}_2^2}}
\end{align*}
Given that $\hat{p}_1 = 1 - \hat{p_2}$, we have that 
\begin{align*}
    \sigma_{\min}(\hat{\Gamma})  &= \sqrt{(1 - \hat{p}_2)^2 + (1 - \hat{p}_2)\hat{p}_2 + \hat{p}_2^2 - (1 - \hat{p}_2) \sqrt{(1 - \hat{p}_2)^2 + 2(1 - \hat{p}_2)\hat{p}_2 + 2 \hat{p}_2^2}}\\
    &= \sqrt{\hat{p}_2^2 - (1 - \hat{p}_2)\sqrt{ (\hat{p}_2^2 + 1)} - \hat{p}_2 + 1}
\end{align*}
We have 
\begin{align*}
    - (1 - \hat{p}_2)\sqrt{\hat{p}_2^2 + 1} - \hat{p}_2 + 1 &= (\hat{p}_2 - 1)( \sqrt{\hat{p}_2^2 + 1} - 1)\\
    &= \frac{(\hat{p}_2 - 1)(\sqrt{\hat{p}_2^2 + 1} - 1)(\sqrt{\hat{p}_2^2 + 1} + 1)}{\sqrt{\hat{p}_2^2 + 1} + 1}\\
    &= \frac{(\hat{p}_2 - 1)((\hat{p}_2^2 + 1) - 1)}{1+ \sqrt{\hat{p}_2^2 + 1}}\\
    &= \frac{(\hat{p}_2 - 1)(\hat{p}_2^2)}{1+ \sqrt{\hat{p}_2^2 + 1}}\\
    &= \hat{p}_2^2\frac{\hat{p}_2 - 1}{1 + \sqrt{\hat{p}_2^2 + 1}}
\end{align*}
Thus, we have 
\begin{align*}
    \sigma_{\min}(\hat{\Gamma}) &= \sqrt{\hat{p}_2^2 - \sqrt{(\hat{p}_2 - 1)^2 (\hat{p}_2^2 + 1)} - \hat{p}_2 + 1}\\
    &= \sqrt{\hat{p}_2^2 + \hat{p}_2^2\frac{\hat{p}_2 - 1}{1 + \sqrt{\hat{p}_2^2 + 1}}}\\
    &= \sqrt{\hat{p}_2^2 \left( 1 + \frac{\hat{p}_2 - 1}{1 + \sqrt{\hat{p}_2^2 + 1}} \right)}\\
    &= \sqrt{\hat{p}_2^2 \left( \frac{1 + \sqrt{\hat{p}_2^2 + 1} + \hat{p}_2 - 1}{1 + \sqrt{\hat{p}_2^2 + 1}} \right)}\\
    &= \sqrt{\hat{p}_2^2 \left( \frac{\sqrt{\hat{p}_2^2 + 1} + \hat{p}_2}{1 + \sqrt{\hat{p}_2^2 + 1}} \right)}\\
    &\geq \sqrt{\frac{1}{2}\hat{p}_2^2} = \frac{\sqrt{2}}{2}\hat{p}_2
\end{align*}

Next, by Corollary~\ref{cor:multiplicative-chernoff}, with probability at least $1 - \delta$, the empirical proportion of type 2 agents $\hat{p}_2 \geq \frac{p_2}{2}$ at round $t \geq \frac{12}{p_2}\log(1/\delta)$. Thus, the minimum singular value 
\[\sigma_{\min}(\hat{\Gamma}) \geq \frac{\sqrt{2}}{4}p_2\]
\end{proof}

\begin{proof}
In our sampling stage algorithm, we guarantee that $p_1$ of the population will always follow our recommendations. Similarly, in the racing stage, we guarantee that $p_2$ of the population will follow our recommendations. Let the proportion of agents that follow our recommendations in both stages algorithm be $p$. At round $t$, we have
\begin{align}
    p = \frac{L_1 (\rho + 1) p_1 + (q - L_1) p_2}{t}
\end{align}
where $L_1(\rho + 1)$ is the length of the sampling stage and $q$ is the current phase in the racing stage. 
Let the actual numbers of agents that follow our recommendations in both stages be $\hat{p}$.
We have 
\begin{equation}
    \hat{\Gamma} = (1 - \hat{p})\begin{pmatrix}
       1 & 0\\
       1 & 0
    \end{pmatrix} + \hat{p}\begin{pmatrix}
       1 & 0\\
       0 & 1
    \end{pmatrix} = (1 - \hat{p})\begin{pmatrix}
       1 & 0\\
       1 & 0
    \end{pmatrix} + \hat{p} I
\end{equation}
Hence, we have the outer product
\begin{align*}
    \hat{\Gamma} \hat{\Gamma}^\intercal  &=  
    ((1 - \hat{p})\begin{pmatrix}
       1 & 0\\
       1 & 0
    \end{pmatrix} + \hat{p} I) ((1 - \hat{p})\begin{pmatrix}
       1 & 0\\
       1 & 0
    \end{pmatrix} + \hat{p} I)^\intercal\\
    &= (1 - \hat{p})^2 \begin{pmatrix}
        1 & 1\\
        1 & 1
    \end{pmatrix} + \hat{p}^2 I +(1 - \hat{p}) \hat{p} \begin{pmatrix}
        1 & 0\\
        1 & 0
    \end{pmatrix} + (1 - \hat{p})\hat{p} \begin{pmatrix}
        1 & 1\\
        0 & 0
    \end{pmatrix}\\
    &= \begin{pmatrix}
        (1 - \hat{p})^2 + 2 (1 - \hat{p})\hat{p} + \hat{p}^2 &(1 - \hat{p}) \hat{p} + \hat{p}^2\\
        (1 - \hat{p})\hat{p} + \hat{p}^2 & (1 - \hat{p})^2 + \hat{p}^2
    \end{pmatrix}
\end{align*}
Thus, the minimum singular value of $\hat{\Gamma}$ is 
\begin{align*}
    \sigma_{\min}(\hat{\Gamma}) &= \sqrt{\lambda_{\min}(\hat{\Gamma} \hat{\Gamma}^\intercal)}\\
    &= \sqrt{(1 - \hat{p})^2 + (1 - \hat{p}) \hat{p} + \hat{p}^2 - (1 - \hat{p})\sqrt{(1 - \hat{p})^2 + 2 (1 - \hat{p})\hat{p} + 2 \hat{p}^2}}\\
    &= \sqrt{\hat{p}^2 - (1 - \hat{p})\sqrt{ (\hat{p}^2 + 1)} - \hat{p} + 1}
\end{align*}
We have 
\begin{align*}
    - (1 - \hat{p})\sqrt{\hat{p}^2 + 1} - \hat{p} + 1 &= (\hat{p} - 1)( \sqrt{\hat{p}^2 + 1} - 1)\\
    &= \frac{(\hat{p} - 1)(\sqrt{\hat{p}^2 + 1} - 1)(\sqrt{\hat{p}^2 + 1} + 1)}{\sqrt{\hat{p}^2 + 1} + 1}\\
    &= \frac{(\hat{p} - 1)((\hat{p}^2 + 1) - 1)}{1+ \sqrt{\hat{p}^2 + 1}}\\
    &= \frac{(\hat{p} - 1)(\hat{p}^2)}{1+ \sqrt{\hat{p}^2 + 1}}\\
    &= \hat{p}^2\frac{\hat{p} - 1}{1 + \sqrt{\hat{p}^2 + 1}}
\end{align*}
Thus, we have 
\begin{align*}
    \sigma_{\min}(\hat{\Gamma}) &= \sqrt{\hat{p}^2 - \sqrt{(\hat{p} - 1)^2 (\hat{p}^2 + 1)} - \hat{p} + 1}\\
    &= \sqrt{\hat{p}^2 + \hat{p}^2\frac{\hat{p} - 1}{1 + \sqrt{\hat{p}^2 + 1}}}\\
    &= \sqrt{\hat{p}^2 \left( 1 + \frac{\hat{p} - 1}{1 + \sqrt{\hat{p}^2 + 1}} \right)}\\
    &= \sqrt{\hat{p}^2 \left( \frac{1 + \sqrt{\hat{p}^2 + 1} + \hat{p} - 1}{1 + \sqrt{\hat{p}^2 + 1}} \right)}\\
    &= \sqrt{\hat{p}^2 \left( \frac{\sqrt{\hat{p}^2 + 1} + \hat{p}}{1 + \sqrt{\hat{p}^2 + 1}} \right)}\\
    &\geq \sqrt{\frac{1}{2}\hat{p}^2} = \frac{\sqrt{2}}{2}\hat{p}
\end{align*}
\lscomment{Not sure if we need to show that last line (i.e. show the derivative / minimized at $\hat{p}=0$).}

Next, by Corollary~\ref{cor:multiplicative-chernoff}, the empirical proportion of agents following our recommendation $\hat{p} \geq 
\frac{p}{2}$ at round $t \geq \frac{12}{p} \log(1/\delta)$. Thus, the minimum singular value 
\begin{align}
    \sigma_{\min}(\hat{\Gamma}) &\geq \frac{\sqrt{2}}{4}p\\
&= \frac{\sqrt{2}}{4}\left(\frac{L_1 (\rho + 1) p_1 + (q-L_1) p_2}{t} \right)
\end{align}

\end{proof}

In the following, we will demonstrate an upper bound on $\norm{\hat{\beta}_n - \beta}_2$.
\begin{lemma}
\label{lemma:mahalanobis-bound} For some $\delta \in (0,1)$, with probability at least $1-\delta$,
\begin{align}
    \norm{\tilde{\beta} - \beta^*}_{\Sigma + \lambda \bI} \leq \sqrt{\lambda (m + \Upsilon^2)} + 2\sqrt{2\log\left(\frac{2}{\delta_2}\right) + (m+1)\log\left( 1 + \frac{2n}{\lambda(m+1)}\right)}
\end{align}
where $\abs{\E[g(u)]} \leq \Upsilon$.
\end{lemma}
\begin{proof}
We have:
\begin{align*}
    \tilde{\beta} - \beta^* = - (\Sigma + \lambda \bI)^{-1} \lambda \beta^* + (\Sigma + \lambda \bI)^{-1} \left(\sum_{i=1}^n \tilde{z}_i\gamma_i \right) + (\Sigma + \lambda \bI)^{-1} \left(\sum_{i=1}^n\tilde{z}_i \nu_i \right)
\end{align*}
Observe that 
\begin{align*}
    \norm{(\Sigma + \lambda \bI)^{-1} \lambda \beta^*}_{\Sigma + \lambda \bI} &= \sqrt{\lambda (\beta^*)^\intercal ((\Sigma + \lambda \bI)^{-1})^\intercal (\Sigma + \lambda \bI) (\Sigma + \lambda \bI)^{-1} \lambda \beta^*} \\
    &= \sqrt{\lambda (\beta^*)^\intercal ((\Sigma + \lambda \bI)^{-1})^\intercal \lambda \beta^*} \\
    &\leq \lambda \sqrt{\norm{\beta^*}_2^2 \norm{(\Sigma + \lambda \bI)^{-1}}}_2 \ \tag{by Theorem~\eqref{thm:cauchy-schwarz}}\\
    &= \lambda \norm{\beta^*}_2 \sqrt{\lambda_{\max}\left\{(\Sigma + \lambda \bI)^{-1}\right\}}\\
    &= \lambda \norm{\beta^*}_2 \frac{1}{\sqrt{\lambda_{\min}\left\{\Sigma +
    \lambda \bI \right\}}}\\
    &\leq \lambda \norm{\left(\beta, \E_u[g(u)] \right)}_2 \frac{1}{\sqrt{\lambda}}\\
    &= \sqrt{\lambda \left(\norm{\beta}_2^2 + \left(\E_u[g(u)]\right)^2 \right)}\\
    &\leq \sqrt{\lambda(m + \Upsilon^2)}
\end{align*}
We also have that, for some confidence $\delta_1>0$, with probability at least $1-\delta_1$
\begin{align*}
    \norm{(\Sigma + \lambda \bI)^{-1} \left(\sum_{i=1}^n \tilde{z}_i\gamma_i \right)}_{\Sigma + \lambda \bI} &= \sqrt{\left((\Sigma + \lambda \bI)^{-1} \left(\sum_{i=1}^n \tilde{z}_i\gamma_i \right)\right)^\intercal (\Sigma + \lambda \bI) (\Sigma + \lambda \bI)^{-1} \left(\sum_{i=1}^n \tilde{z}_i\gamma_i \right)}\\
    &= \sqrt{\left(\sum_{i=1}^n \tilde{z}_i\gamma_i \right)^\intercal ((\Sigma + \lambda \bI)^{-1}) ^\intercal \left(\sum_{i=1}^n \tilde{z}_i\gamma_i \right)}\\
    &= \norm{\sum_{i=1}^n \tilde{z}_i\gamma_i}_{((\Sigma + \lambda \bI)^{-1}) ^\intercal}\\
    &\leq \sqrt{2\log\left(\frac{1}{\delta_1}\right) + \log\left(\frac{\det(\Sigma + \lambda \bI)}{\lambda^{m+1}}\right)} \ \tag{by Theorem~\ref{thm:mahalanobis-norm-bound}}\\
    &\leq \sqrt{2\log\left(\frac{1}{\delta_1}\right) + (m+1)\log\left( 1 + \frac{2n}{\lambda(m+1)}\right)} \ \tag{by Lemma~\eqref{lemma:epl}}
\end{align*}

Finally, we want to bound $\norm{(\Sigma + \lambda \bI)^{-1} \left(\sum_{i=1}^n\tilde{z}_i \nu_i \right)}_{\Sigma + \lambda \bI}$. We will do so by invoking Theorem~\eqref{thm:mahalanobis-norm-bound}, as above. However, in order to show that this theorem applies, we first have to reduce the sum $\sum_{i=1}^n \tilde{z}_i \nu_i$ is mean-zero. Let $n_j = e_j^\intercal \sum_{i=1}^n z_i$ and $\tilde{e}_j = (e_j, 1)$. We have:
\begin{align*}
    \sum_{i=1}^n \tilde{z}_i \nu_i &= \sum_{i=1}^n \tilde{z}_i \theta^\intercal (\Gamma - \hat{\Gamma})^\intercal z_i\\
    &= \sum_{i=1}^n \tilde{z}_i \theta^\intercal \Gamma^\intercal z_i - \sum_{i=1}^n \tilde{z}_i \theta^\intercal \hat{\Gamma}^\intercal z_i\\
    &= \sum_{i=1}^n \tilde{z}_i \theta^\intercal \Gamma^\intercal z_i - \sum_{j=1}^m n_j \tilde{e}_j \theta^\intercal \hat{\Gamma}_j^\intercal \ \text{(where $\hat{\Gamma}_j$ is the j-th row of $\hat{\Gamma}$)}\\
    &= \sum_{i=1}^n \tilde{z}_i \theta^\intercal \Gamma^\intercal z_i - \sum_{j=1}^m n_j \tilde{e}_j \theta^\intercal \left(\frac{1}{n_j} \sum_{i=1}^n \1[z_i = e_j]x_i \right)\\
    &= \sum_{i=1}^n \tilde{z}_i \theta^\intercal \Gamma^\intercal z_i - \sum_{j=1}^m \tilde{e}_j \theta^\intercal \sum_{i=1}^n \1[z_i = e_j]x_i\\
    &= \sum_{i=1}^n \tilde{z}_i \theta^\intercal \Gamma^\intercal z_i - \sum_{i=1}^n \tilde{z}_i \theta^\intercal x_i\\
    &= \sum_{i=1}^n \tilde{z}_i ( \theta^\intercal \Gamma^\intercal z_i - \theta^\intercal x_i)
\end{align*}

This term is mean-zero. Hence, for confidence $\delta_2>0$, with probability at least $1-\delta_2$, we have:
\begin{align*}
    \norm{(\Sigma + \lambda \bI)^{-1} \left(\sum_{i=1}^n\tilde{z}_i \nu_i \right)}_{\Sigma + \lambda \bI} &= \sqrt{\left((\Sigma + \lambda \bI)^{-1} \left(\sum_{i=1}^n\tilde{z}_i \nu_i \right) \right)^\intercal (\Sigma + \lambda \bI) (\Sigma + \lambda \bI)^{-1} \left(\sum_{i=1}^n\tilde{z}_i \nu_i \right)}\\
    &= \sqrt{ \left(\sum_{i=1}^n\tilde{z}_i \nu_i \right)^\intercal \left((\Sigma + \lambda \bI)^{-1} \right)^\intercal \left(\sum_{i=1}^n\tilde{z}_i \nu_i \right)}\\
    &= \norm{\sum_{i=1}^n\tilde{z}_i \nu_i}_{\left((\Sigma + \lambda \bI)^{-1} \right)^\intercal}\\
    &\leq \sqrt{2\log\left(\frac{1}{\delta_2}\right) + \log\left(\frac{\det(\Sigma + \lambda \bI)}{\lambda^{m+1}}\right)} \ \tag{by Theorem~\eqref{thm:mahalanobis-norm-bound}}\\
    &\leq \sqrt{2\log\left(\frac{1}{\delta_2}\right) + (m+1)\log\left( 1 + \frac{2n}{\lambda(m+1)}\right)} \ \tag{by Lemma~\eqref{lemma:epl}}
\end{align*}

Combining these three bounds, we get that, for confidence $\delta>0$, with probability at least $1-\delta$,
\[ \norm{\tilde{\beta} - \beta^*}_{\Sigma + \lambda \bI} \leq \sqrt{\lambda (m + \Upsilon^2)} + 2\sqrt{2\log\left(\frac{2}{\delta}\right) + (m+1)\log\left( 1 + \frac{2n}{\lambda(m+1)}\right)} \tag{by Lemma~\eqref{thm:union}}\]
\end{proof}

\begin{lemma}
\label{lemma:min_sigma}
The minimum eigenvalue
\[ \displaystyle \lambda_{\min} \left\{\sum_{i=1}^n z_i z_i^{\intercal} \right\} = n_{\min},
\]
the minimum frequency at which any arm is recommended
from the sample set $(z,X,y)_n$.
\end{lemma} 

\begin{proof}
Consider for arbitrary fixed $i$, the vector
$z_i = \left(0, \ \cdots, \ 0, 1, 0, \ \cdots, \ 0 \right)$, where the position of the single $1$ corresponds to the arm $a_i$ recommended in the $i^{\text{th}}$ sample, e.g. if we recommend arm $1$ in the $i^{\text{th}}$ sample, then $z_i = \left( 1, 0, \ \cdots, \ 0 \right).$ 
Then, the normalized sum 
\[  \sum_{i=1}^n z_i z_i^{\intercal} =  \sum_{i=1}^n \diag(z_i) = \diag\left( \sum_{i=1}^n \ind[z_i = \e_1],\ \cdots \ ,  \sum_{i=1}^n \ind[z_i = \e_m] \right),
\]

where \[\diag(a_1, a_2, \cdots, a_n) := 
\begin{pmatrix}
    a_1 & 0 & \cdots & 0\\
    0 & a_2 & \cdots & 0\\
    \vdots & \vdots & \ddots & \vdots \\
    0 & 0 & \cdots & a_n
\end{pmatrix}.\]
For a single arm $j \in [1,m]$, the term $ \sum_{i=1}^n \ind[z_i = \e_j]$ corresponds to the frequency at which treatment $j$ is recommend out of all $n$ samples. 
Let $n_{\min}$ be the minimum number of times that any one arm is recommended such that
\[
n_{\min} := \min_j \sum_{i=1}^n \ind[z_i = \e_j].
\]

With this, we may express the smallest diagonal entry in the matrix as $n_{\min}$. 

Since $\sum_{i=1}^n z_i z_i^{\intercal}$ is a non-negative semidefinite diagonal matrix, its eigenvalues are simply the entries of the diagonal. Thus, 
\[\lambda_{\min} \left\{ \sum_{i=1}^n z_i z_i^{\intercal} \right\} = n_{\min}. \]
\end{proof} 
\begin{theorem} 
\label{thm:beta-bound}
For some $\delta \in (0,1)$, with probability at least $1-\delta$,
\begin{align*}
    \norm{\hat{\beta} - \beta}_2 \leq \frac{\sqrt{\lambda (m + \Upsilon^2)} + 2\sqrt{2\log\left(\frac{2}{\delta}\right) + (m+1)\log\left( 1 + \frac{2n}{\lambda(m+1)}\right)}}{\sqrt{n_{\min}}}
\end{align*}
where $n_{\min}$ is the minimum number of times any arm is recommended, i.e. $\displaystyle n_{\min} := \argmin_j \sum_{i=1}^n \ind[z_i = \e_j]$.
\end{theorem}
\begin{proof}

Let $\Sigma = \sum_{i=1}^n \tilde{z}_i \tilde{z}_i^\intercal$ where $\tilde{z}_i = (z_i,1)$. Let $\lambda\geq0$ be some non-negative constant. Remember that $\beta^* = (\beta, \E[g(u)])$. Using ridge regression, we estimate the relationship between $y_i$ and $\tilde{z}_i$ as:
\begin{align*}
    \tilde{\beta} &= (\Sigma + \lambda \bI)^{-1} \left(\sum_{i=1}^n \tilde{z}_i y_i \right)\\
    &= (\Sigma + \lambda \bI)^{-1} \left(\sum_{i=1}^n \tilde{z}_i (\tilde{z}_i^\intercal \beta^* + \gamma_i + \nu_i) + \lambda \beta^* - \lambda \beta^* \right) \ \tag{by Equation \ref{eq:y}}\\
    &= \beta^* - (\Sigma + \lambda \bI)^{-1} \lambda \beta^* + (\Sigma + \lambda \bI)^{-1} \left(\sum_{i=1}^n \tilde{z}_i\gamma_i \right) + (\Sigma + \lambda \bI)^{-1} \left(\sum_{i=1}^n\tilde{z}_i \nu_i\right)
\end{align*}
Let $\hat{\beta}$ be such that $\tilde{\beta} = \left( \hat{\beta}, \hat{\E}[g(u)] \right)$ where $\hat{\E}[g(u)]$ estimates $\E[g(u)]$ and $\hat{\beta}$ estimates $\beta$.\\

Now, let $\norm{x}_M \triangleq \sqrt{x^\intercal M x}$ for any real matrix $M$ and vector $x$ (see lemma~\ref{thm:mahalanobis-norm}). We have 
\begin{align*}
    \norm{\tilde{\beta} - \beta^*}^2_{\Sigma + \lambda \bI} &\geq \norm{(\hat{\beta}, 0) - (\beta, 0)}^2_{\Sigma + \lambda\bI}\\
    &= (\hat{\beta} - \beta, 0)^\intercal (\Sigma + \lambda \bI) (\hat{\beta} - \beta, 0)\\
    &= (\hat{\beta} - \beta, 0)^\intercal \Sigma (\hat{\beta} - \beta, 0) + \lambda\norm{\hat{\beta} - \beta}_2^2\\
    &= \sum_{i=1}^n (\langle(\hat{\beta} - \beta, 0), (z_i, 1))\rangle)^2 + \lambda \norm{\hat{\beta} - \beta}_2^2\\
    &= \sum_{i=1}^n (\langle\hat{\beta} - \beta, z_i\rangle)^2 + \lambda \norm{\hat{\beta} - \beta}_2^2\\
    &= (\hat{\beta} - \beta)^\intercal \left( \sum_{i=1}^n z_i z_i^\intercal \right) (\hat{\beta} - \beta) + \lambda \norm{\hat{\beta} - \beta}_2^2\\
    &\geq \lambda_{\min}\left\{\sum_{i=1}^n z_i z_i^\intercal \right\} \norm{\hat{\beta} - \beta}_2^2 + \lambda \norm{\hat{\beta} - \beta}_2^2 \tag{see proof of Lemma~\eqref{lemma:min_sigma}}\\
    &= (n_{\min} + \lambda) \norm{\hat{\beta} - \beta}_2^2, \ \tag{by Lemma~\eqref{lemma:min_sigma}}
\end{align*}
where $n_{\min}$ is the minimum number of times any arm is recommended, i.e. $\displaystyle n_{\min} := \argmin_j \sum_{i=1}^n \ind[z_i = \e_j]$.
Hence, for some $\delta \in (0,1)$, with probability at least $1 - \delta$:
\begin{align*}
    \norm{\hat{\beta} - \beta}_2 &\leq \frac{\sqrt{\lambda (m + \Upsilon^2)} + 2\sqrt{2\log\left(\frac{2}{\delta}\right) + (m+1)\log\left( 1 + \frac{2n}{\lambda(m+1)}\right)}}{\sqrt{n_{\min}}} \ \tag{by Lemma~\eqref{lemma:mahalanobis-bound}}
\end{align*}
\end{proof}

\input{theorems}
