# Supplementary material for: Incentivizing Compliance with Algorithmic Instruments
Source: arXiv:2107.10093 source file (2021-07-28)
Supplement: Supplementary file 3 [file control-treatment-appendix-nu-eps.tex]

\appendix
\section{Supplementary Material}
\subsection{IV Estimator Proof for Control-Treatment Setting}
\label{sec:iv-estimator}
% \subsubsection{Finite Sample Analysis}
Recall that our model can be stated as the following two-stage equations:
\begin{equation}
    \begin{cases}
    y_i = \theta x_i + g(u_i) + \epsilon_i\\
    x_i = f(u_i, z_i, i)
    \end{cases}
\end{equation}
\swcomment{the selection function also depends on $t$?}
\lscomment{I think so. Is your comment implying it should or shouldn't be dependent on $t$?}

\swdelete{The recommendation $z_i$ and the action choice $x_i$ to be binary, i.e, either $0$ or $1$. This correspond to our control-treatment setting where the control action correspond to $0$, and the treatment correspond to $1$. The reward $y_i$ is given by the action $x_i$, treatment effect $\theta$, zero-mean noise $\epsilon$ and the unobserved confounding shift $g(u_i)$. Our goal is to consistently estimate the treatment effect $\theta$. This is complicated by the unobserved confounding shift $g(u_i)$ and its correlation with the action choice $x_i$.\\} % Redundant text

To analyze the Wald estimator, we introduce two conditional probabilities that an agent choose the treatment given a recommendation $\gamma_0$ and $\gamma_1$, formally defined as
\begin{align*}
    \gamma_0 = \Prob[x_i = 1| z_i = 0] \qquad \text{and} \qquad
    \gamma_1 = \Prob[x_i = 1| z_i = 1]
\end{align*}
Then, we can rewrite $x_i$ as such:
\begin{align*}
    x_i &= \gamma_1 z_i + \gamma_0 (1 - z_i) + (f(u_i, z_i) - \gamma_1 z_i - \gamma_0 (1 - z_i))\\
    &= \gamma_1 z_i + \gamma_0 (1 - z_i) + \eta_i\\
    &= \gamma z_i + \gamma_0 + \eta_i
\end{align*}
where $\eta_i = f(u_i, z_i) - \gamma_1 z_i - \gamma_0 (1 - z_i)$ is a mean-zero random variable and $\gamma = \gamma_1 - \gamma_0$ is the population \textit{compliance coefficient}. Now, we can rewrite the reward $y_i$ as 
\begin{align*}
    y_i &= \theta\left(\gamma z_i + \gamma_0 + \eta_i\right) + g(u_i) + \epsilon_i\\
    &= \underbrace{\theta\,\gamma}_{\beta} z_i + \theta \gamma_0 + \theta \eta_t + g(u_i) + \epsilon_i
\end{align*}
Let the operator $\bar{\cdot}$ denote the mean, such that $\bar{y}:=\frac{1}{n}\sum_{i=1}^n y_i$ and $\bar{g}:=\frac{1}{n}\sum_{i=1}^n g(u_i)$, etc. Then,
\begin{align*}
    \bar{y} &= \beta\bar{z} + \theta\gamma_0 + \theta\bar{\eta} + \bar{g} + \bar{\epsilon}
\end{align*}
Thus, the centered reward and treatment choice at round $i$ are given as:
\begin{equation}
    \begin{cases}
    \label{eq:centered-reward-treatment-choice}
    y_i - \bar{y}_i = \beta(z_i-\bar{z}) + \theta(\eta_i-\bar{\eta}) + g(u_i)-\bar{g} + \epsilon_i-\bar{\epsilon}\\
    x_i - \bar{x}_i = \gamma(z_i-\bar{z}) + \eta_i-\bar{\eta}
    \end{cases}
\end{equation}
This formulation of the centered reward $y_i-\bar{y}$ allows us to express and bound the error between the treatment effect $\theta$ and its instrumental variable estimate $\hat{\theta}_n$, which we show in the following section.
% \subsubsection{Finite Sample Analysis}
\label{sec:approximation-bound-proof}
Given $n\in\RR$ samples $(z, x, y)_n$, we would like to bound the difference between the predicted exogenous treatment effect, denoted $\hat{\theta}_n$, and the true exogenous treatment effect $\theta$. 

\treatmentapproximationbound*

\begin{proof}
We can estimate $\hat{\theta}_n$ via a Two-Stage Least Squares (2SLS). In the first stage, we regress $y_i-\bar{y}$ onto $z_i-\bar{z}$ to get the empirical estimate $\hat{\beta}_n$ and $x_i-\bar{x}$ onto $z_i-\bar{z}$ to get $\hat{\gamma}_n$ as such:
\begin{equation}
    \hat{\beta}_n := \frac{\sum_{i=1}^n (y_i - \bar{y})(z_i - \bar{z})}{\sum_{i=1}^n (z_i -\bar{z})^2} \hspace{1cm}\text{and}\hspace{1cm} \hat{\gamma}_n := \frac{\sum_{i=1}^n (x_i - \bar{x})(z_i - \bar{z})}{\sum_{i=1}^n (z_i -\bar{z})^2}
    \label{eq:beta-gamma-hat}
\end{equation}
Second, we take their quotient as the predicted treatment effect $\hat{\theta}_n$, i.e. 
\begin{align}
    \hat{\theta}_n &= \frac{\hat{\beta}_n}{\hat{\gamma}_n}\\
    &= \frac{\sum_{i=1}^n (y_i - \bar{y})(z_i - \bar{z})}{\sum_{i=1}^n (z_i -\bar{z})^2} \frac{\sum_{i=1}^n (z_i -\bar{z})^2}{\sum_{i=1}^n (x_i - \bar{x})(z_i - \bar{z})} \nonumber\\
    &= \frac{\sum_{i=1}^n (y_i - \bar{y})(z_i - \bar{z})}{\sum_{i=1}^n (x_i - \bar{x})(z_i - \bar{z})}
\end{align}

Hence, the absolute value of the difference
\begin{align*}
    \left| \hat{\theta}_n - \theta \right|
    &= \left| \frac{\sum_{i=1}^n (y_i - \bar{y})(z_i - \bar{z})}{\sum_{i=1}^n (x_i - \bar{x})(z_i - \bar{z})} - \theta \right|\\
    &= \left| \frac{\sum_{i=1}^n \left(\theta\gamma(z_i-\bar{z}) + \theta(\eta_i-\bar{\eta}) + g(u_i)-\bar{g} + \epsilon_i-\bar{\epsilon}\right)(z_i - \bar{z})}{\sum_{i=1}^n (x_i - \bar{x})(z_i - \bar{z})} - \theta \right| \tag{by \cref{eq:centered-reward-treatment-choice}}\\
    &= \left| \theta + \frac{\sum_{i=1}^n \left(g(u_i)-\bar{g} + \epsilon_i-\bar{\epsilon}\right)(z_i - \bar{z})}{\sum_{i=1}^n (x_i - \bar{x})(z_i - \bar{z})} - \theta \right|\\
    &= \frac{\left|\sum_{i=1}^n \left(g(u_i)-\bar{g} + \epsilon_i-\bar{\epsilon}\right)(z_i - \bar{z})\right|}{\left|\sum_{i=1}^n (x_i - \bar{x})(z_i - \bar{z})\right|}\\
    &= \frac{\left|\sum_{i=1}^n \left(g(u_i)-\bar{g} + \epsilon_i-\bar{\epsilon}\right)(z_i - \bar{z})\right|}{\left|\sum_{i=1}^n (x_i - \bar{x})(z_i - \bar{z})\right|}
\end{align*}
Finally, we need to find an upper bound for the numerator $\displaystyle\left|\sum_{i=1}^n \left(g(u_i)-\bar{g} + \epsilon_i-\bar{\epsilon}\right)(z_i - \bar{z})\right|$. We do so in \cref{eq:approximation-bound-numerator}.
\end{proof}

\begin{lemma}\label{eq:approximation-bound-numerator}
For some $\delta \in (0,1)$, with probability at least $1-\delta$, we have
\begin{equation}
    \left|\sum_{i=1}^n \left(g(u_i)-\bar{g} + \epsilon_i-\bar{\epsilon}\right)(z_i - \bar{z})\right| \leq \left(2\sigma_{\eps}+4\Upsilon\right)\sqrt{2n\log(4/\delta)}
\end{equation}
\end{lemma}
\begin{proof}
    \begin{align*}
        &\left|\sum_{i=1}^n \left(g(u_i)-\bar{g} + \epsilon_i-\bar{\epsilon}\right)(z_i - \bar{z})\right|\\
        &= \left|\sum_{i=1}^n \left(g(u_i)-\E[g(u)] + \E[g(u)]-\bar{g} + \epsilon_i-\bar{\epsilon}\right)(z_i - \bar{z})\right|\\
        &= \left|\sum_{i=1}^n \left(g(u_i)-\E[g(u)] + \epsilon_i\right)z_i - \sum_{i=1}^n \left(g(u_i)-\E[g(u)] + \epsilon_i\right)\bar{z} + \sum_{i=1}^n \left(\E[g(u)]-\bar{g}-\bar{\epsilon}\right)(z_i - \bar{z})\right|\\
        &= \left|\sum_{i=1}^n \left(g(u_i)-\E[g(u)] + \epsilon_i\right)z_i - \sum_{i=1}^n \left(g(u_i)-\E[g(u)] + \epsilon_i\right)\bar{z}\right| \tag{since $\sum_{i=1}^n(z_i - \bar{z})=0$}\\
        &\leq \left|\sum_{i=1}^n \left(g(u_i)-\E[g(u)] + \epsilon_i\right)z_i\right| + \left|\sum_{i=1}^n \left(g(u_i)-\E[g(u)] + \epsilon_i\right)\right| \tag{by the triangle inequality and $|\bar{z}|\leq1$}\\
        &\leq \left|\sigma_{\eps}\sqrt{2n_1\log(1/\delta_1)} + 2\Upsilon\sqrt{\frac{n_1\log(1/\delta_2)}{2}}\right| + \left|\sigma_{\eps}\sqrt{2n\log(1/\delta_3)} + 2\Upsilon\sqrt{\frac{n\log(1/\delta_4)}{2}}\right| \tag{by Chernoff Bound, where $n_1:=\sum_{i=1}^nz_i$}\\
        &\leq \left(2\sigma_{\eps}+4\Upsilon\right)\sqrt{2n\log(4/\delta)} \tag{since $n_1\leq\,n$ and by Union Bound, where $\delta:=\delta_1+\delta_2+\delta_3+\delta_4$}\\
    \end{align*}
\end{proof}

\swcomment{we are no longer using BIC for our wording}

\begin{corollary}[Lower bound on $\left|\sum_{i=1}^n(x_i-\bar{x})(z_i-\bar{z})\right|$]\label{thm:approximation-bound-denominator}
    Fix any phase. Let $p_{BIC}$ be the proportion in the population of agents who are BIC in this phase. Then, the denominator of the approximation bound given by the samples of this phase
    \[\left|\sum_{i=1}^n(x_i-\bar{x})(z_i-\bar{z})\right| \geq \begin{cases}
        n\bar{z}(1-\bar{z}) & \text{if the proportion $p_{BIC}=1$};\\
        \bar{z}\left(np_{BIC}(1-\bar{z})-\sqrt{\frac{n(1-\bar{z})\log(1/\delta)}{2}}\right) & \text{with probability at least $1-\delta$ otherwise}.
    \end{cases}\]
\end{corollary}
\begin{proof}
Fix any phase. Recall that $\bar{z}$ is the probability of recommending arm 1 in this phase. Also let $n_0$ and $n_1$ be the number of samples with agents of type 0 and type 1, respectively. Let $n_{0,0}$ be the number of samples with agents of type 0 with recommendations of arm 0.

\begin{align*}
    \left|\sum_{i=1}^n(x_i-\bar{x})(z_i-\bar{z})\right|
    &= \left|\sum_{i=1}^n(x_i-\bar{x})z_i-\bar{z}\sum_{i=1}^n(x_i-\bar{x})\right|\\
    &= \left|\sum\limits_{i=1}^n(1-\bar{x})\1[z_i=1]-\bar{z}\sum_{i=1}^n(x_i-\bar{x})\right|\tag{since algorithms~\ref{alg:sampling-control-treatment} \& \ref{alg:racing-two-types-mixed-preferences} are BIC for type 0, $z_i=1\Rightarrow x_i=1$ ; otherwise, $z_i=0$}\\
    &= \left|\bar{z}n(1-\bar{x})-\bar{z}\sum_{i=1}^nx_i+\bar{z}\sum_{i=1}^n\bar{x}\right|\\
    &= \left|\bar{z}n-\bar{z}n\bar{x}+\bar{z}n\bar{x}-\bar{z}\sum_{i=1}^nx_i\right|\\
    &= \bar{z}\left|n-\sum_{i=1}^nx_i\right|\\
    &= \bar{z}n_{0,0}\\
\end{align*}

Now, we need to lower bound $n_{0,0}$. 
Let $p_{BIC}$ be the proportion in the population of agents who are BIC in this phase. Thus, in any round where the recommendation $z_i=0$, the probability that an agent takes the recommendation is $p_{BIC}$. Thus, the expected value 
\[\E[n_{0,0}]=np_{BIC}(1-\bar{z}).\]

Now, there are two cases:
\begin{enumerate}
    \item If the proportion $p_{BIC}=1$, i.e. in a phase when our recommendation is BIC for all agents, then $n_{0,0}=\E[n_{0,0}]=n(1-\bar{z})$. In this case, the denominator \[\left|\sum_{i=1}^n(x_i-\bar{x})(z_i-\bar{z})\right|=n\bar{z}(1-\bar{z})\]
    \item Otherwise, we may take a high probability bound on the number of agents $n_{0,0}$ that take our recommendation of arm 0. With probability at least $1-\delta$,
    \[n_{0,0} \geq np_{BIC}(1-\bar{z})-\sqrt{\frac{n(1-\bar{z})\log(1/\delta)}{2}}.\]

    Therefore, with probability at least $1-\delta$,
    \[\left|\sum_{i=1}^n(x_i-\bar{x})(z_i-\bar{z})\right|\geq \bar{z}\left(np_{BIC}(1-\bar{z})-\sqrt{\frac{n(1-\bar{z})\log(1/\delta)}{2}}\right)\].
\end{enumerate}
\end{proof}

%%%%%%%%%%%%%%%%%%%%%%%%%%%%%%%%%%%%%%%%%%%%%
%%%%%%%%%%%%%%%%%%%%%%%%%%%%%%%%%%%%%%%%%%%%%

\subsection{Sampling Stage Proofs}
\subsubsection{Sampling Stage Type 0 Compliant Proof}\label{sec:sampling-bic-proof}
\bicsamplingcontroltreatment*
\begin{proof} Recall that for type 0, the \textit{fighting chance} event:
\begin{equation}
    \xi_0 = \left\{ \frac{1}{\ell_1} \sum_{t=1}^{\ell_1} y_t^1 - \frac{1}{\ell_0} \sum_{t=1}^{\ell_0} y_t^0 > 2\Upsilon + \sigma_\epsilon \sqrt{\frac{2\log(1/\delta)}{\ell_0}} + \sigma_\epsilon \sqrt{\frac{2\log(1/\delta)}{\ell_1}} + \frac{1}{2} + \nu   \right\} 
\end{equation}
happens with probability at least $1-\delta$ for confidence $\delta > 0$.

Let $\displaystyle G := \E_{\cP_0}[\theta|S_{1, \ell_0}, S_{2, \ell_1}]$. It is sufficient to show that $\displaystyle \E_{\cP_0}[G|z_t = 0]\Prob_{\cP_0}[z_t = 0] \geq 0$ (by \cref{claim:bic-equiv}).
\begin{claim}
\label{claim:bic-equiv}
Assume that we have $\displaystyle \E_{\cP_0}[\theta|z_t = 1]\Prob_{\cP_0}[z_t = 1] \geq 0$. Then we also have 
\newline$\displaystyle \E_{\cP_0}[\theta|z_t = 0]\Prob_{\cP_0}[z_t = 0] < 0$.
\end{claim}
\begin{proof}
Algorithm~\ref{alg:sampling-control-treatment} is designed in a way such that we always recommend arm 1 with some positive possibility, i.e. $\Prob_{\cP_0}[z_t = 1] > 0$.\\
Similarly, assume that we also recommend arm 0 with some positive probability: $\Prob_{\cP_0}[z_t = 0] > 0$. Assume that the expected difference in mean rewards $\displaystyle \E_{\cP_0}[\theta]\leq 0$. Then, we have:
\begin{align*}
    0 &\geq \E_{\cP_0}[\theta] \\
    &= \E_{\cP_0}[\theta|z_t = 0]\Prob_{\cP_0}[z_t = 0] + \E_{\cP_0}[\theta|z_t = 1]\Prob_{\cP_0}[z_t = 1]
\end{align*}
Since, by assumption, the product $\displaystyle \E_{\cP_0}[\theta|z_t = 1]\Prob[z_t=1] \geq 0$, it must be that the product 
\[\E_{\cP_0}[\theta|z_t = 0]\Prob_{\cP_0}[z_t = 0] \leq 0.\] 
Hence, when given an recommendation for arm 0, the agent of type $0$ will take our recommendation.
\end{proof}
Note that we have 
\begin{align*}
&\quad	\E_{\cP_0}[G | z_t = 1] \Prob_{\cP_0}[z_t = 1] \\
	&= \E_{\cP_0}[G |z_t = 1 \ \& \ p_t \in P-Q]\Prob_{\cP_0}[z_t = 1 \ \& \ p_t \in P-Q] \\
	& \hspace{.4cm} + \E_{\cP_0}[G|z_t = 1 \ \& \ p_t \in Q]\Prob_{\cP_0}[z_t = 1 \ \& \ p_t \in Q]\\
	&= \E_{\cP_0}[G | \xi_0]\Prob_{\cP_0}[\xi_0]\left(1 - \frac{1}{\rho} \right) + \E_{\cP_0}[G|z_t = 1 \ \& \ p_t \in Q]\Prob_{\cP_0}[z_t = 1 \ \& \ p_t \in Q]\\
	&= \E_{\cP_0}[G | \xi_0]\Prob_{\cP_0}[\xi_0]\left(1 - \frac{1}{\rho} \right) + \E_{\cP_0}[G|p_t\in Q]\Prob_{\cP_0}[p_t \in Q], \ \ \text{(by definition $p_t\in Q \Rightarrow z_t=0$)}\\
	&= \E_{\cP_0}[G | \xi_0]\Prob_{\cP_0}[\xi_0]\left(1 - \frac{1}{\rho} \right) + \E_{\cP_0}[\theta | p_t\in Q]\Prob_{\cP_0}[p_t \in Q] \ \ \text{(by Law of Total Expectation)}\\
	&= \E_{\cP_0}[G | \xi_0]\Prob_{\cP_0}[\xi_0]\left(1 - \frac{1}{\rho} \right) + \E_{\cP_0}[\theta]\Prob_{\cP_0}[p_t \in Q] \\
	&= \E_{\cP_0}[G | \xi_0]\Prob_{\cP_0}[\xi_0]\left(1 - \frac{1}{\rho} \right) + (\mu_0^1 - \mu_0^0)\Prob_{\cP_0}[p_t \in Q]\\
	&= \E_{\cP_0}[G | \xi_0]\Prob_{\cP_0}[\xi_0]\left(1 - \frac{1}{\rho} \right) + \frac{1}{\rho}(\mu_0^1 - \mu_0^0)
\end{align*}
For agents of type $i$ to follow our recommendation for arm 2, we need to pick $\rho$:
\begin{align}
    \E_{\cP_0}[G | z_t = 1] \Prob_{\cP_0}[z_t = 1] &\geq \phi(u_t) \nonumber\\
	\E_{\cP_0}[G | \xi_0]\Prob_{\cP_0}[\xi_0]\left(1 - \frac{1}{\rho} \right) + \frac{1}{\rho}(\mu_0^1 - \mu_0^0) &\geq \phi(u_t)\Prob_{\cP_0}[\xi_0] \nonumber\\
	\E_{\cP_0}[G | \xi_0]\Prob_{\cP_0}[\xi_0] - \frac{1}{\rho}\E_{\cP_0}[G|\xi_0] \Prob_{\cP_0}[\xi_0] + \frac{1}{\rho}(\mu_0^1 - \mu_0^0) &\geq \phi(u_t)\Prob_{\cP_0}[\xi_0] \nonumber\\
	\rho\E_{\cP_0}[G|\xi_0]\Prob_{\cP_0}[\xi_0] - \rho \phi(u_t)\Prob_{\cP_0}[\xi_0] &\geq \E_{\cP_0}[G | \xi_0]\Prob_{\cP_0}[\xi_0] - (\mu_0^1 - \mu_0^0) \nonumber\\
	\rho &\geq 1 + \frac{\mu_0^0 - \mu_0^1 + \phi(u_t)\Prob_{\cP_0}[\xi_0]}{\E_{\cP_0}[G | \xi_0]\Prob_{\cP_0}[\xi_0] - \phi(u_t)\Prob_{\cP_0}[\xi_0]} \nonumber\\
	\rho &\geq 1 + \frac{\mu_0^0 - \mu_0^1 + \nu\Prob_{\cP_0}[\xi_0]}{\E_{\cP_0}[G | \xi_0]\Prob_{\cP_0}[\xi_0] - \nu\Prob_{\cP_0}[\xi_0]} \nonumber
	\label{eq:L-condition}
\end{align}

This comes down to finding a lower bound on the denominator of the expression above. First, we define clean events $C_1$ and $C_2$ where the average errors $\frac{1}{\ell_0}\sum_{i=1}^{\ell_0} \epsilon_i$ and $\frac{1}{\ell_1}\sum_{i=1}^{\ell_1} \epsilon_i$ are bounded (following Corollary \ref{thm:high-prob-unbounded-chernoff}):
\begin{align}
     C_1 := \left \{ \bigg\vert\frac{1}{\ell_0} \sum_{i=1}^{\ell_0} \epsilon_i \bigg\vert \leq \sigma_\epsilon \sqrt{\frac{2\log(1/\delta)}{\ell_0}} \right \}.\\
      C_2 := \left \{ \bigg\vert\frac{1}{\ell_1} \sum_{i=1}^{\ell_1} \epsilon_i \bigg\vert \leq \sigma_\epsilon \sqrt{\frac{2\log(1/\delta)}{\ell_1}} \right \}.
\end{align}
Define another clean event $C'$ where both $C_1$ and $C_2$ happens simultaneously. The event $C'$ occurs with probability at least $1 - \delta$ for $\displaystyle \delta < \delta' := \frac{\Prob_{\cP_0}[\xi_0]}{8}$.

We have 
\begin{align}
    \E_{\cP_0}[G | \xi_0] \Prob_{\cP_0}[\xi_0] &= \E_{\cP_0}[G | \xi_0, C'] \Prob_{\cP_0}[\xi_0, C'] + \E_{\cP_0}[G | \xi_0, \neg C'] \Prob_{\cP_0}[\xi_0, \neg C'] \nonumber\\
    &\geq \E_{\cP_0}[G | \xi_0, C'] \Prob_{\cP_0}[\xi_0, C'] - \delta \tag{since $G \geq -1$ and $\Prob_{\cP_0}[\neg C']<\delta$} \nonumber\\
    &= \E_{\cP_0}[G | \xi_0, C'] (\Prob_{\cP_0}[\xi_0] - \Prob_{\cP_0}[\xi_0, \neg C']) - \delta \nonumber\\
    &\geq \E_{\cP_0}[G | \xi_0, C'] (\Prob_{\cP_0}[\xi_0] - \Prob_{\cP_0}[\neg C']) - \delta \nonumber\\
    &\geq \E_{\cP_0}[G | \xi_0, C'] (\Prob_{\cP_0}[\xi_0] - \delta) - \delta \nonumber\\
    &= \E_{\cP_0}[G | \xi_0, C'] \Prob_{\cP_0}[\xi_0] - \delta(1 + \E_{\cP_0}[G | \xi_0, C']) \nonumber\\
    &\geq \E_{\cP_0}[G | \xi_0, C'] \Prob_{\cP_0}[\xi_0] - 2\delta \label{eq:sampling-two-arm-clean-event}
\end{align}

This comes down to finding a lower bound on the denominator of the expression above. We can reduce the dependency of the denominator to a single prior-dependent constant $\Prob_{\cP_0}[\xi_0]$ if we lower bound the prior-dependent expected value $\E_{\cP_0}[G | \xi_0]$. That way, assuming we know the prior and can calculate the probability of event $\xi_0$, we can pick an appropriate $\rho$ to satisfy the BIC condition for all agents of type $i$. Remember that event $\xi_0 = \{ \bar{y}^1_{\ell_0} + C < \bar{y}^2_{\ell_1}\}$ where $C = 2\Upsilon + \sigma_{\epsilon}\sqrt{\frac{2\log(1/\delta)}{\ell_0}} + \sigma_{\epsilon}\sqrt{\frac{2\log(1/\delta)}{\ell_0}} +\frac{1}{2} + \nu$ and $\displaystyle G := \E_{\cP_0}[\theta|S_{1, \ell_0}, S_{2, \ell_1}]$. Then, the expected value
\begin{align}
    &\quad \E_{\cP_0}[G | \xi_0, C'] \nonumber\\ 
    &= \E_{\cP_0}[\E_{\cP_0}[\theta|S_{1, \ell_0}, S_{2, \ell_1}] | \xi_0, C'] \nonumber\\
    &= \E_{\cP_0}\left[\theta \middle| 2\Upsilon + \sigma_{\epsilon}\sqrt{\frac{2\log(1/\delta)}{\ell_0}} + \sigma_{\epsilon}\sqrt{\frac{2\log(1/\delta)}{\ell_0}} +\frac{1}{2} + \nu + \bar{y}^0_{\ell_0}< \bar{y}^1_{\ell_1}, C'\right] \nonumber\\
    &= \E_{\cP_0}\left[\theta \middle| 2\Upsilon + \sigma_{\epsilon}\sqrt{\frac{2\log(1/\delta)}{\ell_0}} + \sigma_{\epsilon}\sqrt{\frac{2\log(1/\delta)}{\ell_0}} +\frac{1}{2} + \nu + \frac{1}{\ell_0} \sum_{t=1}^{\ell_0} y^0_t< \frac{1}{\ell_1} \sum_{t=1}^{\ell_1} y^1_t, C'\right] \nonumber\\
    &= \E_{\cP_0}\left[\theta \middle|2\Upsilon + \sigma_{\epsilon}\sqrt{\frac{2\log(1/\delta)}{\ell_0}} + \sigma_{\epsilon}\sqrt{\frac{2\log(1/\delta)}{\ell_0}} +\frac{1}{2} + \nu + \right. \nonumber\\
    &\left. \hspace{4cm} \frac{1}{\ell_0} \sum_{t=1}^{\ell_0} g(u_t) + \epsilon_t< \theta + \frac{1}{\ell_1} \sum_{t=1}^{\ell_1} g(u_t) + \epsilon_t, C'\right] \nonumber\\
    &> \E_{\cP_0}\left[\theta \middle|2\Upsilon + \sigma_{\epsilon}\sqrt{\frac{2\log(1/\delta)}{\ell_0}} + \sigma_{\epsilon}\sqrt{\frac{2\log(1/\delta)}{\ell_1}} + \frac{1}{2} + \nu - \right.\\
    &\left. \hspace{4cm} \Upsilon - \sigma_{\epsilon}\sqrt{\frac{2\log(1/\delta)}{\ell_0}} < \theta + \Upsilon + \sigma_{\epsilon}\sqrt{\frac{2\log(1/\delta)}{\ell_1}} \right] \tag{since $g(u_t) > -\Upsilon$ and $\frac{1}{\ell_1}\sum_{t=1}^{\ell_1}\epsilon_t > -\sigma_\epsilon \sqrt{\frac{2\log(1/\delta)}{\ell_1}}$ by event $C'$} \nonumber\\
    &> \E_{\cP_0}\left[\theta \middle|\frac{1}{2} + \nu < \theta\right] \nonumber\\
    &> \frac{1}{2} + \nu \label{eq:sampling-stage-two-arm-gap}
\end{align}
Hence, the lower bound on the denominator is
\begin{align}
    \E_{\cP_0}[G | \xi_0] \Prob_{\cP_0}[\xi_0] - \nu\Prob_{\cP_0}[\xi_0] &\geq \E_{\cP_0}[G | \xi_0, C']\Prob_{\cP_0}[\xi_0] - 2\delta - \nu\Prob_{\cP_0}[\xi_0] \tag{by Equation \ref{eq:sampling-two-arm-clean-event}}\\
    &> \frac{1}{2}\Prob_{\cP_0}[\xi_0] + \nu\Prob_{\cP_0}[\xi_0] - 2\delta - \nu\Prob_{\cP_0}[\xi_0] \tag{by Equation \ref{eq:sampling-stage-two-arm-gap}}\\
    &= \frac{1}{4}\Prob_{\cP_0}[\xi_0] + \frac{1}{4}\Prob_{\cP_0}[\xi_0] - 2\delta \\ 
    &= 2\delta' + \frac{\Prob_{\cP_0}[\xi_0]}{4} - 2\delta \tag{since $\delta' = \frac{1}{8} \Prob_{\cP_0}[\xi_0]$}\\
    &\geq \frac{\Prob_{\cP_0}[\xi_0]}{4} \tag{since $\delta < \delta'$}
\end{align}
Hence, we can pick :
\begin{align*}
    \rho &\geq 1 + \frac{4(\mu_0^0 - \mu_0^1 + \nu\Prob_{\cP_0}[\xi_0])}{\Prob_{\cP_0}[\xi_0]}
\end{align*}
to satisfy the BIC condition for all agents of type $0$.
\end{proof}

%%%%%%%%%%%%%%%%%%%%%%%%%%%%%%%%%%%%%%%%%%%%%%%%%%

\subsubsection{Sampling Stage Treatment Effect Confidence Interval}
\lscomment{Fix this proof so the Union Bound is made more explicit and maybe change the phrase ``Estimation Bound.''}
\label{sec:sampling-estimation-bound}
\samplingestimationbound*
\begin{proof}
    Recall that the mean recommendation $\bar{z}=1/\rho$ in the sampling stage; the proportion of agents who are type 0 is $p_0$. We assume \cref{alg:sampling-control-treatment} to be initialized with parameters (see \cref{lemma:bic-sampling-control-treatment} for details) such that its recommendations are BIC for agents of type 0. Therefore, we may apply \cref{thm:approximation-bound-denominator} where we let the proportion $p_{BIC}=p_0$. Finally, we combine the high probability bound on the denominator with the high probability bound on the numerator (given by \cref{thm:treatment-approximation-bound}), taking a union bound to achieve the confidence parameters $\delta$.
\end{proof}

%%%%%%%%%%%%%%%%%%%%%%%%%%%%%%%%%%%%%%%%%%%%%%%%%%%%%%%%%%%%%%%%%%%%%%%%%%%%%%%%%%%%%%%%%%%%%%%%%%%%%%%%%%%%%%%%%%%%%%%%%%%%%%%%%%%%%%%%%%%%%%%%%%%%%%

\subsection{Racing Stage}
\subsubsection{Racing Stage Type 0 Compliant proof}
\label{sec:bic-racing-type-0}
\bicracingcontroltreatmentzero*
\begin{proof} 
Let the decision threshold $s_q$ for a phase $q$ be defined as in \cref{alg:racing-two-types-mixed-preferences}. Assume that after the elimination, at every iteration a sample of the eliminated arm is also drawn, but not revealed to the agent.\\
We define the event $\cC_1$ as the accuracy guarantee of $\hat{\theta}$ such that:
\begin{equation}
\label{eq:event-C-1}
    \cC_1 := \left\{ \forall q \geq L: |\theta - \hat{\theta}_q| < s_q \right\}
\end{equation}
where $L$ is the number of samples after running the sampling stage.\\
Let $X^a_q$ be the number of arm $a\in\{0,1\}$ samples in phase $q$. The decision threshold $s_q$ in phase $q$ is unbounded if $X^a_q=0$ for either arm $a$. We also define event $\cC_2$ where there is at least one sample of each arm in each phase:
\begin{equation}
\label{eq:event-C-2}
    \cC_2 := \left\{\forall q\geq L,a: X^a_q \geq 1 \right\}
\end{equation}
Recall that $p_0$ of the population is of type $0$. Then, if \cref{alg:racing-two-types-mixed-preferences} is BIC for all agents of type 0 and we recommend each arm at least $h$ times in phase $q$, we have $X^0_q>h$ and $X^0_q \sim B(h,p_0)$. Hence, we have
\begin{equation}
    \Prob[X^0_q \geq 1] = 1 - p_0^h = \delta'.
\end{equation}

Let $\tau\in(0,1)$. Fix phase $q\geq L$, and some agent $t$ in this phase. In order to prove that \cref{alg:racing-two-types-mixed-preferences} is BIC for all agents of type 0, we want to show that 
\begin{equation}
    \label{eq:racing-bic-type0}
    \E_{\cP_0}[\theta\vert z_t=1]\Prob_{\cP_0}[z_t=1] \geq \phi(u_t).
\end{equation}

Note that, by assumption, the parameter
\begin{align*}
    h &\geq \frac{\log\left(\frac{3\tau\Prob_{\cP_0}[\theta\geq\tau]+4}{4\tau\Prob_{\cP_0}[\theta\geq\tau]+4}\right)}{\log(1-p_2)}\\
    \Rightarrow \left(\frac{1}{2}
    \right)^h 
    &\geq \frac{3\tau\Prob_{\cP_0}[\theta\geq\tau]+4}{4\tau\Prob_{\cP_0}[\theta\geq\tau]+4}\\
    \Rightarrow \delta' = 1 - \left(\frac{1}{2}\right)^h 
    &\leq \frac{\tau\Prob_{\cP_0}[\theta\geq\tau]}{4\tau\Prob_{\cP_0}[\theta\geq\tau]+4}.
\end{align*}

From \cref{thm:treatment-approximation-bound}, with probability $\delta>0$ we have that
\begin{equation*}
    \Prob[\neg \cC_1 \vert G] \leq \delta
\end{equation*} 
Define event $\cC$ such that both events $\cC_1$ and $\cC_2$ hold simultaneously in a round: 
\begin{equation}
\label{eq:event-C}
    \cC := \left\{ \forall q \geq L_1: \cC_1 \  \& \ \cC_2 \right\}
\end{equation}

Using union bound, we have
\begin{align}
    \Prob[\neg \cC \vert G] &\leq \Prob[\neg \cC_1 \vert G] + \Prob[\neg \cC_2 \vert G]\\
    &\leq \delta + \delta' \nonumber\\
    &\leq \delta_{\tau} + \delta' \nonumber \\
    &\leq \frac{\tau\Prob_{\cP_0}[\theta\geq\tau]}{4\tau\Prob_{\cP_0}[\theta\geq\tau]+4} + \frac{\tau\Prob_{\cP_0}[\theta\geq\tau]}{4\tau\Prob_{\cP_0}[\theta\geq\tau]+4} \nonumber \\
    &= \frac{\tau\Prob_{\cP_0}[\theta\geq\tau]}{2\tau\Prob_{\cP_0}[\theta\geq\tau]+2} \label{eq:delta'}
\end{align}
Therefore, since $\theta\geq -1$, we have: 
\begin{align*}
\label{eq:racing-bic}
    \E_{\cP_0}[\theta|z_t=1]\Prob_{\cP_0}[z_t=1] &= \E_{\cP_0}[\theta|z_t=1, \cC]\Prob_{\cP_0}[z_t=1, \cC] + \E_{\cP_0}[\theta|z_t=1, \neg C]\Prob_{\cP_0}[z_t=1, \neg C]\\
    &\geq \E_{\cP_0}[\theta|z_t=1, \cC]\Prob_{\cP_0}[z_t=1, \cC] - \frac{\tau\Prob_{\cP_0}[\theta\geq\tau]}{2\tau\Prob_{\cP_0}[\theta\geq\tau]+2} 
\end{align*}
We want to upper bound the first term. This can be done by splitting it into four cases based on the value of $\theta$. We have:

\begin{equation} 
    \begin{split}
    \E_{\cP_0}[\theta|z_t=1,\cC]\Prob_{\cP_0}[z_t=1, \cC] = 
    &\E_{\cP_0}[\theta|z_t=1, \cC, \theta\geq \tau]\Prob_{\cP_0}[z_t=1, \cC, \theta\geq \tau] \\
    &\ + \E_{\cP_0}[\theta|z_t=1, \cC, 0 \leq \theta < \tau]\Prob_{\cP_0}[z_t=1, \cC, 0 \leq \theta < \tau] \\
    &\ + \E_{\cP_0}[\theta|z_t=1, \cC, -2s_q < \theta < 0]\Prob_{\cP_0}[z_t=1, \cC, -2s_q < \theta < 0] \\
    &\ + \E_{\cP_0}[\theta|z_t=1, \cC, \theta \leq -2s_q]\Prob_{\cP_0}[z_t=1, \cC, \theta\leq -2s_q] \label{eq:racing-bic-cases}
    \end{split}
\end{equation}

By definition of $s_q$, we have:
\begin{align*}
    2s_q &\leq 2s_{L}\\
    &\leq \frac{\tau\Prob_{\cP_0}[\theta\geq\tau]}{2}-\nu\\
    &\leq \tau
\end{align*}

% \lscomment{End: Need to edit this part to prove that $s_q\leq s_L$ for all $q>L$}

Conditional on $\cC$, the empirical estimate $\hat{\theta}_q > \theta - s_q \geq 2s_q$. Hence, when we have $\theta \geq \tau \geq 2s_q$, then $\hat{\theta}\geq s_q$ and arm 0 must have already been eliminated at phase $q \geq L_1$. This implies that the probability $\Prob_{\cP_0}[z_t=1, \cC, \theta\geq \tau] = \Prob_{\cP_0}[\cC, \theta\geq \tau]$. Similarly, when we have $\theta \leq -2s_q$, then $\hat{\theta} \leq -s_q$ and arm 1 must have already been eliminated at phase $q \geq L_1$. Hence, arm 1 could not be recommended in that case and the probability $\Prob_{\cP_0}[z_t=1, \cC, \theta\leq-2s_q] = 0$.\\
We can then rewrite equation~\eqref{eq:racing-bic-cases} as
\begin{align*} 
    \E_{\cP_0}[\theta|z_t=1, \cC]\Prob_{\cP_0}[z_t=1 ,\cC] \geq &\E_{\cP_0}[\theta|z_t=1, \cC, \theta \geq \tau]\Prob_{\cP_0}[z_t=1, \cC, \theta \geq \tau]\\
    &+ \E_{\cP_0}[\theta|z_t=1, \cC, 0 \leq \theta < \tau]\Prob_{\cP_0}[z_t=1, \cC, 0 \leq \theta < \tau]\\
    &+ \E_{\cP_0}[\theta|z_t=1, \cC, -2s_q < \theta < 0]\Prob_{\cP_0}[z_t=1, \cC, -2s_q < \theta < 0]\\
    \geq &\tau \Prob_{\cP_0}[\cC, \theta \geq \tau] + 0\cdot \Prob_{\cP_0}[z_t=1, \cC, 0 \leq \theta < \tau] -2s_q \Prob_{\cP_0}[z_t=1, \cC, -2s_q<\theta<0]\\
    \geq &\tau \Prob_{\cP_0}[\cC, \theta \geq \tau] - 2s_q\\
    \geq &\tau \Prob_{\cP_0}[\cC, \theta \geq \tau] - \frac{\tau\Prob_{\cP_0}[\theta\geq\tau]}{2}+\nu\\
    \geq &\tau \Prob_{\cP_0}[\cC | \theta \geq \tau] \Prob_{\cP_0}[\theta \geq \tau] - \frac{\tau\Prob_{\cP_0}[\theta\geq\tau]}{2}+\nu\\
    \geq &\tau (1 - (\delta + \delta')) \Prob_{\cP_0}[\theta \geq \tau] - \frac{\tau\Prob_{\cP_0}[\theta\geq\tau]}{2}+\nu\\
    = & \left(\frac{1}{2} - (\delta + \delta') \right) \tau \Prob_{\cP_0}[\theta \geq \tau]+\nu\\
    \geq & \left(\frac{1}{2} - \frac{\frac{1}{2} \tau \Prob_{\cP_0}[\theta \geq \tau]}{\tau \Prob_{\cP_0}[\theta \geq \tau] + 1} \right) \tau \Prob_{\cP_0}[\theta \geq \tau]+\nu \tag{by Equation~\ref{eq:delta'}}\\
    = & \frac{1}{2} \left(\frac{\tau \Prob_{\cP_0}[\theta \geq \tau] + 1 - \tau \Prob_{\cP_0}[\theta\geq \tau]}{\tau \Prob_{\cP_0}[\theta \geq \tau] + 1} \right)\tau \Prob_{\cP_0}[\theta \geq \tau]+\nu\\
    = & \frac{1}{2} \left(\frac{\tau \Prob_{\cP_0}[\theta \geq \tau]}{\tau \Prob_{\cP_0}[\theta \geq \tau] + 1} \right)+\nu
\end{align*}
Hence, we have 
\begin{align*}
    \E_{\cP_0}[\theta|z_t=1]\Prob_{\cP_0}[z_t=1] &\geq \E[\theta|z_t=1, \cC]\Prob_{\cP_0}[z_t=1, \cC] - \frac{\tau\Prob_{\cP_0}[\theta\geq\tau]}{2\tau\Prob_{\cP_0}[\theta\geq\tau]+2} \\
    &\geq \frac{\tau\Prob_{\cP_0}[\theta\geq\tau]}{2\tau\Prob_{\cP_0}[\theta\geq\tau]+2}+\nu  -  \frac{\tau\Prob_{\cP_0}[\theta\geq\tau]}{2\tau\Prob_{\cP_0}[\theta\geq\tau]+2} \\
    &= \nu \geq \phi(u_t)
\end{align*}
Therefore, Algorithm~\ref{alg:racing-two-types-mixed-preferences} fulfills equation~\ref{eq:racing-bic-type0} and is BIC for all agents of type 0.
\end{proof}

\subsubsection{Racing Stage First Part Estimation Bound}
\lscomment{Fix this proof so the Union Bound is made more explicit and maybe change the phrase ``Estimation Bound.''}
\label{sec:racing-estimation-bound-first}
\racingestimationboundfirst*
\begin{proof}
    We assume \cref{alg:racing-two-types-mixed-preferences} to be initialized with parameters (see \cref{lemma:bic-racing-control-treatment-0} for details) such that its recommendations are BIC for agents of type 0. Therefore, we may apply \cref{thm:approximation-bound-denominator} where we let the proportion $p_{BIC}=p_0$. Finally, we combine the high probability bound on the denominator with the high probability bound on the numerator (given by \cref{thm:treatment-approximation-bound}), taking a union bound to achieve the confidence parameters $\delta$.
\end{proof}

%%%%%%%%%%%%%%%%%%%%%%%%%%%%%%%%%%%%%%%%%%%%
%%%%%%%%%%%%%%%%%%%%%%%%%%%%%%%%%%%%%%%%%%%%

\subsubsection{Racing Stage Type 1 Compliant Proof}
\label{sec:bic-racing-type-1}
\bicracingcontroltreatmentone*
\begin{proof} 
Let $L_1$ be the biggest phase length of the first racing stage. Let the decision threshold $s_q$ for a phase $q$ be defined as in \cref{alg:racing-two-types-mixed-preferences}. Assume that after the elimination, at every iteration a sample of the eliminated arm is also drawn, but not revealed to the agent.\\
We define the event $\cC_1$ as the accuracy guarantee of $\hat{\theta}$ such that:
\begin{equation}
\label{eq:event-C-1}
    \cC_1 := \left\{ \forall q \geq L_1: |\theta - \hat{\theta}_q| < s_q \right\}
\end{equation}
where $L$ is the number of samples after running the sampling stage.\\
Let $X^a_q$ be the number of arm $a\in\{0,1\}$ samples in phase $q$. The decision threshold $s_q$ in phase $q$ is unbounded if $X^a_q=0$ for either arm $a$. We also define event $\cC_2$ where there is at least one sample of each arm in each phase:
\begin{equation}
\label{eq:event-C-2}
    \cC_2 := \left\{\forall q\geq L,a: X^a_q \geq 1 \right\}
\end{equation}
Recall that $p_0$ of the population is of type $0$. Then, if \cref{alg:racing-two-types-mixed-preferences} is BIC for all agents of type 0 and we recommend each arm at least $h$ times in phase $q$, we have $X^0_q>h$ and $X^0_q \sim B(h,p_0)$. Hence, we have
\begin{equation}
    \Prob[X^0_q \geq 1] = 1 - p_0^h = \delta'.
\end{equation}

Let $\tau\in(0,1)$. Fix phase $q\geq L_1$, and some agent $t$ in this phase. In order to prove that \cref{alg:racing-two-types-mixed-preferences} is BIC for all agents of type 1, we want to show that 
\begin{equation}
    \label{eq:racing-bic-type1}
    \E_{\cP_1}[\theta\vert z_t=0]\Prob_{\cP_1}[z_t=0] < \phi(u_t).
\end{equation}

Note that, by assumption, the parameter
\begin{align*}
    h &\geq \frac{\log\left(\frac{3\tau\Prob_{\cP_1}[\theta< -\tau]+4}{4\tau\Prob_{\cP_0}[\theta<-\tau]+4}\right)}{\log(1-p_2)}\\
    \Rightarrow \left(\frac{1}{2}
    \right)^h 
    &\geq \frac{3\tau\Prob_{\cP_1}[\theta<-\tau]+4}{4\tau\Prob_{\cP_1}[\theta<-\tau]+4}\\
    \Rightarrow \delta' = 1 - \left(\frac{1}{2}\right)^h 
    &\leq \frac{\tau\Prob_{\cP_1}[\theta<-\tau]}{4\tau\Prob_{\cP_1}[\theta<-\tau]+4}.
\end{align*}

From \cref{thm:treatment-approximation-bound}, with probability $\delta>0$ we have that
\begin{equation*}
    \Prob[\neg \cC_1 \vert G] \leq \delta
\end{equation*} 
Define event $\cC$ such that both events $\cC_1$ and $\cC_2$ hold simultaneously in a round: 
\begin{equation}
\label{eq:event-C}
    \cC := \left\{ \forall q \geq L_1: \cC_1 \  \& \ \cC_2 \right\}
\end{equation}

Using union bound, we have
\begin{align}
    \Prob[\neg \cC \vert G] &\leq \Prob[\neg \cC_1 \vert G] + \Prob[\neg \cC_2 \vert G]\\
    &\leq \delta + \delta' \nonumber\\
    &\leq \delta_{\tau} + \delta' \nonumber \\
    &\leq \frac{\tau\Prob_{\cP_1}[\theta<-\tau]}{4\tau\Prob_{\cP_1}[\theta<-\tau]+4} + \frac{\tau\Prob_{\cP_1}[\theta<-\tau]}{4\tau\Prob_{\cP_1}[\theta<-\tau]+4} \nonumber \\
    &= \frac{\tau\Prob_{\cP_1}[\theta<-\tau]}{2\tau\Prob_{\cP_1}[\theta<-\tau]+2} \label{eq:delta'-type1}
\end{align}
Therefore, since $\theta\leq 1$, we have: 
\begin{align*}
\label{eq:racing-bic}
    \E_{\cP_1}[\theta|z_t=0]\Prob_{\cP_1}[z_t=0] &= \E_{\cP_1}[\theta|z_t=0, \cC]\Prob_{\cP_1}[z_t=0, \cC] + \E_{\cP_1}[\theta|z_t=0, \neg C]\Prob_{\cP_1}[z_t=0, \neg C]\\
    &\leq \E_{\cP_1}[\theta|z_t=0, \cC]\Prob_{\cP_1}[z_t=0, \cC] + \frac{\tau\Prob_{\cP_1}[\theta<-\tau]}{2\tau\Prob_{\cP_1}[\theta<-\tau]+2} 
\end{align*}
We want to upper bound the first term. This can be done by splitting it into four cases based on the value of $\theta$. We have:

\begin{equation} 
    \begin{split}
    \E_{\cP_1}[\theta|z_t=0,\cC]\Prob_{\cP_1}[z_t=0, \cC] = 
    &\E_{\cP_1}[\theta|z_t=0, \cC, \theta \geq  2s_q]\Prob_{\cP_1}[z_t=0, \cC, \theta \geq 2s_q] \\
    &\ + \E_{\cP_1}[\theta|z_t=0, \cC, 0 \leq \theta < 2s_q]\Prob_{\cP_1}[z_t=0, \cC, 0 \leq \theta < 2s_q] \\
    &\ + \E_{\cP_1}[\theta|z_t=0, \cC, -\tau \leq \theta < 0]\Prob_{\cP_1}[z_t=0, \cC, -\tau \leq \theta < 0] \\
    &\ + \E_{\cP_1}[\theta|z_t=0, \cC, \theta \leq -\tau]\Prob_{\cP_1}[z_t=0, \cC, \theta < -\tau] \label{eq:racing-bic-cases-type1}
    \end{split}
\end{equation}

By definition of $s_q$, we have:
\begin{align*}
    2s_q &\leq 2s_{L_1}\\
    &\leq \frac{\tau\Prob_{\cP_1}[\theta<-\tau]}{2}-\nu\\
    &\leq \tau
\end{align*}

% \lscomment{End: Need to edit this part to prove that $s_q\leq s_L$ for all $q>L$}

Conditional on $\cC$, the empirical estimate $\hat{\theta}_q > \theta - s_q \geq 2s_q$. Hence, when we have $\theta \geq 2s_q$, then $\hat{\theta}\geq s_q$ and arm 0 must have already been eliminated at phase $q \geq L_1$. This implies that the probability $\Prob_{\cP_1}[z_t=0, \cC, \theta\geq 2s_q] = 0$. Similarly, when we have $\theta \leq -\tau \leq -2s_q$, then $\hat{\theta} \leq -s_q$ and arm 1 must have already been eliminated at phase $q \geq L_1$. Hence, arm 1 could not be recommended in that case and the probability $\Prob_{\cP_1}[z_t=0, \cC, \theta < -\tau] = \Prob_{\cP_1}[\cC, \tau < -\tau]$.\\
We can then rewrite equation~\eqref{eq:racing-bic-cases-type1} as
\begin{align*} 
    &\E_{\cP_1}[\theta|z_t=0, \cC]\Prob_{\cP_1}[z_t=0 ,\cC] \\
    = &\E_{\cP_1}[\theta|z_t=0, \cC, 0 \leq \theta < 2s_q]\Prob_{\cP_1}[z_t=0, \cC, 0 \leq \theta < 2s_q]\\
    &+ \E_{\cP_1}[\theta|z_t=0, \cC, -\tau \leq \theta < 0]\Prob_{\cP_1}[z_t=0, \cC, -\tau \leq \theta < 0]\\
    &+ \E_{\cP_1}[\theta|z_t=0, \cC, \theta < -\tau]\Prob_{\cP_1}[z_t=0, \cC, \theta < -\tau]\\
    \leq &-\tau \Prob_{\cP_1}[\cC, \theta < -\tau] + 0\cdot \Prob_{\cP_0}[z_t=1, \cC, -\tau \leq \theta < 0] + 2s_q \Prob_{\cP_1}[z_t=0, \cC, 0 \leq \theta < 2s_q]\\
    \leq &2s_q - \tau \Prob_{\cP_1}[\cC, \theta \leq -\tau]\\
    \leq &\frac{\tau\Prob_{\cP_1}[\theta<-\tau]}{2}-\nu - \tau \Prob_{\cP_1}[\cC, \theta < -\tau] \\
    \leq &\frac{\tau\Prob_{\cP_1}[\theta<-\tau]}{2}-\nu - \tau \Prob_{\cP_1}[\cC | \theta < -\tau] \Prob_{\cP_1}[\theta < -\tau]\\
    \leq &\frac{\tau\Prob_{\cP_1}[\theta<-\tau]}{2}-\nu - \tau (1 - \delta - \delta') \Prob_{\cP_1}[\theta < -\tau]\\
    = & \left(\frac{-1}{2} + \delta + \delta' \right) \tau \Prob_{\cP_1}[\theta < -\tau]-\nu\\
    \leq & \left(\frac{-1}{2} + \frac{\tau \Prob_{\cP_1}[\theta < -\tau]}{2\tau \Prob_{\cP_1}[\theta < -\tau] + 2} \right) \tau \Prob_{\cP_1}[\theta < -\tau]-\nu \tag{by Equation~\ref{eq:delta'-type1}}\\
    = & \frac{-1}{2} \left(\frac{\tau \Prob_{\cP_1}[\theta < -\tau] + 1 - \tau \Prob_{\cP_1}[\theta < -\tau]}{\tau \Prob_{\cP_1}[\theta < -\tau] + 1} \right)\tau \Prob_{\cP_1}[\theta < -\tau] - \nu\\
    = & \frac{-1}{2} \left(\frac{\tau \Prob_{\cP_1}[\theta < -\tau]}{\tau \Prob_{\cP_1}[\theta < -\tau] + 1} \right)+\nu
\end{align*}
Hence, we have 
\begin{align*}
    \E_{\cP_1}[\theta|z_t=0]\Prob_{\cP_1}[z_t=0] &\leq \E[\theta|z_t=0, \cC]\Prob_{\cP_1}[z_t=0, \cC] + \frac{\tau\Prob_{\cP_1}[\theta<-\tau]}{2\tau\Prob_{\cP_1}[\theta<-\tau]+2} \\
    &\leq \frac{-\tau\Prob_{\cP_1}[\theta<-\tau]}{2\tau\Prob_{\cP_1}[\theta<-\tau]+2}-\nu  +  \frac{\tau\Prob_{\cP_1}[\theta<-\tau]}{2\tau\Prob_{\cP_1}[\theta<-\tau]+2} \\
    &= -\nu \leq \phi(u_t)
\end{align*}
Therefore, Algorithm~\ref{alg:racing-two-types-mixed-preferences} fulfills equation~\ref{eq:racing-bic-type1} and is BIC for all agents of type 1.
\end{proof}

%%%%%%%%%%%%%%%%%%%%%%%%%%%%%%%%%%%%%%%%%%%%%%%%%%%%%%%%%%%%%%%%%

\subsubsection{Racing Stage Second Part Estimation Bound}
\lscomment{Fix this proof so the Union Bound is made more explicit and maybe change the phrase ``Estimation Bound.''}
\label{sec:racing-estimation-bound-second}
\racingestimationboundsecond*
\begin{proof}
    We assume \cref{alg:racing-two-types-mixed-preferences} to be initialized with parameters (see \cref{lemma:bic-racing-control-treatment-0,lemma:bic-racing-control-treatment-1} for details) such that its recommendations are BIC for all agents. Therefore, we may apply \cref{thm:approximation-bound-denominator} where we let the proportion $p_{BIC}=1$. Finally, we combine the high probability bound on the denominator with the high probability bound on the numerator (given by \cref{thm:treatment-approximation-bound}), taking a union bound to achieve the confidence parameters $\delta$.
\end{proof}
