# Supplementary material for: Incentivizing Compliance with Algorithmic Instruments
Source: arXiv:2107.10093 source file (2021-07-28)
Supplement: Supplementary file 4 [file expected-g-zero-without-centering.tex]

\subsection{Finite Sample Analysis Proof}
\label{sec:general-approximation-bound-proof}
Given $n \in \RR$ samples $\left\{(z_i, x_i, y_i)\right\}_{i=1}^n$, of the recommendation $z_i$, action $x_i$, and reward $y_i$ at each round $i$, we would like to bound the difference between the predicted exogenous treatment effect, denoted $\hat{\theta}_n$, and the true exogenous treatment effect $\theta$. \lscomment{should we use the phrase `exogenous treatment effect' or something else like `latent treatment effect'?} 

\subsubsection{IV Estimate}
First, we form the estimate $\hat{\theta}_n$ of $\theta$ via Two-Stage Least Squares (2SLS) regression. In the first stage, we form the estimate $\hat{\beta}_n$ of $\beta$ by regressing $y_i$ onto $z_i$ and the estimate $\hat{\Gamma}_n$ of $\Gamma$ by regressing $x_i$ onto $z_i$:
\begin{equation}
    \hat{\beta}_n = \bigg(\sum_{i=1}^nz_iz_i^\intercal\bigg)^{-1}\sum_{i=1}^ny_iz_i
    \hspace{.4cm}
    \text{ and }
    \hspace{.4cm}
    \hat{\Gamma}_n = \bigg(\sum_{i=1}^nz_iz_i^\intercal\bigg)^{-1}\sum_{i=1}^nz_ix_i^\intercal
\end{equation}

Second, we take the inverse of $\Gamma$ times $\beta$ as the predicted causal effect vector $\hat{\theta}_n$:
\begin{align*}
    \hat{\theta}_n
    &= \hat{\Gamma}_n^{-1}\hat{\beta}_n\\
    &= \bigg(\sum_{i=1}^nz_ix_i^\intercal\bigg)^{-1}\bigg(\sum_{i=1}^nz_iz_i^\intercal\bigg)\bigg(\sum_{i=1}^nz_iz_i^\intercal\bigg)^{-1}\sum_{i=1}^nz_iy_i\\
    &= \bigg(\sum_{i=1}^nz_ix_i^\intercal\bigg)^{-1}\sum_{i=1}^nz_iy_i
\end{align*}

Note that the sum of the outer product $\sum_{i=1}^nz_ix_i$ must be full rank in order to form a meaningful estimate of $\theta$. Next, we bound the difference between the treatment effect vector $\theta$ and its estimate $\hat{\theta}_n$.

\subsubsection{Finite Sample Bound on the Difference between the Treatment Effect and IV Estimate}
By the standard argument with the law of large numbers, we could show that $\hat{\theta}_n$ is a consistent estimator of the treatment effect vector $\theta$, insofar as the L2-norm of the difference between $\theta$ and $\hat{\theta}_n$, denoted $\norm{\hat{\theta}_n-\theta}_2=0$, when $n$ approaches infinity. However, in our setting, we are more interested in upper bounding this difference between $\theta$ and $\hat{\theta}_n$ for finite $n$.

In order to do so, we first reformulate the L2-norm of the difference between $\theta$ and $\hat{\theta}_n$ in terms of entirely empirical terms, namely $z_i, x_i, g(u_i)$ and $\eps_i$. Second, in \Cref{eq:general-approximation-bound-numerator} we provide a high-probability upper bound on the numerator of our finite sample IV estimation bound in \Cref{eq:finite-sample-bound-numerator-denominator}; at this point, we are able to use the bound we obtain within \Cref{alg:multi-arm-racing}.

Lastly, we provide a number \lscomment{three, probably} of high-probability lower bounds on the denominator of our bound in \Cref{eq:finite-sample-bound-numerator-denominator}. Since the term $\sum_{i=1}^n z_ix_i^{\intercal}$ relies on the interactions between the recommendation $z_i$ and the agents' chosen action $x_i$ over each round $i$, the lower bound on the denominator depends on how compliant agents are to our recommendations at each stage of our algorithm. \lscomment{cite the three lemmas for estimation bounds at each stage of the algorithm. also maybe change the terminology of `stages' versus `phases' and such...}

First, the L2-norm of the difference between $\theta$ and $\hat{\theta}_n$ is given as:
\begin{align}
    \norm{\hat{\theta}_n - \theta}_2
    &= \norm{\bigg(\sum_{i=1}^nz_ix_i^\intercal\bigg)^{-1}\sum_{i=1}^nz_iy_i}_2 \nonumber\\
    &= \norm{\bigg(\sum_{i=1}^nz_ix_i^\intercal\bigg)^{-1}\sum_{i=1}^nz_i\left(\langle\theta,x_i\rangle + g(u_i) + \epsilon_i\right)^\intercal\bigg) - \theta}_2 \nonumber\\
    &= \norm{\bigg(\sum_{i=1}^nz_ix_i^\intercal\bigg)^{-1}\sum_{i=1}^nz_i\left(x_i^\intercal\theta + g(u_i) + \epsilon_i\right)\bigg) - \theta}_2 \nonumber\\
    &= \norm{\theta + \bigg(\sum_{i=1}^nz_ix_i^\intercal\bigg)^{-1}\sum_{i=1}^nz_i\left(g(u_i) + \epsilon_i\right) - \theta}_2 \nonumber\\
    &= \norm{\bigg(\sum_{i=1}^nz_ix_i^\intercal\bigg)^{-1}\sum_{i=1}^nz_i\left(g(u_i) + \epsilon_i\right)}_2 \label{eq:l2-norm-difference-empirical-terms}\\
    &\leq \norm{\bigg(\sum_{i=1}^nz_ix_i^\intercal\bigg)^{-1}}_2\norm{\sum_{i=1}^nz_i(g(u_i)+\epsilon_i)}_2\tag{by Cauchy-Schwarz \lscomment{cite theorem}} \nonumber\\
    &= \frac{\norm{\sum_{i=1}^nz_i(g(u_i)+\epsilon_i)}_2}{\sigma_{\min}\left\{\sum_{i=1}^nz_ix_i^\intercal\right\}} \label{eq:finite-sample-bound-numerator-denominator},
\end{align}
where $\sigma_{\min}\{\cdot\}$ denotes the minimum singular value.

Now, we upper bound the numerator of \Cref{eq:finite-sample-bound-numerator-denominator} above in the following \Cref{eq:general-approximation-bound-numerator}:
\begin{lemma}\label{eq:general-approximation-bound-numerator}
For some $\delta \in (0,1)$, with probability at least $1-\delta$, we have
\begin{equation}
    \norm{\sum_{i=1}^nz_i(g(u_i)+\epsilon_i)}_2 \leq \left(2\Upsilon+\sigma_{\eps}\right)\sqrt{2nk\log(2k/\delta)}
\end{equation}
\begin{proof} We can express the L2-norm of the sum in the numerator of \Cref{eq:finite-sample-bound-numerator-denominator} as such:
    \begin{align*}
        \norm{\sum_{i=1}^n (g(u_i)+\epsilon_i)z_i}_2
        &=\sqrt{\sum_{j=1}^k\left(\sum_{i=1}^n (g(u_i)+\epsilon_i)\1[z_i=\e_j]\right)^2}\\
        &=\sqrt{\sum_{j=1}^k\left(\sum_{i=1}^{n_j} (g(u_i)+\epsilon_i)\right)^2}\tag{where $n_j=\sum_{i=1}^n\1[z_i=\e_j]$}\\
        &\leq \sqrt{\sum_{j=1}^k\left(2\Upsilon\sqrt{\frac{n_j\log(1/\delta_j)}{2}} + \sigma_{\eps}\sqrt{2n_j\log(1/\delta_j')}\right)^2} \tag{by Chernoff Bound and since $\E[g(u)]=0$ \lscomment{refer to theorems}}\\
        &\leq \sqrt{\sum_{j=1}^k\left(2\Upsilon\sqrt{\frac{n_j\log(2k/\delta)}{2}} + \sigma_{\eps}\sqrt{2n_j\log(2k/\delta)}\right)^2} \tag{by Union Bound with $\delta=\sum_{j=1}^k\delta_j+\delta_j'$}\\
        &\leq\sqrt{k\left(2\Upsilon\sqrt{\frac{n\log(2k/\delta)}{2}} + \sigma_{\eps}\sqrt{2n\log(2k/\delta)}\right)^2} \tag{since $n_j\leq n$ for all $j$}\\
        &=\sqrt{k}\left(2\Upsilon\sqrt{\frac{n\log(2k/\delta)}{2}} + \sigma_{\eps}\sqrt{2n\log(2k/\delta)}\right)\\
        &\leq (2\Upsilon+\sigma_{\eps})\sqrt{2nk\log(2k/\delta)} \tag{since $\sqrt{\frac{n\log(2k/\delta)}{2}}\leq\sqrt{2n\log(2k/\delta)}$}
    \end{align*}
\end{proof}
\end{lemma}

Next, we bound the denominator.
