# Supplementary material for: Incentivizing Compliance with Algorithmic Instruments
Source: arXiv:2107.10093 source file (2021-07-28)
Supplement: Supplementary file 5 [file appendix-many-arms-many-types.tex]

\section{Many Arms \& Many Types}

\subsection{Sampling Stage BIC Proof}
\Cref{lemma:bic-general-sampling}:
\bicgeneralsampling*

\begin{proof} Agent $t$ in phase $i$ of the algorithm is recommended either arm 1 or arm $i$. We
need to prove incentive-compatibility for type $\kappa$ for the two cases separately.
Let $\xi^i_{\kappa}$ be the event that the exploit arm $a^* = i$ in phase $i$ when we calibrate the algorithm to type $\kappa$, i.e.
\begin{equation}
    \xi^i_{\kappa} := \left\{ \bar{y}_{\ell_1}^1 + C \leq \min_{1<j<i} \bar{y}_{\ell_1}^j - C \ \text{ and } \ \max_{1<j<i} \bar{y}_{\ell_1}^j + C \leq \mu_{\kappa}^i \right\}.
\end{equation}

\paragraph{Part I (Recommendation for arm i):} We first argue that an agent $t$ of type $\kappa$ who is recommended arm $i$ will not switch to any other arm $j$. For arms $j > i$, there is no information about arms $i$ or $j$ collected by the algorithm and by assumption, we have $\mu^i_{\kappa} \geq \mu^j_{\kappa}$. Hence, it suffices to consider when $j<i$. We want to show that
    \begin{equation}
        \label{eq:bic-sample-many-arms-types}
        \E_{\cP_{\kappa}}[\theta^j - \theta^1 | z_t = \e_i] \Prob_{\cP_{\kappa}}[z_t = \e_i] \geq 0.
    \end{equation}
Agent $t$ is in the explore group $Q$ with probability $1/\rho_{\kappa}$ and in the exploit group $P - Q$ with probability $1 - (1/\rho_{\kappa})$. Since being in the explore group does not confer any information about the mean rewards of any arm, the expected gain from choosing arm $i$ over arm $j$ conditional on the agent $t$ being in the explore group is $\mu^i_{\kappa} - \mu^j_{\kappa}$. Since $\mu^i_{\kappa} \leq \mu^j_{\kappa}$ for all $j < i$, this difference $\mu^i_{\kappa} - \mu^j_{\kappa} \leq 0$. If the agent is in the exploit group, then a recommendation of arm $i$ implies that the event $\xi^i_{\kappa}$ has happened. Hence, we have:
    \begin{equation*}
        \E_{\cP_{\kappa}}[\mu^i_{\kappa} - \theta^j | z_t = \e_i] \Prob_{\cP_{\kappa}}[z_t = \e_i] = \E_{\cP_{\kappa}}[\mu^i_{\kappa} - \theta^j | \xi^i_{\kappa}] \Prob_{\cP_{\kappa}}[\xi^i_{\kappa}] \left(1 - \frac{1}{\rho_{\kappa}}\right) + \frac{\mu^i_{\kappa} - \mu^j_{\kappa}}{\rho_{\kappa}}.
    \end{equation*}

For the algorithm to be incentive-compatible for type $\kappa$, we must pick $\rho_{\kappa}$ large enough so that:
    \begin{align}
        \E_{\cP_{\kappa}}[\mu^i_{\kappa} - \theta^j | \xi^i_{\kappa}] \Prob_{\cP_{\kappa}}[\xi^i_{\kappa}] \left(1 - \frac{1}{\rho_{\kappa}}\right) + \frac{\mu^i_{\kappa} - \mu^j_{\kappa}}{\rho_{\kappa}} &\geq 0 \nonumber\\
    	\Leftrightarrow \frac{-1}{\rho_{\kappa}} \left[ \E_{\cP_{\kappa}}[\theta_0^i - \theta^j|\hat{\xi}_i] \Prob_{\cP_{\kappa}}[\hat{\xi}_i] + \mu^j_{\kappa} - \mu^i_{\kappa} \right] &\geq -\E_{\cP_{\kappa}}[\mu^i_{\kappa} - \theta^j | \xi^i_{\kappa}] \Prob_{\cP_{\kappa}}[\xi^i_{\kappa}] \nonumber\\
    	\Leftrightarrow \frac{1}{\rho_{\kappa}} &\leq \frac{\E_{\cP_{\kappa}}[\mu^i_{\kappa} - \theta^j | \xi^i_{\kappa}] \Prob_{\cP_{\kappa}}[\xi^i_{\kappa}]}{ \E_{\cP_{\kappa}}[\theta_0^i - \theta^j|\hat{\xi}_i] \Prob_{\cP_{\kappa}}[\hat{\xi}_i] + \mu^j_{\kappa} - \mu^i_{\kappa}} \nonumber\\
    	\Leftrightarrow \rho_{\kappa} &\geq 1 + \frac{\mu^j_{\kappa} - \mu^i_{\kappa}}{\underset{\cP_{\kappa}}{\E}[\mu^i_{\kappa} - \theta^j | \xi^i_{\kappa}] \underset{\cP_{\kappa}}{\Prob}[\xi^i_{\kappa}]} \label{eq:multi-arm-type-rho-condition}
    \end{align}

This comes down to finding a lower bound on the denominator of the expression above. First, we define a clean event $C'$ where the average error $\frac{1}{\ell_1}\sum_{i=1}^{\ell_1} \epsilon_i$ of the first $\ell_1$ samples of arm 1 is bounded (following Corollary \ref{thm:high-prob-unbounded-chernoff}):
\begin{equation}
     C' := \left \{ \bigg\vert\frac{1}{\ell_1} \sum_{i=1}^{\ell_1} \epsilon_i \bigg\vert \leq \sigma_\epsilon \sqrt{\frac{2\log(1/\delta)}{\ell_1}} \right \}.
\end{equation}
The event $C'$ occurs with probability at least $1 - \delta$ for $\displaystyle \delta < \delta' := \frac{\Prob_{\cP_{\kappa}}[\xi^i_{\kappa}]}{16}$.

We have 
\begin{align}
    \E_{\cP_{\kappa}}[\mu^i_{\kappa} - \theta^j | \xi^i_{\kappa}] \Prob_{\cP_{\kappa}}[\xi^i_{\kappa}] &= \E_{\cP_{\kappa}}[\mu^i_{\kappa} - \theta^j | \xi^i_{\kappa}, C'] \Prob_{\cP_{\kappa}}[\xi^i_{\kappa}, C'] + \E_{\cP_{\kappa}}[\mu^i_{\kappa} - \theta^j | \xi^i_{\kappa}, \neg C'] \Prob_{\cP_{\kappa}}[\xi^i_{\kappa}, \neg C'] \nonumber\\
    &\geq \E_{\cP_{\kappa}}[\mu^i_{\kappa} - \theta^j | \xi^i_{\kappa}, C'] \Prob_{\cP_{\kappa}}[\xi^i_{\kappa}, C'] - \delta \tag{since $\mu^i_{\kappa} - \theta^j \geq -1$ and $\Prob_{\cP_{\kappa}}[\neg C']<\delta$} \nonumber\\
    &= \E_{\cP_{\kappa}}[\mu^i_{\kappa} - \theta^j | \xi^i_{\kappa}, C'] (\Prob_{\cP_{\kappa}}[\xi^i_{\kappa}] - \Prob_{\cP_{\kappa}}[\xi^i_{\kappa}, \neg C']) - \delta \nonumber\\
    &\geq \E_{\cP_{\kappa}}[\mu^i_{\kappa} - \theta^j | \xi^i_{\kappa}, C'] (\Prob_{\cP_{\kappa}}[\xi^i_{\kappa}] - \Prob_{\cP_{\kappa}}[\neg C']) - \delta \nonumber\\
    &\geq \E_{\cP_{\kappa}}[\mu^i_{\kappa} - \theta^j | \xi^i_{\kappa}, C'] (\Prob_{\cP_{\kappa}}[\xi^i_{\kappa}] - \delta) - \delta \nonumber\\
    &= \E_{\cP_{\kappa}}[\mu^i_{\kappa} - \theta^j | \xi^i_{\kappa}, C'] \Prob_{\cP_{\kappa}}[\xi^i_{\kappa}] - \delta(1 + \E_{\cP_{\kappa}}[\mu^i_{\kappa} - \theta^j | \xi^i_{\kappa}, C']) \nonumber\\
    &\geq \E_{\cP_{\kappa}}[\mu^i_{\kappa} - \theta^j | \xi^i_{\kappa}, C'] \Prob_{\cP_{\kappa}}[\xi^i_{\kappa}] - 2\delta \label{eq:sampling-two-arm-clean-event}
\end{align}

This comes down to finding a lower bound on the denominator of the expression above. We can reduce the dependency of the denominator to a single prior-dependent constant $\Prob_{\cP_{\kappa}}[\xi^i_{\kappa}]$ if we lower bound the prior-dependent expected value $\E_{\cP_{\kappa}}[\mu^i_{\kappa} - \theta^j | \xi^i_{\kappa}]$. That way, assuming we know the prior and can calculate the probability of event $\xi^i_{\kappa}$, we can pick an appropriate $\rho_{\kappa}$ to satisfy the BIC condition for all agents of type $\kappa$ (see Definition~\ref{def:bic}). Remember that event
\begin{equation}
    \xi^i_{\kappa} = \{ \bar{y}_{\ell_1}^1 + C \leq \min_{1<j<i} \bar{y}_{\ell_1}^j - C \ \text{ and } \ \max_{1<j<i} \bar{y}_{\ell_1}^j + C \leq \mu_{\kappa}^i\}
\end{equation}
where $C = \Upsilon + \sigma_{\epsilon}\sqrt{\frac{2\log(1/\delta)}{\ell_1}} + \frac{1}{4}$. Then, the expected value
\begin{align}
    \E_{\cP_{\kappa}}[\mu^i_{\kappa} - \theta^j | \xi^i_{\kappa}, C'] 
    &= \mu_{\kappa}^i - \E_{\cP_{\kappa}}\left[\theta^j \middle| \Upsilon + \sigma_{\epsilon}\sqrt{\frac{2\log(1/\delta)}{\ell_1}} + \frac{1}{4}  + \bar{y}^1_{\ell_1}< \mu_i^2, C'\right] \nonumber\\
    &= \mu_{\kappa}^i - \E_{\cP_{\kappa}}\left[\theta^j \middle| \Upsilon + \sigma_{\epsilon}\sqrt{\frac{2\log(1/\delta)}{\ell_1}} + \frac{1}{4}  +  \frac{1}{\ell_1}\sum_{t=1}^{\ell_1} y_t^1< \mu_{\kappa}^i, C'\right] \nonumber\\
    &= \mu_{\kappa}^i - \E_{\cP_{\kappa}}\left[\theta^j \middle| \Upsilon + \sigma_{\epsilon}\sqrt{\frac{2\log(1/\delta)}{\ell_1}} + \frac{1}{4}  + \frac{1}{\ell_1}\sum_{t=1}^{\ell_1} \theta^j + g(u_t) + \epsilon_t  < \mu_{\kappa}^i, C'\right] \nonumber\\
    &= \mu_{\kappa}^i - \E_{\cP_{\kappa}}\left[\theta^j \middle| \theta^j + \Upsilon + \sigma_{\epsilon}\sqrt{\frac{2\log(1/\delta)}{\ell_1}} + \frac{1}{4} + \frac{1}{\ell_1}\sum_{t=1}^{\ell_1} g(u_t) + \epsilon_t  < \mu_{\kappa}^i, C'\right] \nonumber\\
    &> \mu_{\kappa}^i - \E_{\cP_{\kappa}}\left[\theta^1 \middle| \theta^j + \Upsilon + \sigma_{\epsilon}\sqrt{\frac{2\log(1/\delta)}{\ell_1}} + \frac{1}{4} - \Upsilon - \sigma_{\epsilon}\sqrt{\frac{2\log(1/\delta)}{\ell_1}} < \mu_{\kappa}^i\right] \tag{since $g(u_t) > -\Upsilon$ and $\frac{1}{\ell_1}\sum_{t=1}^{\ell_1}\epsilon_t > -\sigma_\epsilon \sqrt{\frac{2\log(1/\delta)}{\ell_1}}$ by event $C'$} \nonumber\\
    &> \mu_{\kappa}^i - \E_{\cP_{\kappa}}\left[\theta^j \middle| \theta^j + \frac{1}{4} < \mu_{\kappa}^i\right] \nonumber\\
    &> \frac{1}{4} 
    \label{eq:sampling-stage-multi-arm-gap}
\end{align}
Hence, the lower bound on the denominator is
\begin{align}
    \E_{\cP_{\kappa}}[\mu^i_{\kappa} - \theta^j | \xi^i_{\kappa}] \Prob_{\cP_{\kappa}}[\xi^i_{\kappa}] &\geq \E_{\cP_{\kappa}}[\mu^i_{\kappa} - \theta^j | \xi^i_{\kappa}, C']\Prob_{\cP_{\kappa}}[\xi^i_{\kappa}] - 2\delta \tag{by Equation \ref{eq:sampling-two-arm-clean-event}}\\
    &> \frac{1}{4}\Prob_{\cP_{\kappa}}[\xi^i_{\kappa}] - 2\delta \tag{by Equation \ref{eq:sampling-stage-two-arm-gap}}\\
    &= \frac{1}{8}\Prob_{\cP_{\kappa}}[\xi^i_{\kappa}] + \frac{1}{8}\Prob_{\cP_{\kappa}}[\xi^i_{\kappa}] - 2\delta \\ 
    &= 2\delta' + \frac{\Prob_{\cP_{\kappa}}[\xi^i_{\kappa}]}{8} - 2\delta\tag{since $\delta' = \frac{1}{8} \Prob_{\cP_{\kappa}}[\xi^i_{\kappa}]$}\\
    &\geq \frac{\Prob_{\cP_{\kappa}}[\xi^i_{\kappa}]}{8} \tag{since $\delta < \delta'$}
\end{align}
Hence, we can pick :
\begin{align*}
    \rho_{\kappa} &\geq 1 + \frac{8(\mu_{\kappa}^j - \mu_{\kappa}^j)}{\Prob_{\cP_{\kappa}}[\xi^i_{\kappa}]}
\end{align*}
to satisfy the BIC condition for all agents of type $\kappa$.
    
\paragraph{Part II (Recommendation for arm 1):} When agent $t$ is recommended arm 1, they know that they are not in the explore group $Q$. Therefore, they know that the event $\neg \xi^i_{\kappa}$ occurred. \ls{But, the agent does not know which round they are in. So, we must show that for any $i$, they wouldn't switch.} Thus, in order to prove that Algorithm~\ref{alg:general-sampling} is BIC for an agent of type $\kappa$, we need to show the following for any arm $j > 1$:
\begin{equation}
    \label{eq:sampling-multi-arm-type-rec-1}
    \E_{\cP_{\kappa}}[\theta^1 - \theta^j | z_t=e_1]\Prob_{\cP_{\kappa}}[z_t=e_1] = \E_{\cP_{\kappa}}[\theta^1 - \theta^j | \neg \xi^i_{\kappa}]\Prob_{\cP_{\kappa}}[\neg \xi^i_{\kappa}]\geq 0
\end{equation}

Again, there is no information collected by the algorithm about any arm $j\geq i$ and, by assumption, $\mu^1_{\kappa} \geq \mu^j_{\kappa}$. Hence, it suffices to consider arms $j<i$. Observe that:
    \begin{align*}
        \E_{\cP_{\kappa}}[\theta^1 - \theta^j | \neg \xi^i_{\kappa}]\Prob_{\cP_{\kappa}}[\neg \xi^i_{\kappa}] 
        &= \E_{\cP_{\kappa}}[\theta^1 - \theta^j] - \E_{\cP_{\kappa}}[\theta^1 - \theta^j | \xi^i_{\kappa}]\Prob_{\cP_{\kappa}}[\xi^i_{\kappa}] \\
        &= \mu^1_{\kappa} - \mu^j_{\kappa} + \E_{\cP_{\kappa}}[\theta^j - \theta^1 | \xi^i_{\kappa}]\Prob_{\cP_{\kappa}}[\xi^i_{\kappa}]
    \end{align*}
By definition $\mu^1_{\kappa} - \mu^j_{\kappa} \geq 0$. Thus, in order to fulfill Equation~\eqref{eq:sampling-multi-arm-type-rec-1}, it would suffice to show that $\E_{\cP_{\kappa}}[\theta^j - \theta^1 | \xi^i_{\kappa}]\Prob_{\cP_{\kappa}}[\xi^i_{\kappa}] \geq 0$.\\
With event $C'$ defined above, we have 
\begin{align}
    \E_{\cP_{\kappa}}[\theta^j - \theta^1 | \xi^i_{\kappa}] \Prob_{\cP_{\kappa}}[\xi^i_{\kappa}] &= \E_{\cP_{\kappa}}[\theta^j - \theta^1 | \xi^i_{\kappa}, C'] \Prob_{\cP_{\kappa}}[\xi^i_{\kappa}, C'] + \E_{\cP_{\kappa}}[\theta^j - \theta^1 | \xi^i_{\kappa}, \neg C'] \Prob_{\cP_{\kappa}}[\xi^i_{\kappa}, \neg C'] \nonumber\\
    &\geq \E_{\cP_{\kappa}}[\theta^j - \theta^1 | \xi^i_{\kappa}, C'] \Prob_{\cP_{\kappa}}[\xi^i_{\kappa}, C'] - \delta \tag{since $\theta^j - \theta^1 \geq -1$ and $\Prob_{\cP_{\kappa}}[\neg C']<\delta$} \nonumber\\
    &= \E_{\cP_{\kappa}}[\theta^j - \theta^1 | \xi^i_{\kappa}, C'] (\Prob_{\cP_{\kappa}}[\xi^i_{\kappa}] - \Prob_{\cP_{\kappa}}[\xi^i_{\kappa}, \neg C']) - \delta \nonumber\\
    &\geq \E_{\cP_{\kappa}}[\theta^j - \theta^1 | \xi^i_{\kappa}, C'] (\Prob_{\cP_{\kappa}}[\xi^i_{\kappa}] - \Prob_{\cP_{\kappa}}[\neg C']) - \delta \nonumber\\
    &\geq \E_{\cP_{\kappa}}[\theta^j - \theta^1 | \xi^i_{\kappa}, C'] (\Prob_{\cP_{\kappa}}[\xi^i_{\kappa}] - \delta) - \delta \nonumber\\
    &= \E_{\cP_{\kappa}}[\theta^j - \theta^1 | \xi^i_{\kappa}, C'] \Prob_{\cP_{\kappa}}[\xi^i_{\kappa}] - \delta(1 + \E_{\cP_{\kappa}}[\theta^j - \theta^1 | \xi^i_{\kappa}, C']) \nonumber\\
    &\geq \E_{\cP_{\kappa}}[\theta^j - \theta^1 | \xi^i_{\kappa}, C'] \Prob_{\cP_{\kappa}}[\xi^i_{\kappa}] - 2\delta \label{eq:sampling-two-arm-clean-event}
\end{align}

When event $\xi^i_{\kappa}$ occurs, we have the following:
\ls{Should we denote the constants $C$ differently? Is it too messy?}
\ls{We separate the $C_1$ and $C_j$ because we need to take separate Chernoff bounds for two separate samples collected from samples of arm 1 and arm $j$. We do this again in the proof below, except we subtract it. Note that the summations in the third line from the bottom in the system of inequalities below are over the same respective samples from arms 1 and $j$. Thus, the Chernoff bounds are equivalent and cancel to equal 0.}
% \begin{align*}
%     \bar{y}^j_{\ell_1} - \bar{y}^1_{\ell_1} 
%     &> C_1 + C_j\\
%         \E[y^j] - \E[y^1]
%     &> C_1 + C_j + \bar{y}^1_{\ell_1} -  \bar{y}^j_{\ell_1} + \E[y_j] - E[y_1]\\
%         \theta^j + \E[g(u_t)] - \theta^1 - \E[g(u_t)]
%     &> C_1 + C_j + \frac{1}{\ell_1}\sum_{t_1=1}^{\ell_1}[\theta^1 + (u_{t_1}) + \epsilon_{t_1}] - \frac{1}{\ell_1}\sum_{t_j=1}^{\ell_1}[\theta^j + g(u_{t_j}) + \epsilon_{t_j}] \\
%     &\hspace{1,5cm}+ \theta^j + \E[g(u_t)] - \theta^1 - \E[g(u_t)]\\
%         \theta^j - \theta^1 
%     &> C_1 + C_j + \frac{1}{\ell_1}\sum_{t_1=1}^{\ell_1}[g(u_{t_1}) + \epsilon_{t_1}] - \frac{1}{\ell_1}\sum_{t_j=1}^{\ell_1}[g(u_{t_j}) + \epsilon_{t_j}]\\
%     &> 2\Upsilon + \sigma_{\epsilon} \sqrt{\frac{2\log(1/\delta_1)}{\ell_1}} + \sigma_{\epsilon}\sqrt{\frac{2\log(1/\delta_2)}{\ell_1}} - 2\Upsilon\\
%     &\hspace{1.5cm} - \sigma_{\epsilon} \sqrt{\frac{2\log(1/\delta_1)}{\ell_1}} - \sigma_{\epsilon}\sqrt{\frac{2\log(1/\delta_2)}{\ell_1}}\\
%     &= 0.
% \end{align*} 

\begin{align}
    &\quad\E_{\cP_{\kappa}}[\theta^j - \theta^1 | \xi^i_{\kappa}, C']\\ 
    &= \theta^j - \E_{\cP_{\kappa}}\left[\theta^1 \middle| C_1 + C_J + \bar{y}^1_{\ell_1}< \bar{y}^j_{\ell_1}, C'\right] \nonumber\\
    &= \theta^j - \E_{\cP_{\kappa}}\left[\theta^1 \middle| 2\Upsilon + 2\sigma_{\epsilon}\sqrt{\frac{2\log(1/\delta)}{\ell_1}} + \frac{1}{2} + \bar{y}^1_{\ell_1}< \bar{y}^j_{\ell_1}, C'\right] \nonumber\\
    &= \theta^j - \E_{\cP_{\kappa}}\left[\theta^1 \middle| 2\Upsilon + 2\sigma_{\epsilon}\sqrt{\frac{2\log(1/\delta)}{\ell_1}} + \frac{1}{2} + \frac{1}{\ell_1}\sum_{t=1}^{\ell_1} y_t^1< \frac{1}{\ell_1}\sum_{t=1}^{\ell_1} y_t^j, C'\right] \nonumber\\
    &= \theta^j - \E_{\cP_{\kappa}}\left[\theta^1 \middle| 2\Upsilon + 2\sigma_{\epsilon}\sqrt{\frac{2\log(1/\delta)}{\ell_1}} + \frac{1}{2}  + \frac{1}{\ell_1}\sum_{t=1}^{\ell_1} \theta^1 + g(u_t) + \epsilon_t  < \frac{1}{\ell_1}\sum_{t=1}^{\ell_1} \theta^j + g(u_t) + \epsilon_t, C'\right] \nonumber\\
    &= \theta^j - \E_{\cP_{\kappa}}\left[\theta^1 \middle| \theta^1 + 2\Upsilon + 2\sigma_{\epsilon}\sqrt{\frac{2\log(1/\delta)}{\ell_1}} + \frac{1}{2} + \frac{1}{\ell_1}\sum_{t=1}^{\ell_1} \left( g(u_t) + \epsilon_t\right) - \frac{1}{\ell_1}\sum_{t=1}^{\ell_1} \left( g(u_t) + \epsilon_t\right) < \theta^j, C'\right] \nonumber\\
    &> \theta^j - \E_{\cP_{\kappa}}\left[\theta^1 \middle| \theta^1 + 2\Upsilon + 2\sigma_{\epsilon}\sqrt{\frac{2\log(1/\delta)}{\ell_1}} + \frac{1}{2} - 2\Upsilon - 2\sigma_{\epsilon}\sqrt{\frac{2\log(1/\delta)}{\ell_1}} < \theta^j\right] \tag{since $\abs{g(u_t)} < \Upsilon$ and $\bigg\vert\frac{1}{\ell_1}\sum_{t=1}^{\ell_1}\epsilon_t \bigg\vert> -\sigma_\epsilon \sqrt{\frac{2\log(1/\delta)}{\ell_1}}$ by event $C'$} \nonumber\\
    &> \theta^j - \E_{\cP_{\kappa}}\left[\theta^1 \middle| \theta^1 + \frac{1}{2} < \theta^j\right] \nonumber\\
    &> \frac{1}{2} 
\end{align}
This demonstrates Equation~\eqref{eq:sampling-multi-arm-type-rec-1} and proves that agents of type $\kappa$ will take arm 1 when recommended it in any phase $i$. In fact, the above proof for Part II is applicable to any type $\kappa$ in any phase $i$. So, every agent will take arm 1 if they are recommended it. \ls{Think of a better way to express this.}\\
Therefore, Algorithm~\ref{alg:general-sampling} is BIC for all agents of type $\kappa$ when we set the exploration probability $\rho_{\kappa}$ to be 
\begin{align*}
    \rho_{\kappa} &\geq 1 + \frac{8(\mu_{\kappa}^j - \mu_{\kappa}^j)}{\Prob_{\cP_{\kappa}}[\xi^i_{\kappa}]}
\end{align*}
    and agents of all types will always comply with a recommendation for arm 1.
    
\ls{Note that the summations here are over $t_i$ for some arm $i$. This should be replaced with something clearer or just explain what it is (iterating over rounds $t$ that just contain samples of arm $i$).}
\end{proof}

\subsection{Racing Stage BIC Proof}
Lemma~\ref{lemma:racing-bic-many-types-1st-group}:
\bicracingmanytypesfirst*

\begin{proof}
We want to show that for any agent at time $t$ with a type $i<\kappa$ in the racing stage and for any two arms $a,b \in B:$
\begin{align*}
    \E_{\cP_i}[\theta^a - \theta^b | z_t=e_a]\Prob_{\cP_i}[z_t=e_a] \geq 0
\end{align*}
We will prove a stronger statement:
\begin{align*}
    \E_{\cP_i}[\theta^a - \max_{b \neq a} \theta^b| z_t=e_a]\Prob_{\cP_i}[z_t=e_a] \geq 0
\end{align*}
For each pair of arms $a,b \in B$, denote $G_{ab} = \theta^a - \theta^b$ and 
\begin{align*}
    G_a = \theta^a - \max_{b \neq a} \theta^b = \min_{b \neq a} G_{ab}.
\end{align*}

 Let 
\[s_q := \frac{12\sqrt{\log(2T/\delta) + (k+1)\log(2T(k+\Upsilon^2))}}{\left(\sigma_{\min}\{\hat{\Gamma}\}\right)^2 \sqrt{q}}\] be the decision threshold for each phase $q \geq \ell_1$ in Algorithm~\ref{alg:racing-many-types-two-phases}. Assume that after elimination, at every iteration a sample of the eliminated arm is also drawn, but not revealed to the agent.\\
We define the event $\cC_1$ as the accuracy guarantee of $\hat{\theta}$ such that:
\begin{equation}
\label{eq:event-C-1}
    \cC_1 := \left\{ \forall q \geq \ell_1: |G - \hat{G}_n| < s_q \right\}
\end{equation}
where $\ell_1$ is the number of samples of each arm after running the sampling stage.\\
Let $X^a_q$ be the number of arm $a$ samples in phase $q$. We also define event $\cC^a_2$ where there is at least one sample of arm $a$ in each phase:
\begin{equation}
    \cC^a_2 := \left\{\forall q: X^a_q >= 1 \right\}
\end{equation}
Then, let the clean event $\cC_2$ be the event where there is at least one sample from every arm in each phase, i.e.
\begin{equation}
\label{eq:event-C-2-many-types}
    \cC_2 := \bigcap_{1\leq a \leq k}\cC^a_2 = \left\{\forall q, \forall a: X^a_q >= 1 \right\}
\end{equation}
Let $p_1$ be the proportion of agents with type $j>\kappa$ and $p_2$ be the proportion of agents with type $i<\kappa$. If Algorithm~\ref{alg:racing-many-types-two-phases} is BIC for all agents of types $i<\kappa$, then for each arm $a$ we have $X^a_q \sim Binom(h, p_2)$. 

Hence, we have
\begin{equation}
    \Prob[X^a_q \geq 1] = 1-(1 - p_2)^h,
\end{equation}
and
\begin{equation}
    \Prob[\forall a, \ X^a_q \geq 1] = \left(1-(1 - p_2)^h\right)^m = \delta'
\end{equation}
\ls{Double check this. Don't think it's right.}

Let $\tau \in (0, 1)$. Fix phase $q \geq \ell_1$, and some agent $t$ in this phase. In order to prove that Algorithm~\ref{alg:racing-many-types-two-phases} is BIC for agents of types $i<\kappa$, we want to show that for any type $i<\kappa$ and arm $a$
\begin{equation}
    \label{eq:racing-bic-arm2}
    \E_{\cP_i}[G\vert z_t=\e_a, u_t=i]\Prob_{\cP_i}[z_t=\e_a, u_t=i] \geq 0.
\end{equation}
From Corollary ~\eqref{cor:finite-sample}, with probability $\delta$ we have that
\begin{equation*}
    \Prob[\neg \cC_1 \vert G] \leq \delta
\end{equation*} 
Define event $\cC$ such that
\begin{equation}
\label{eq:event-C}
    \cC := \left\{ \forall q \geq \ell_1: \cC_1 \  \& \ \cC_2 \right\}
\end{equation}
Using union bound, we have
\begin{align}
    \Prob[\neg \cC \vert G] &\leq \Prob[\neg \cC_1 \vert G] + \Prob[\neg \cC_2 \vert G]\\
    &\leq \delta + \delta' 
\end{align}
Therefore, since $G\geq -1$, we have: 
\begin{align*}
\label{eq:racing-bic}
    \E_{\cP_i}[G|z_t=\e_a]\Prob_{\cP_i}[z_t=\e_a]
    &= \E_{\cP_i}[G|z_t=\e_a, \cC]\Prob_{\cP_i}[z_t=\e_a, \cC] + \E_{\cP_i}[G|z_t=\e_a, \neg C]\Prob_{\cP_i}[z_t=\e_a, \neg C]\\
    &\geq \E_{\cP_i}[G|z_t=\e_a, \cC]\Prob_{\cP_i}[z_t=\e_a, \cC] - (\delta + \delta')
\end{align*}
We want to upper bound the first term. This can be done by splitting it into four cases based on the value of $G$. We have:

\begin{equation} 
    \begin{split}
    &\quad\E_{\cP_i}[G | z_t = \e_2, \cC]\Prob_{\cP_i}[z_t = \e_2, \cC] \\
    &= 
    \E_{\cP_i}[G | z_t = \e_2, \cC, G \geq \tau]\Prob_{\cP_i}[z_t= \e_2, \cC, G \geq \tau] \\
    &\ + \E_{\cP_i}[G | z_t = \e_2, \cC, 0 \leq G < \tau]\Prob_{\cP_i}[z_t = \e_2, \cC, 0 \leq G < \tau] \\
    &\ + \E_{\cP_i}[G | z_t = \e_2, \cC, -2s_q < G < 0]\Prob_{\cP_i}[z_t = \e_2, \cC, -2s_q < G < 0] \\
    &\ + \E_{\cP_i}[G | z_t = \e_2, \cC, G \leq -2s_q]\Prob_{\cP_i}[z_t = \e_2, \cC, G \leq -2s_q] \label{eq:racing-bic-cases}
    \end{split}
\end{equation}

%\frac{12\sqrt{\log(2T/\delta) + (m+1)\log(2n(m+\Upsilon^2))}}{\left(\sigma_{\min}\{\hat{\Gamma}\}\right)^2 \sqrt{q}}

Observe that, by definition of $s_q$, we have:
\begin{align*}
    2s_q &\leq 2s_{\ell_1}
    = \frac{24\sqrt{\log(2T/\delta) + 3\log(2n(2+\Upsilon^2))} \ \left(\sigma_{\min}\{\hat{\Gamma}\}\right)^2 \tau \Prob_{\cP_i}[G \geq \tau] }{48\sqrt{(\log(2T/\delta) + 3\log(2n(2+\Upsilon^2)))} \ \left(\sigma_{\min}\{\hat{\Gamma}\}\right)^2}\\
    &= \frac{\tau \Prob_{\cP_i}[G \geq \tau]}{2}\\
    &\leq \tau
\end{align*}

Conditional on $\cC$, the empirical estimate $\hat{G}_q > G - s_q \geq 2s_q$. Hence, when we have $G \geq \tau \geq 2s_q$, then $G=\theta^2 - \theta^1 \geq 2s_q$ and arm 1 must have already been eliminated at phase $q \geq \ell_1$. This implies that the probability $\Prob_{\cP_i}[z_t=\e_a, \cC, G\geq \tau] = \Prob_{\cP_i}[\cC, G\geq \tau]$. Similarly, when we have $G \leq -2s_q$, then $\theta^a - \theta^1 \leq -2s_q$ and arm $a$ must have already been eliminated at phase $q \geq \ell_1$. Hence, arm $a$ could not be recommended in that case and the probability $\Prob_{\cP_i}[z_t=\e_a, \cC, G\leq-2s_q] = 0$.\\
We can then rewrite equation~\eqref{eq:racing-bic-cases} as
\begin{align*}
    \E_{\cP_i}[G | z_t=\e_a, \cC]\Prob_{\cP_i}[z_t = \e_2 ,\cC] &\geq\E_{\cP_i}[G | z_t=\e_a, \cC, G \geq \tau]\Prob_{\cP_i}[z_t= \e_2, \cC, G \geq \tau]\\
    &+ \E_{\cP_i}[G | z_t=\e_a, \cC, 0 \leq G < \tau]\Prob_{\cP_i}[z_t=\e_a, \cC, 0 \leq G < \tau]\\
    &+ \E_{\cP_i}[G | z_t=\e_a, \cC, -2s_q < G < 0]\Prob_{\cP_i}[z_t=\e_a, \cC, -2s_q < G < 0]\\
    &\geq\tau \Prob_{\cP_i}[\cC, G \geq \tau] + 0\cdot \Prob_{\cP_i}[\cC, 0 \leq G < \tau] -2s_q \Prob_{\cP_i}[z_t=\e_a, \cC, -2s_q<G<0]\\
    &\geq\tau \Prob_{\cP_i}[\cC, G \geq \tau] - 2s_q\\
    &\geq\tau \Prob_{\cP_i}[\cC, G \geq \tau] - \frac{\tau \Prob_{\cP_i}[G \geq \tau]}{2}\\
    &\geq\tau \Prob_{\cP_i}[\cC | G \geq \tau] \Prob_{\cP_i}[G \geq \tau] - \frac{\tau \Prob_{\cP_i}[G \geq \tau]}{2}\\
    &\geq\tau (1 - (\delta + \delta')) \Prob_{\cP_i}[G \geq \tau] - \frac{\tau \Prob_{\cP_i}[G \geq \tau]}{2}\\
    &= \left(\frac{1}{2} - (\delta + \delta') \right) \tau \Prob_{\cP_i}[G \geq \tau]\\
    &\geq \left(\frac{1}{2} - (\delta_\tau + \delta') \right) \tau \Prob_{\cP_i}[G \geq \tau]\\
    &= \left(\frac{1}{2} - \frac{\frac{1}{2} \tau \Prob_{\cP_i}[G \geq \tau]}{\tau \Prob_{\cP_i}[G \geq \tau] + 1} \right) \tau \Prob_{\cP_i}[G \geq \tau]\\
    &= \frac{1}{2} \left(\frac{\tau \Prob_{\cP_i}[G\geq \tau] + 1 - \tau \Prob_{\cP_i}[G\geq \tau]}{\tau \Prob_{\cP_i}[G\geq \tau] + 1} \right)\tau \Prob_{\cP_i}[G\geq \tau]\\
    &= \frac{1}{2} \left(\frac{\tau \Prob_{\cP_i}[G\geq \tau]}{\tau \Prob_{\cP_i}[G\geq \tau] + 1} \right)\\
    &= \ \delta_\tau + \delta'\\
    &\geq \ \delta + \delta'.
\end{align*}
Hence, we have 
\begin{align*}
    \E_{\cP_i}[G|z_t = \e_2]\Prob_{\cP_i}[z_t = \e_2] &\geq \E[G|z_t = \e_2, \cC]\Prob_{\cP_i}[z_t = \e_2, \cC] - (\delta + \delta')\\
    &\geq \delta + \delta' -  (\delta + \delta')\\
    &= 0
\end{align*}

Hence, when we have $G_a \geq \tau \geq 2s_q$, then all other arms except arm $a$ must have already been eliminated at phase $q \geq \ell_1$, since conditional on $\cC$, $\hat{G}_q^{ab} > G_{ab} - s_q \geq G_a - s_q  \geq  s_q$. Similarly, when we have $G_a \leq -2s_t$, then arm $i$ must have already been eliminated at phase $q \geq \ell_1$ since
\begin{align*}
    \theta_q^i - \theta_q^* = \min_{j \neq i} G_n^{ab} < \min_{j \neq i} G_{ab} + s_q = G_a + s_q \leq -s_q
\end{align*}
Hence, arm $a$ could not be recommended in that case. We can then rewrite~\eqref{eq:multi-arm-racing-bic-cases} as

\begin{align*}
    \E_{\cP_i}[G_a | z_t=e_a, \cC]\Prob_{\cP_i}[z_t=e_a ,\cC] &\geq\E_{\cP_i}[G_a | z_t=e_a, \cC, G_a \geq \tau]\Prob_{\cP_i}[z_t= e_i, \cC, G_a \geq \tau] +\\
    &\E_{\cP_i}[G_a | z_t=e_a, \cC, 0 \leq G_a < \tau]\Prob_{\cP_i}[z_t=e_a, \cC, 0 \leq G_a < \tau] +\\
    &\E_{\cP_i}[G_a | z_t=e_a, \cC, -2s_q < G_a < 0]\Prob_{\cP_i}[z_t=e_a, \cC, -2s_q < G_a < 0]\\
    &\geq\tau \Prob_{\cP_i}[\cC, G_a \geq \tau] + 0 \Prob_{\cP_i}[\cC, 0 \leq G_a < \tau] -2s_q \Prob_{\cP_i}[\cC, G_a \leq -2s_q]\\
    &=\tau \Prob_{\cP_i}[\cC, G_a \geq \tau] - 2s_q\Prob_{\cP_i}[\cC, G_a \geq -2s_q]\\
    &\geq\tau \Prob_{\cP_i}[\cC, G_a \geq \tau] - 2s_q\\
    &\geq\tau \Prob_{\cP_i}[\cC, G_a \geq \tau] - \frac{\tau \Prob_{\cP_i}[G_a \geq \tau]}{2}\\
    &\geq\tau \Prob_{\cP_i}[\cC | G_a \geq \tau] \Prob_{\cP_i}[G_a \geq \tau] - \frac{\tau \Prob_{\cP_i}[G_a \geq \tau]}{2}\\
    &\geq\tau (1 - (\delta + \delta')) \Prob_{\cP_i}[G_a \geq \tau] - \frac{\tau \Prob_{\cP_i}[G_a \geq \tau]}{2}\\
    &= \left(\frac{1}{2} - (\delta + \delta') \right) \tau \Prob_{\cP_i}[G_a \geq \tau]\\
    &\geq \left(\frac{1}{2} - (\delta_\tau + \delta') \right) \tau \Prob_{\cP_i}[G_a \geq \tau]\\
    &= \left(\frac{1}{2} - \frac{\frac{1}{2} \tau \Prob_{\cP_i}[G_a \geq \tau]}{\tau \Prob_{\cP_i}[G_a \geq \tau] + 1} \right) \tau \Prob_{\cP_i}[G_a \geq \tau]\\
    &= \frac{\frac{1}{2} \tau^2 (\Prob_{\cP_i}[G_a \geq \tau])^2 + \frac{1}{2} \tau \Prob_{\cP_i}[G_a \geq \tau] - \frac{1}{2} \tau^2 (\Prob_{\cP_i}[G_a \geq \tau])^2}{\tau \Prob_{\cP_i}[G_a \geq \tau] + 1}\\
    &= \frac{\frac{1}{2} \tau \Prob_{\cP_i}[G_a \geq \tau]}{\tau \Prob_{\cP_i}[G_a \geq \tau] + 1}\\
    &= \delta_\tau + \delta'\\
    &\geq \delta + \delta'
\end{align*}
Hence, we have 
\begin{align*}
    \E_{\cP_i}[G_a|z_t=e_a]\Prob_{\cP_i}[z_t=e_a] &\geq \E_{\cP_i}[G_a|z_t=e_a, \cC]\Prob_{\cP_i}[z_t=e_a, \cC] - (\delta + \delta')\\
    &\geq \delta + \delta' - (\delta + \delta')\\
    &= 0
\end{align*}

Therefore, Algorithm~\ref{alg:racing-many-types-two-phases} fulfills equation~\eqref{eq:racing-bic-arm2} and is BIC for agents of types $i<\kappa$.
\end{proof}

During the first racing stage, we collect more samples of arm 2 through agents of type 2. After getting sufficient samples of arm 2, we can also convince agents of type 1 to follow our recommendation for arm 2. The following Lemma $\ref{lemma:racing-bic-many-types-2nd-group}$, which follow the same structure as that of Lemma $\ref{lemma:racing-bic-many-types-1st-group}$, proves the second racing stage algorithm is BIC for both agents of type 1 and type 2.

%%%%%%%%%%%%%%%%%%%%%%%%%%%%%%%%%%%%%%%%%%%%%%%%%%%%%%%%%
%%%%%%%%%%%%%%%%%%%%%%%% 2nd Part %%%%%%%%%%%%%%%%%%%%%%%
%%%%%%%%%%%%%%%%%%%%%%%%%%%%%%%%%%%%%%%%%%%%%%%%%%%%%%%%%

Lemma~\ref{lemma:racing-bic-many-types-2nd-group}
\bicracingmanytypessecond*

\begin{proof}
We want to show that for any agent $t$ with a type $i<\kappa$ in the racing stage and for any two arms $a,b \in B:$
\begin{align*}
    \E_{\cP_j}[\theta^a - \theta^b | z_t=e_a]\Prob_{\cP_j}[z_t=e_a] \geq 0
\end{align*}
We will prove a stronger statement:
\begin{align*}
    \E_{\cP_j}[\theta^a - \max_{b \neq a} \theta^b| z_t=e_a]\Prob_{\cP_j}[z_t=e_a] \geq 0
\end{align*}
For each pair of arms $a,b \in B$, denote $G_{ab} = \theta^a - \theta^b$ and 
\begin{align*}
    G_a = \theta^a - \max_{b \neq a} \theta^b = \min_{b \neq a} G_{ab}.
\end{align*}

 Let 
\[s_q := \frac{12\sqrt{\log(2T/\delta) + (m+1)\log(2n(m+\Upsilon^2))}}{\left(\sigma_{\min}\{\hat{\Gamma}\}\right)^2 \sqrt{q}}\] be the decision threshold for each phase $q \geq \ell_1$ in Algorithm~\ref{alg:racing-many-types-two-phases}. Assume that after elimination, at every iteration a sample of the eliminated arm is also drawn, but not revealed to the agent.\\
We define the event $\cC$ as the accuracy guarantee of $\hat{\theta}$ such that:
\begin{equation}
\label{eq:event-C}
    \cC := \left\{ \forall q \geq \ell_1: |G - \hat{G}_n| < s_q \right\}
\end{equation}
where $\ell_1$ is the number of samples of each arm after running the sampling stage.\\
Let $p_1$ be the proportion of agents with type $j>\kappa$ and $p_2$ be the proportion of agents with type $i<\kappa$.

Let $\tau \in (0, 1)$. Fix phase $q \geq \ell_1$, and some agent $t$ in this phase. In order to prove that Algorithm~\ref{alg:racing-many-types-two-phases} is BIC for agents of types $i<\kappa$, we want to show that for any type $i<\kappa$ and arm $a$
\begin{equation}
    \label{eq:racing-bic-arm2}
    \E_{\cP_j}[G\vert z_t=\e_a, u_t=i]\Prob_{\cP_j}[z_t=\e_a, u_t=i] \geq 0.
\end{equation}
From Corollary ~\eqref{cor:finite-sample}, with probability $\delta$ we have that
\begin{equation*}
    \Prob[\neg \cC \vert G] \leq \delta
\end{equation*} 

Using union bound, we have
\begin{align}
    \Prob[\neg \cC \vert G] &\leq \Prob[\neg \cC_1 \vert G] + \Prob[\neg \cC_2 \vert G]\\
    &\leq \delta + \delta' 
\end{align}
Therefore, since $G\geq -1$, we have: 
\begin{align*}
\label{eq:racing-bic}
    \E_{\cP_j}[G|z_t=\e_a]\Prob_{\cP_j}[z_t=\e_a]
    &= \E_{\cP_j}[G|z_t=\e_a, \cC]\Prob_{\cP_j}[z_t=\e_a, \cC] + \E_{\cP_j}[G|z_t=\e_a, \neg C]\Prob_{\cP_j}[z_t=\e_a, \neg C]\\
    &\geq \E_{\cP_j}[G|z_t=\e_a, \cC]\Prob_{\cP_j}[z_t=\e_a, \cC] - (\delta + \delta')
\end{align*}
We want to upper bound the first term. This can be done by splitting it into four cases based on the value of $G$. We have:

\begin{equation} 
    \begin{split}
    \E_{\cP_j}[G | z_t = \e_2, \cC]\Prob_{\cP_j}[z_t = \e_2, \cC] = 
    &\E_{\cP_j}[G | z_t = \e_2, \cC, G \geq \tau]\Prob_{\cP_j}[z_t= \e_2, \cC, G \geq \tau] \\
    &\ + \E_{\cP_j}[G | z_t = \e_2, \cC, 0 \leq G < \tau]\Prob_{\cP_j}[z_t = \e_2, \cC, 0 \leq G < \tau] \\
    &\ + \E_{\cP_j}[G | z_t = \e_2, \cC, -2s_q < G < 0]\Prob_{\cP_j}[z_t = \e_2, \cC, -2s_q < G < 0] \\
    &\ + \E_{\cP_j}[G | z_t = \e_2, \cC, G \leq -2s_q]\Prob_{\cP_j}[z_t = \e_2, \cC, G \leq -2s_q] \label{eq:racing-bic-cases}
    \end{split}
\end{equation}

Observe that, by definition of $s_q$, we have:
\begin{align*}
    2s_q &\leq 2s_{\ell_1}
    = \frac{24\sqrt{\log(2T/\delta) + 3\log(2n(2+\Upsilon^2))} \ \left(\sigma_{\min}\{\hat{\Gamma}\}\right)^2 \tau \Prob_{\cP_j}[G \geq \tau] }{48\sqrt{(\log(2T/\delta) + 3\log(2n(2+\Upsilon^2)))} \ \left(\sigma_{\min}\{\hat{\Gamma}\}\right)^2}\\
    &= \frac{\tau \Prob_{\cP_j}[G \geq \tau]}{2}\\
    &\leq \tau
\end{align*}

Conditional on $\cC$, the empirical estimate $\hat{G}_q > G - s_q \geq 2s_q$. Hence, when we have $G \geq \tau \geq 2s_q$, then $G=\theta^2 - \theta^1 \geq 2s_q$ and arm 1 must have already been eliminated at phase $q \geq \ell_1$. This implies that the probability $\Prob_{\cP_i}[z_t=\e_a, \cC, G\geq \tau] = \Prob_{\cP_i}[\cC, G\geq \tau]$. Similarly, when we have $G \leq -2s_q$, then $\theta^2 - \theta^1 \leq -2s_q$ and arm 2 must have already been eliminated at phase $q \geq \ell_1$. Hence, arm 2 could not be recommended in that case and the probability $\Prob_{\cP_i}[z_t=\e_a, \cC, G\leq-2s_q] = 0$.\\
We can then rewrite equation~\eqref{eq:racing-bic-cases} as
\begin{align*}
    \E_{\cP_i}[G | z_t=\e_a, \cC]\Prob_{\cP_i}[z_t = \e_2 ,\cC] &\geq\E_{\cP_i}[G | z_t=\e_a, \cC, G \geq \tau]\Prob_{\cP_i}[z_t= \e_2, \cC, G \geq \tau]\\
    &+ \E_{\cP_i}[G | z_t=\e_a, \cC, 0 \leq G < \tau]\Prob_{\cP_i}[z_t=\e_a, \cC, 0 \leq G < \tau]\\
    &+ \E_{\cP_i}[G | z_t=\e_a, \cC, -2s_q < G < 0]\Prob_{\cP_i}[z_t=\e_a, \cC, -2s_q < G < 0]\\
    &\geq\tau \Prob_{\cP_i}[\cC, G \geq \tau] + 0\cdot \Prob_{\cP_i}[\cC, 0 \leq G < \tau] -2s_q \Prob_{\cP_i}[z_t=\e_a, \cC, -2s_q<G<0]\\
    &\geq\tau \Prob_{\cP_i}[\cC, G \geq \tau] - 2s_q\\
    &\geq\tau \Prob_{\cP_i}[\cC, G \geq \tau] - \frac{\tau \Prob_{\cP_i}[G \geq \tau]}{2}\\
    &\geq\tau \Prob_{\cP_i}[\cC | G \geq \tau] \Prob_{\cP_i}[G \geq \tau] - \frac{\tau \Prob_{\cP_i}[G \geq \tau]}{2}\\
    &\geq\tau (1 - (\delta + \delta')) \Prob_{\cP_i}[G \geq \tau] - \frac{\tau \Prob_{\cP_i}[G \geq \tau]}{2}\\
    &= \left(\frac{1}{2} - (\delta + \delta') \right) \tau \Prob_{\cP_i}[G \geq \tau]\\
    &\geq \left(\frac{1}{2} - (\delta_\tau + \delta') \right) \tau \Prob_{\cP_i}[G \geq \tau]\\
    &= \left(\frac{1}{2} - \frac{\frac{1}{2} \tau \Prob_{\cP_i}[G \geq \tau]}{\tau \Prob_{\cP_i}[G \geq \tau] + 1} \right) \tau \Prob_{\cP_i}[G \geq \tau]\\
    &= \frac{1}{2} \left(\frac{\tau \Prob_{\cP_i}[G\geq \tau] + 1 - \tau \Prob_{\cP_i}[G\geq \tau]}{\tau \Prob_{\cP_i}[G\geq \tau] + 1} \right)\tau \Prob_{\cP_i}[G\geq \tau]\\
    &= \frac{1}{2} \left(\frac{\tau \Prob_{\cP_i}[G\geq \tau]}{\tau \Prob_{\cP_i}[G\geq \tau] + 1} \right)\\
    &= \ \delta_\tau + \delta'\\
    &\geq \ \delta + \delta'.
\end{align*}
Hence, we have 
\begin{align*}
    \E_{\cP_i}[G|z_t = \e_2]\Prob_{\cP_i}[z_t = \e_2] &\geq \E[G|z_t = \e_2, \cC]\Prob_{\cP_i}[z_t = \e_2, \cC] - (\delta + \delta')\\
    &\geq \delta + \delta' -  (\delta + \delta')\\
    &= 0
\end{align*}

Hence, when we have $G_a \geq \tau \geq 2s_q$, then all other arms except arm $a$ must have already been eliminated at phase $q \geq \ell_1$, since conditional on $\cC$, $\hat{G}_q^{ab} > G_{ab} - s_q \geq G_a - s_q  \geq  s_q$. Similarly, when we have $G_a \leq -2s_t$, then arm $i$ must have already been eliminated at phase $q \geq \ell_1$ since
\begin{align*}
    \theta_q^i - \theta_q^* = \min_{j \neq i} G_n^{ab} < \min_{j \neq i} G_{ab} + s_q = G_a + s_q \leq -s_q
\end{align*}
Hence, arm $a$ could not be recommended in that case. We can then rewrite~\eqref{eq:multi-arm-racing-bic-cases} as

\begin{align*}
    \E_{\cP_j}[G_a | z_t=e_a, \cC]\Prob_{\cP_j}[z_t=e_a ,\cC] &\geq\E_{\cP_j}[G_a | z_t=e_a, \cC, G_a \geq \tau]\Prob_{\cP_j}[z_t= e_i, \cC, G_a \geq \tau] +\\
    &\E_{\cP_j}[G_a | z_t=e_a, \cC, 0 \leq G_a < \tau]\Prob_{\cP_j}[z_t=e_a, \cC, 0 \leq G_a < \tau] +\\
    &\E_{\cP_j}[G_a | z_t=e_a, \cC, -2s_q < G_a < 0]\Prob_{\cP_j}[z_t=e_a, \cC, -2s_q < G_a < 0]\\
    &\geq\tau \Prob_{\cP_j}[\cC, G_a \geq \tau] + 0 \Prob_{\cP_j}[\cC, 0 \leq G_a < \tau] -2s_q \Prob_{\cP_j}[\cC, G_a \leq -2s_q]\\
    &=\tau \Prob_{\cP_j}[\cC, G_a \geq \tau] - 2s_q\Prob_{\cP_j}[\cC, G_a \geq -2s_q]\\
    &\geq\tau \Prob_{\cP_j}[\cC, G_a \geq \tau] - 2s_q\\
    &\geq\tau \Prob_{\cP_j}[\cC, G_a \geq \tau] - \frac{\tau \Prob_{\cP_j}[G_a \geq \tau]}{2}\\
    &\geq\tau \Prob_{\cP_j}[\cC | G_a \geq \tau] \Prob_{\cP_j}[G_a \geq \tau] - \frac{\tau \Prob_{\cP_j}[G_a \geq \tau]}{2}\\
    &\geq\tau (1 - (\delta + \delta')) \Prob_{\cP_j}[G_a \geq \tau] - \frac{\tau \Prob_{\cP_j}[G_a \geq \tau]}{2}\\
    &= \left(\frac{1}{2} - (\delta + \delta') \right) \tau \Prob_{\cP_j}[G_a \geq \tau]\\
    &\geq \left(\frac{1}{2} - (\delta_\tau + \delta') \right) \tau \Prob_{\cP_j}[G_a \geq \tau]\\
    &= \left(\frac{1}{2} - \frac{\frac{1}{2} \tau \Prob_{\cP_j}[G_a \geq \tau]}{\tau \Prob_{\cP_j}[G_a \geq \tau] + 1} \right) \tau \Prob_{\cP_j}[G_a \geq \tau]\\
    &= \frac{\frac{1}{2} \tau^2 (\Prob_{\cP_j}[G_a \geq \tau])^2 + \frac{1}{2} \tau \Prob_{\cP_j}[G_a \geq \tau] - \frac{1}{2} \tau^2 (\Prob_{\cP_j}[G_a \geq \tau])^2}{\tau \Prob_{\cP_j}[G_a \geq \tau] + 1}\\
    &= \frac{\frac{1}{2} \tau \Prob_{\cP_j}[G_a \geq \tau]}{\tau \Prob_{\cP_j}[G_a \geq \tau] + 1}\\
    &= \delta_\tau + \delta'\\
    &\geq \delta + \delta'
\end{align*}
Hence, we have 
\begin{align*}
    \E_{\cP_j}[G_a|z_t=e_a]\Prob_{\cP_j}[z_t=e_a] &\geq \E_{\cP_j}[G_a|z_t=e_a, \cC]\Prob_{\cP_j}[z_t=e_a, \cC] - (\delta + \delta')\\
    &\geq \delta + \delta' - (\delta + \delta')\\
    &= 0
\end{align*}

Therefore, Algorithm~\ref{alg:racing-two-types} fulfills equation~\eqref{eq:racing-bic-arm2} and is BIC for agents of types $i<\kappa$.
\end{proof}
