# Supplementary material for: Incentivizing Compliance with Algorithmic Instruments
Source: arXiv:2107.10093 source file (2021-07-28)
Supplement: Supplementary file 6 [file appendix-two-arms-general.tex]

\newpage
\section{Omitted Proofs for two arms two types generalization}
\bicsamplingtwoarmsgeneral*
Recall that for type $i$, the event:
\begin{equation}
    \xi_i = \left\{ \frac{1}{L_2}\sum_{t = 1}^{L_2} y^1_t + \frac{1}{2} + \nu + \Upsilon + \sigma_\epsilon \sqrt{\frac{2\log(1/\delta)}{L_2}} < \mu^2_i \right\},
\end{equation}
with probability at least $1-\delta$ for confidence $\delta > 0$.
\begin{proof} Let $\displaystyle G_{L_2} := \E_{\cP_i}[\theta^2 - \theta^1|S_{1, L_2}]$. It is sufficient to show that $\displaystyle \E_{\cP_i}[G_{L_2}|z_t = \e_2]\Prob_{\cP_i}[z_t = \e_2] \geq 0$ (by \cref{claim:bic-equiv}).
\begin{claim}
\label{claim:bic-equiv}
Assume that we have $\displaystyle \E_{\cP_i}[\theta^2 - \theta^1|z_t = \e_2]\Prob_{\cP_i}[z_t = \e_2] \geq 0$. Then we also have $\displaystyle \E_{\cP_i}[\theta^1 - \theta^2|z_t = \e_1]\Prob_{\cP_i}[z_t = \e_1] \geq 0$.
\end{claim}
\begin{proof}
Algorithm~\ref{alg:sampling-two-types-general} is designed in a way such that we always have $\Prob_{\cP_i}[z_t = \e_2] > 0$.\\
Similarly, assume that we also recommend arm 1 with some positive probability: $\Prob_{\cP_i}[z_t = \e_1] > 0$. Assume that the expected difference in mean rewards $\displaystyle \E_{\cP_i}[\theta^2 - \theta^1]\leq 0$. Then, we have:
\begin{align*}
    0 &\geq \E_{\cP_i}[\theta^2 - \theta^1] \\
    &= \E_{\cP_i}[\theta^2 - \theta^1|z_t = \e_2]\Prob_{\cP_i}[z_t = \e_2] + \E_{\cP_i}[\theta^2 - \theta^1|z_t = \e_1]\Prob_{\cP_i}[z_t = \e_1]
\end{align*}
Since, by assumption, the product $\displaystyle \E_{\cP_i}[\theta^2 - \theta^1|z_t = \e_2]\Prob[z_t=\e_2] \geq 0$, it must be that the product 
\[\E_{\cP_i}[\theta^2 - \theta^1|z_t = \e_1]\Prob_{\cP_i}[z_t = \e_1] \leq 0.\] 
Reversing the order of operands, we have that
$\E_{\cP_i}[\theta^1 - \theta^2|z_t = \e_1]\Prob_{\cP_i}[z_t = \e_1] \geq 0.$
\end{proof}
Note that we have 
\begin{align*}
&\quad	\E_{\cP_i}[G_{L_2} | z_t = \e_2] \Prob_{\cP_i}[z_t = \e_2] \\
	&= \E_{\cP_i}[G_{L_2} |z_t = \e_2 \ \& \ p_t \in P-Q]\Prob_{\cP_i}[z_t = \e_2 \ \& \ p_t \in P-Q] \\
	& \hspace{.4cm} + \E_{\cP_i}[G_{L_2}|z_t = \e_2 \ \& \ p_t \in Q]\Prob_{\cP_i}[z_t = \e_2 \ \& \ p_t \in Q]\\
	&= \E_{\cP_i}[G_{L_2} | \xi_2]\Prob_{\cP_i}[\xi_i]\left(1 - \frac{1}{\rho} \right) + \E_{\cP_i}[G_{L_2}|z_t = \e_2 \ \& \ p_t \in Q]\Prob_{\cP_i}[z_t = \e_2 \ \& \ p_t \in Q]\\
	&= \E_{\cP_i}[G_{L_2} | \xi_i]\Prob_{\cP_i}[\xi_i]\left(1 - \frac{1}{\rho} \right) + \E_{\cP_i}[G_{L_2}|p_t\in Q]\Prob_{\cP_i}[p_t \in Q], \ \ \text{(by definition $p_t\in Q \Rightarrow z_t=\e_2$)}\\
	&= \E_{\cP_i}[G_{L_2} | \xi_i]\Prob_{\cP_i}[\xi_i]\left(1 - \frac{1}{\rho} \right) + \E_{\cP_i}[\theta^2 - \theta^1 | p_t\in Q]\Prob_{\cP_i}[p_t \in Q] \ \ \text{(by Law of Total Expectation)}\\
	&= \E_{\cP_i}[G_{L_2} | \xi_i]\Prob_{\cP_i}[\xi_i]\left(1 - \frac{1}{\rho} \right) + \E_{\cP_i}[\theta^2 - \theta^1]\Prob_{\cP_i}[p_t \in Q] \\
	&= \E_{\cP_i}[G_{L_2} | \xi_i]\Prob_{\cP_i}[\xi_i]\left(1 - \frac{1}{\rho} \right) + (\mu_i^2 - \mu_i^1)\Prob_{\cP_i}[p_t \in Q]\\
	&= \E_{\cP_i}[G_{L_2} | \xi_i]\Prob_{\cP_i}[\xi_i]\left(1 - \frac{1}{\rho} \right) + \frac{1}{\rho}(\mu_i^2 - \mu_i^1)
\end{align*}
For agents of type $i$ to follow our recommendation for arm 2, we need to pick $\rho$:
\begin{align}
    \E_{\cP_i}[G_{L_2} | z_t = \e_2] \Prob_{\cP_i}[z_t = \e_2] &\geq \phi(u_t) \nonumber\\
	\E_{\cP_i}[G_{L_2} | \xi_i]\Prob_{\cP_i}[\xi_i]\left(1 - \frac{1}{\rho} \right) + \frac{1}{\rho}(\mu_i^2 - \mu_i^1) &\geq \phi(u_t)\Prob_{\cP_i}[\xi_i] \nonumber\\
	\E_{\cP_i}[G_{L_2} | \xi_i]\Prob_{\cP_i}[\xi_i] - \frac{1}{\rho}\E_{\cP_i}[G_{L_2}|\xi_i] \Prob_{\cP_i}[\xi_i] + \frac{1}{\rho}(\mu_i^2 - \mu_i^1) &\geq \phi(u_t)\Prob_{\cP_i}[\xi_i] \nonumber\\
	\rho\E_{\cP_i}[G_{L_2}|\xi_i]\Prob_{\cP_i}[\xi_i] - \rho \phi(u_t)\Prob_{\cP_i}[\xi_i] &\geq \E_{\cP_i}[G_{L_2} | \xi_i]\Prob_{\cP_i}[\xi_i] - (\mu_i^2 - \mu_i^1) \nonumber\\
	\rho &\geq 1 + \frac{\mu_i^1 - \mu_i^2 + \phi(u_t)\Prob_{\cP_i}[\xi_i]}{\E_{\cP_i}[G_{L_2} | \xi_i]\Prob_{\cP_i}[\xi_i] - \phi(u_t)\Prob_{\cP_i}[\xi_i]} \nonumber\\
	\rho &\geq 1 + \frac{\mu_i^1 - \mu_i^2 + \nu\Prob_{\cP_i}[\xi_i]}{\E_{\cP_i}[G_{L_2} | \xi_i]\Prob_{\cP_i}[\xi_i] - \nu\Prob_{\cP_i}[\xi_i]} \nonumber
	\label{eq:L-condition}
\end{align}

This comes down to finding a lower bound on the denominator of the expression above. First, we define a clean event $C'$ where the average error $\frac{1}{L_2}\sum_{i=1}^{L_2} \epsilon_i$ is bounded (following Corollary \ref{thm:high-prob-unbounded-chernoff}):
\begin{equation}
     C' := \left \{ \bigg\vert\frac{1}{L_2} \sum_{i=1}^{L_2} \epsilon_i \bigg\vert \leq \sigma_\epsilon \sqrt{\frac{2\log(1/\delta)}{L_2}} \right \}.
\end{equation}
The event $C'$ occurs with probability at least $1 - \delta$ for $\displaystyle \delta < \delta' := \frac{\Prob_{\cP_i}[\xi_i]}{8}$.

We have 
\begin{align}
    \E_{\cP_i}[G_{L_2} | \xi_i] \Prob_{\cP_i}[\xi_i] &= \E_{\cP_i}[G_{L_2} | \xi_i, C'] \Prob_{\cP_i}[\xi_i, C'] + \E_{\cP_i}[G_{L_2} | \xi_i, \neg C'] \Prob_{\cP_i}[\xi_i, \neg C'] \nonumber\\
    &\geq \E_{\cP_i}[G_{L_2} | \xi_i, C'] \Prob_{\cP_i}[\xi_i, C'] - \delta \tag{since $G_{L_2} \geq -1$ and $\Prob_{\cP_i}[\neg C']<\delta$} \nonumber\\
    &= \E_{\cP_i}[G_{L_2} | \xi_i, C'] (\Prob_{\cP_i}[\xi_i] - \Prob_{\cP_i}[\xi_i, \neg C']) - \delta \nonumber\\
    &\geq \E_{\cP_i}[G_{L_2} | \xi_i, C'] (\Prob_{\cP_i}[\xi_i] - \Prob_{\cP_i}[\neg C']) - \delta \nonumber\\
    &\geq \E_{\cP_i}[G_{L_2} | \xi_i, C'] (\Prob_{\cP_i}[\xi_i] - \delta) - \delta \nonumber\\
    &= \E_{\cP_i}[G_{L_2} | \xi_i, C'] \Prob_{\cP_i}[\xi_i] - \delta(1 + \E_{\cP_i}[G_{L_2} | \xi_i, C']) \nonumber\\
    &\geq \E_{\cP_i}[G_{L_2} | \xi_i, C'] \Prob_{\cP_i}[\xi_i] - 2\delta \label{eq:sampling-two-arm-clean-event}
\end{align}

This comes down to finding a lower bound on the denominator of the expression above. We can reduce the dependency of the denominator to a single prior-dependent constant $\Prob_{\cP_i}[\xi_i]$ if we lower bound the prior-dependent expected value $\E_{\cP_i}[G_{L_2} | \xi_i]$. That way, assuming we know the prior and can calculate the probability of event $\xi_i$, we can pick an appropriate $\rho$ to satisfy the BIC condition for all agents of type $i$. Remember that event $\xi_i = \{ \bar{y}^1_{L_2} + C < \mu^2_i\}$ where $C = \Upsilon + \sigma_{\epsilon}\sqrt{\frac{2\log(1/\delta)}{L_2}} + \frac{1}{2} + \nu$ and $\displaystyle G_{L_2} := \E_{\cP_i}[\theta^2 - \theta^1|S_{1, L_2}]$. Then, the expected value
\begin{align}
    \E_{\cP_i}[G_{L_2} | \xi_i, C'] 
    &= \E_{\cP_i}[\E_{\cP_i}[\theta^2 - \theta^1|S_{1, L_2}] | \xi_i, C'] \nonumber\\
    &= \mu_i^2 - \E_{\cP_i}\left[\theta^1 \middle| \Upsilon + \sigma_{\epsilon}\sqrt{\frac{2\log(1/\delta)}{L_2}} + \frac{1}{2} + \nu + \bar{y}^1_{L_2}< \mu_i^2, C'\right] \nonumber\\
    &= \mu_i^2 - \E_{\cP_i}\left[\theta^1 \middle| \Upsilon + \sigma_{\epsilon}\sqrt{\frac{2\log(1/\delta)}{L_2}} + \frac{1}{2} + \nu +  \frac{1}{L_2}\sum_{t=1}^{L_2} y_t^1< \mu_i^2, C'\right] \nonumber\\
    &= \mu_i^2 - \E_{\cP_i}\left[\theta^1 \middle| \Upsilon + \sigma_{\epsilon}\sqrt{\frac{2\log(1/\delta)}{L_2}} + \frac{1}{2}  + \frac{1}{L_2}\sum_{t=1}^{L_2} \theta^1 + g(u_t) + \epsilon_t  < \mu_i^2, C'\right] \nonumber\\
    &= \mu_i^2 - \E_{\cP_i}\left[\theta^1 \middle| \theta^1 + \Upsilon + \sigma_{\epsilon}\sqrt{\frac{2\log(1/\delta)}{L_2}} + \frac{1}{2} + \nu + \frac{1}{L_2}\sum_{t=1}^{L_2} g(u_t) + \epsilon_t  < \mu_i^2, C'\right] \nonumber\\
    &> \mu_i^2 - \E_{\cP_i}\left[\theta^1 \middle| \theta^1 + \Upsilon + \sigma_{\epsilon}\sqrt{\frac{2\log(1/\delta)}{L_2}} + \frac{1}{2} + \nu - \Upsilon - \sigma_{\epsilon}\sqrt{\frac{2\log(1/\delta)}{L_2}} < \mu_i^2\right] \tag{since $g(u_t) > -\Upsilon$ and $\frac{1}{L_2}\sum_{t=1}^{L_2}\epsilon_t > -\sigma_\epsilon \sqrt{\frac{2\log(1/\delta)}{L_2}}$ by event $C'$} \nonumber\\
    &> \mu_i^2 - \E_{\cP_i}\left[\theta^1 \middle| \theta^1 + \frac{1}{2} + \nu < \mu_i^2\right] \nonumber\\
    &> \frac{1}{2} + \nu
    \label{eq:sampling-stage-two-arm-gap}
\end{align}
Hence, the lower bound on the denominator is
\begin{align}
    \E_{\cP_i}[G_{L_2} | \xi_i] \Prob_{\cP_i}[\xi_i] - \nu\Prob_{\cP_i}[\xi_i] &\geq \E_{\cP_i}[G_{L_2} | \xi_i, C']\Prob_{\cP_i}[\xi_i] - 2\delta - \nu\Prob_{\cP_i}[\xi_i] \tag{by Equation \ref{eq:sampling-two-arm-clean-event}}\\
    &> \frac{1}{2}\Prob_{\cP_i}[\xi_i] + \nu\Prob_{\cP_i}[\xi_i] - 2\delta - \nu\Prob_{\cP_i}[\xi_i] \tag{by Equation \ref{eq:sampling-stage-two-arm-gap}}\\
    &= \frac{1}{4}\Prob_{\cP_i}[\xi_i] + \frac{1}{4}\Prob_{\cP_i}[\xi_i] - 2\delta \\ 
    &= 2\delta' + \frac{\Prob_{\cP_i}[\xi_i]}{4} - 2\delta \tag{since $\delta' = \frac{1}{8} \Prob_{\cP_i}[\xi_i]$}\\
    &\geq \frac{\Prob_{\cP_i}[\xi_i]}{4} \tag{since $\delta < \delta'$}
\end{align}
Hence, we can pick :
\begin{align*}
    \rho &\geq 1 + \frac{4(\mu_i^1 - \mu_i^2 + \nu\Prob_{\cP_i}[\xi_i])}{\Prob_{\cP_i}[\xi_i]}
\end{align*}
to satisfy the BIC condition for all agents of type $i$.
\end{proof}
 
\racingbictwotypesgeneral*
\begin{proof}
Let $\displaystyle G := \theta^2 - \theta^1$ \dn{just $\theta$?} and $\hat{G}_q := \hat{\theta}^2_q - \hat{\theta}^1_q$. Let 
\[s_q := 192\sqrt{\frac{\log(3T/\delta) + 3\log(2T(2+\Upsilon^2))}{q}}\] be the decision threshold for each phase $q \geq L_2$ in Algorithm~\ref{alg:racing-two-types-general}. Assume that after the elimination, at every iteration a sample of the eliminated arm is also drawn, but not revealed to the agent.\\
We define the event $\cC_1$ as the accuracy guarantee of $\hat{\theta}$ such that:
\begin{equation}
\label{eq:event-C-1}
    \cC_1 := \left\{ \forall q \geq L_2: |G - \hat{G}_q| < s_q \right\}
\end{equation}
where $L_2$ is the number of samples of each arm after running the sampling stage.\\
Let $X^2_q$ be the number of arm 2 samples in phase $q$. We also define event $\cC_2$ where there is at least one sample of arm 2 in each phase:
\begin{equation}
\label{eq:event-C-2}
    \cC_2 := \left\{\forall q: X^2_q \geq 1 \right\}
\end{equation}
Recall that half of the population is of type 1 and the other half is of type 2, and $h$ is the number of types a single arm is recommended during a single phase. Then, if Algorithm~\ref{alg:racing-two-types-general} is BIC for all agents of type 2, we have $X^2_q \sim B(h,1/2)$. Hence, we have
\begin{equation}
    \Prob[X^2_q \geq 1] = 1 - \left(\frac{1}{2}\right)^h = \delta'.
\end{equation}

Let $\tau \in (0, 1)$. Fix phase $q \geq L_2$, and some agent $t$ in this phase. In order to prove that Algorithm~\ref{alg:racing-two-types-general} is BIC for all agents of type 2, we want to show that 
\begin{equation}
    \label{eq:racing-bic-arm2}
    \E_{\cP_2}[G\vert z_p = \e_2]\Prob_{\cP_2}[z_p = \e_2] \geq \nu.
\end{equation}

Note that, by assumption, the parameter
\begin{align*}
    h &\geq \frac{\log\left(\frac{3\tau\Prob_{\cP_2}[G\geq\tau]+4}{4\tau\Prob_{\cP_2}[G\geq\tau]+4}\right)}{\log(1-p_2)}\\
    \Rightarrow \left(\frac{1}{2}
    \right)^h 
    &\geq \frac{3\tau\Prob_{\cP_2}[G\geq\tau]+4}{4\tau\Prob_{\cP_2}[G\geq\tau]+4}\\
    \Rightarrow \delta' = 1 - \left(\frac{1}{2}\right)^h 
    &\leq \frac{\tau\Prob_{\cP_2}[G\geq\tau]}{4\tau\Prob_{\cP_2}[G\geq\tau]+4}.
\end{align*}

From \cref{cor:finite-sample}, with probability $\delta>0$ we have that
\begin{equation*}
    \Prob[\neg \cC_1 \vert G] \leq \delta
\end{equation*} 

Define event $\cC$ such that
\begin{equation}
\label{eq:event-C}
    \cC := \left\{ \forall q \geq L_2: \cC_1 \  \& \ \cC_2 \right\}
\end{equation}

Using union bound, we have
\begin{align}
    \Prob[\neg \cC \vert G] &\leq \Prob[\neg \cC_1 \vert G] + \Prob[\neg \cC_2 \vert G]\\
    &\leq \delta + \delta' \nonumber\\
    &\leq \delta_{\tau} + \delta' \nonumber \\
    &\leq \frac{\tau\Prob_{\cP_2}[G\geq\tau]}{4\tau\Prob_{\cP_2}[G\geq\tau]+4} + \frac{\tau\Prob_{\cP_2}[G\geq\tau]}{4\tau\Prob_{\cP_2}[G\geq\tau]+4} \nonumber \\
    &= \frac{\tau\Prob_{\cP_2}[G\geq\tau]}{2\tau\Prob_{\cP_2}[G\geq\tau]+2} \label{eq:delta'}
\end{align}
Therefore, since $G\geq -1$, we have: 
\begin{align*}
\label{eq:racing-bic}
    \E_{\cP_2}[G|z_p = \e_2]\Prob_{\cP_2}[z_p = \e_2] &= \E_{\cP_2}[G|z_p = \e_2, \cC]\Prob_{\cP_2}[z_p = 2, \cC] + \E_{\cP_2}[G|z_p = \e_2, \neg C]\Prob_{\cP_2}[z_p = \e_2, \neg C]\\
    &\geq \E_{\cP_2}[G|z_p = \e_2, \cC]\Prob_{\cP_2}[z_p = \e_2, \cC] - \frac{\tau\Prob_{\cP_2}[G\geq\tau]}{2\tau\Prob_{\cP_2}[G\geq\tau]+2} 
\end{align*}
We want to upper bound the first term. This can be done by splitting it into four cases based on the value of $G$. We have:

\begin{equation} 
    \begin{split}
    &\quad\E_{\cP_2}[G | z_p = \e_2, \cC]\Prob_{\cP_2}[z_p = \e_2, \cC]\\
    &=\E_{\cP_2}[G | z_p = \e_2, \cC, G \geq \tau]\Prob_{\cP_2}[z_p= \e_2, \cC, G \geq \tau] \\
    & \hspace{0.4cm} + \E_{\cP_2}[G | z_p = \e_2, \cC, 0 \leq G < \tau]\Prob_{\cP_2}[z_p = \e_2, \cC, 0 \leq G < \tau] \\
    & \hspace{0.4cm} + \E_{\cP_2}[G | z_p = \e_2, \cC, -2s_q < G < 0]\Prob_{\cP_2}[z_p = \e_2, \cC, -2s_q < G < 0] \\
    & \hspace{0.4cm} + \E_{\cP_2}[G | z_p = \e_2, \cC, G \leq -2s_q]\Prob_{\cP_2}[z_p = \e_2, \cC, G \leq -2s_q] \label{eq:racing-bic-cases}
    \end{split}
\end{equation}

Observe that, by definition of $s_q$, we have:
\begin{align*}
    2s_q &\leq 2s_{L_2}
    = \frac{384\sqrt{\log(3T/\delta) + 3\log(2T(2+\Upsilon^2))} }{384\sqrt{\log(3T/\delta) + 3\log(2T(2+\Upsilon^2))}} \left(\frac{\tau \Prob_{\cP_2}[G \geq \tau]}{2} - \nu \right)\\
    &= \frac{\tau \Prob_{\cP_2}[G \geq \tau]}{2} - \nu \\
    &\leq \tau
\end{align*}

Conditional on $\cC$, the empirical estimate $\hat{G}_q > G - s_q \geq 2s_q$. Hence, when we have $G \geq \tau \geq 2s_q$, then $G=\theta^2 - \theta^1 \geq 2s_q$ and arm 1 must have already been eliminated at phase $q \geq L_2$. This implies that the probability $\Prob_{\cP_2}[z_p = \e_2, \cC, G\geq \tau] = \Prob_{\cP_2}[\cC, G\geq \tau]$. Similarly, when we have $G \leq -2s_q$, then $\theta^2 - \theta^1 \leq -2s_q$ and arm 2 must have already been eliminated at phase $q \geq L_2$. Hence, arm 2 could not be recommended in that case and the probability $\Prob_{\cP_2}[z_p = \e_2, \cC, G\leq-2s_q] = 0$.\\
We can then rewrite equation~\eqref{eq:racing-bic-cases} as
\begin{align*}
&\quad \E_{\cP_2}[G | z_p = \e_2, \cC]\Prob_{\cP_2}[z_p = \e_2 ,\cC]\\
&\geq \E_{\cP_2}[G | z_p = \e_2, \cC, G \geq \tau]\Prob_{\cP_2}[z_p= \e_2, \cC, G \geq \tau]\\
& \hspace{.4cm}+ \E_{\cP_2}[G | z_p = \e_2, \cC, 0 \leq G < \tau]\Prob_{\cP_2}[z_p = \e_2, \cC, 0 \leq G < \tau]\\
& \hspace{.4cm}+ \E_{\cP_2}[G | z_p = \e_2, \cC, -2s_q < G < 0]\Prob_{\cP_2}[z_p = \e_2, \cC, -2s_q < G < 0]\\
&\geq \tau \Prob_{\cP_2}[\cC, G \geq \tau] + 0\cdot \Prob_{\cP_2}[\cC, 0 \leq G < \tau] -2s_q \Prob_{\cP_2}[z_p = \e_2, \cC, -2s_q<G<0]\\
&\geq \tau \Prob_{\cP_2}[\cC, G \geq \tau] 2s_q\\
&\geq \tau \Prob_{\cP_2}[\cC, G \geq \tau] - \frac{\tau \Prob_{\cP_2}[G \geq \tau]}{2} + \nu \\
&\geq \tau \Prob_{\cP_2}[\cC | G \geq \tau] \Prob_{\cP_2}[G \geq \tau] - \left(\frac{\tau \Prob_{\cP_2}[G \geq \tau]}{2} - \nu\right) \\
&\geq \tau (1 - (\delta + \delta')) \Prob_{\cP_2}[G \geq \tau] - \frac{\tau \Prob_{\cP_2}[G \geq \tau]}{2} + \nu \\
&=  \left(\frac{1}{2} - (\delta + \delta') \right) \tau \Prob_{\cP_2}[G \geq \tau] + \nu \\
&\geq \left(\frac{1}{2} - \frac{\frac{1}{2} \tau \Prob_{\cP_2}[G \geq \tau]}{\tau \Prob_{\cP_2}[G \geq \tau] + 1} \right) \tau \Prob_{\cP_2}[G \geq \tau] \tag{by Equation~\eqref{eq:delta'}} + \nu \\
&= \frac{1}{2} \left(\frac{\tau \Prob_{\cP_2}[G\geq \tau] + 1 - \tau \Prob_{\cP_2}[G\geq \tau]}{\tau \Prob_{\cP_2}[G\geq \tau] + 1} \right)\tau \Prob_{\cP_2}[G\geq \tau] + \nu \\
&= \frac{1}{2} \left(\frac{\tau \Prob_{\cP_2}[G\geq \tau]}{\tau \Prob_{\cP_2}[G\geq \tau] + 1} \right) + \nu 
\end{align*}
Hence, we have 
\begin{align*}
    \E_{\cP_2}[G|z_p = \e_2]\Prob_{\cP_2}[z_p = \e_2] &\geq \E[G|z_p = \e_2, \cC]\Prob_{\cP_2}[z_p = \e_2, \cC] - \frac{\tau\Prob_{\cP_2}[G\geq\tau]}{2\tau\Prob_{\cP_2}[G\geq\tau]+2} \\
    &\geq \frac{\tau\Prob_{\cP_2}[G\geq\tau]}{2\tau\Prob_{\cP_2}[G\geq\tau]+2} + \nu   -  \frac{\tau\Prob_{\cP_2}[G\geq\tau]}{2\tau\Prob_{\cP_2}[G\geq\tau]+2} \\
    &= \nu
\end{align*}
Therefore, Algorithm~\ref{alg:racing-two-types-general} fulfills equation~\eqref{eq:racing-bic-arm2} and is BIC for all agents of type 2.
\end{proof}

\racingbictwotypestypeonegeneral*
\begin{proof}
After collecting more samples of arm 2 in the first part of the racing stage, we can also convince agents of type 1 to follow our recommendations for arm 2 in the second part of the racing stage.
Let $\displaystyle G := \theta^2 - \theta^1$ and $\hat{G}_q := \hat{\theta}^2_q - \hat{\theta}^1_q$. Let 
\[s_q := 192\sqrt{\frac{\log(3T/\delta) + 3\log(2T(2+\Upsilon^2))}{q}}\] be the decision threshold for each phase $q \geq L_2$ in Algorithm~\ref{alg:racing-two-types-general}. Assume that after the elimination, at every iteration a sample of the eliminated arm is also drawn, but not revealed to the agent.\\
We define the event $\cC$ as the accuracy guarantee of $\hat{\theta}$ such that:
\begin{equation}
\label{eq:event-C}
    \cC := \left\{ \forall q \geq L_2: |G - \hat{G}_q| < s_q \right\}
\end{equation}
where $L_2$ is the number of samples of each arm after running the sampling stage.\\
Let $\tau \in (0, 1)$. Fix phase $q \geq L_2$, and some agent $t$ in this phase. In order to prove that Algorithm~\ref{alg:racing-two-types-general} is BIC for agents of type 1, we want to show that 
\begin{equation}
    \label{eq:racing-bic-arm2}
    \E_{\cP_1}[G\vert z_p = \e_2]\Prob_{\cP_1}[z_p = \e_2] \geq \nu.
\end{equation}
From Corollary ~\eqref{cor:finite-sample}, with probability $\delta$ we have that
\begin{equation*}
    \Prob[\neg \cC \vert G] \leq \delta
\end{equation*} 
Therefore, since $G\geq -1$, we have: 
\begin{align*}
\label{eq:racing-bic}
    \E_{\cP_1}[G|z_p = \e_2]\Prob_{\cP_1}[z_p = \e_2] &= \E_{\cP_1}[G|z_p = \e_2, \cC]\Prob_{\cP_1}[z_p = \e_2, \cC] + \E_{\cP_1}[G|z_p = \e_2, \neg C]\Prob_{\cP_1}[z_p = \e_2, \neg C]\\
    &\geq \E_{\cP_1}[G|z_p = \e_2, \cC]\Prob_{\cP_1}[z_p = \e_2, \cC] - \delta
\end{align*}
We want to lower bound the first term. This can be done by splitting it into four cases based on the value of $G$. We have:

\begin{equation} 
    \begin{split}
    &\quad\E_{\cP_1}[G | z_p = \e_2, \cC]\Prob_{\cP_1}[z_p = \e_2, \cC]\\
    &=\E_{\cP_1}[G | z_p = \e_2, \cC, G \geq \tau]\Prob_{\cP_1}[z_p= \e_2, \cC, G \geq \tau] \\
    & \hspace{0.4cm} + \E_{\cP_1}[G | z_p = \e_2, \cC, 0 \leq G < \tau]\Prob_{\cP_1}[z_p = \e_2, \cC, 0 \leq G < \tau] \\
    &\hspace{0.4cm} + \E_{\cP_1}[G | z_p = \e_2, \cC, -2s_q < G < 0]\Prob_{\cP_1}[z_p = \e_2, \cC, -2s_q < G < 0] \\
    & \hspace{0.4cm} + \E_{\cP_1}[G | z_p = \e_2, \cC, G \leq -2s_q]\Prob_{\cP_1}[z_p = \e_2, \cC, G \leq -2s_q] \label{eq:racing-bic-cases}
    \end{split}
\end{equation}

Observe that, by definition of $s_q$, we have:
\begin{align*}
    2s_q &\leq 2s_{L_2}
    = \frac{384\sqrt{\log(3T/\delta) + 3\log(2T(2+\Upsilon^2))}}{384\sqrt{\log(2T/\delta) + 3\log(2T(2+\Upsilon^2))} \ } \left(\frac{ \tau \Prob_{\cP_1}[G \geq \tau]}{2} - \nu \right)\\
    &= \frac{\tau \Prob_{\cP_1}[G \geq \tau]}{2} -\nu\\
    &\leq \tau
\end{align*}

Conditional on $\cC$, the empirical estimate $\hat{G}_q > G - s_q \geq 2s_q$. Hence, when we have $G \geq \tau \geq 2s_q$, then $G=\theta^2 - \theta^1 \geq 2s_q$ and arm 1 must have already been eliminated at phase $q \geq L_2$. This implies that the probability $\Prob_{\cP_1}[z_p = \e_2, \cC, G\geq \tau] = \Prob_{\cP_1}[\cC, G\geq \tau]$. Similarly, when we have $G \leq -2s_q$, then $\theta^2 - \theta^1 \leq -2s_q$ and arm 2 must have already been eliminated at phase $q \geq L_2$. Hence, arm 2 could not be recommended in that case and the probability $\Prob_{\cP_1}[z_p = \e_2, \cC, G\leq-2s_q] = 0$.\\
We can then rewrite equation~\eqref{eq:racing-bic-cases} as
\begin{align*}
    &\quad\E_{\cP_1}[G | z_p = \e_2, \cC]\Prob_{\cP_1}[z_p = \e_2 ,\cC]\\ &\geq \E_{\cP_1}[G | z_p = \e_2, \cC, G \geq \tau]\Prob_{\cP_1}[z_p= \e_2, \cC, G \geq \tau]\\
    & \hspace{.4cm}+ \E_{\cP_1}[G | z_p = \e_2, \cC, 0 \leq G < \tau]\Prob_{\cP_1}[z_p = \e_2, \cC, 0 \leq G < \tau]\\
    & \hspace{.4cm}+ \E_{\cP_1}[G | z_p = \e_2, \cC, -2s_q < G < 0]\Prob_{\cP_1}[z_p = \e_2, \cC, -2s_q < G < 0]\\
    &\geq \tau \Prob_{\cP_1}[\cC, G \geq \tau] + 0\cdot \Prob_{\cP_1}[\cC, 0 \leq G < \tau] -2s_q \Prob_{\cP_1}[z_p = \e_2, \cC, -2s_q<G<0]\\
    &\geq \tau \Prob_{\cP_1}[\cC, G \geq \tau] - 2s_q\\
    &\geq \tau \Prob_{\cP_1}[\cC, G \geq \tau] - \frac{\tau \Prob_{\cP_1}[G \geq \tau]}{2} + \nu\\
    &\geq \tau \Prob_{\cP_1}[\cC | G \geq \tau] \Prob_{\cP_1}[G \geq \tau] - \frac{\tau \Prob_{\cP_1}[G \geq \tau]}{2} + \nu\\
    &\geq \tau (1 - \delta) \Prob_{\cP_1}[G \geq \tau] - \frac{\tau \Prob_{\cP_1}[G \geq \tau]}{2} + \nu\\
    &=\left(\frac{1}{2} - \delta \right) \tau \Prob_{\cP_1}[G \geq \tau] + \nu\\
    &\geq \left(\frac{1}{2} - \delta \right) \tau \Prob_{\cP_1}[G \geq \tau] + \nu\\
    &= \left(\frac{1}{2} - \frac{\frac{1}{2} \tau \Prob_{\cP_1}[G \geq \tau]}{\tau \Prob_{\cP_1}[G \geq \tau] + 1} \right) \tau \Prob_{\cP_1}[G \geq \tau] + \nu\\
    &= \frac{1}{2} \left(\frac{\tau \Prob_{\cP_1}[G\geq \tau] + 1 - \tau \Prob_{\cP_1}[G\geq \tau]}{\tau \Prob_{\cP_1}[G\geq \tau] + 1} \right)\tau \Prob_{\cP_1}[G\geq \tau] + \nu\\
    &= \frac{1}{2} \left(\frac{\tau \Prob_{\cP_1}[G\geq \tau]}{\tau \Prob_{\cP_1}[G\geq \tau] + 1} \right)  + \nu\\
    &= \delta_\tau + \nu\\
    &\geq \delta  + \nu.
\end{align*}
Hence, we have 
\begin{align*}
    \E_{\cP_1}[G|z_p = \e_2]\Prob_{\cP_1}[z_p = \e_2] &\geq \E[G|z_p = \e_2, \cC]\Prob_{\cP_1}[z_p = \e_2, \cC] - \delta\\
    &\geq \delta + \nu -  \delta \\
    &= \nu
\end{align*}
Therefore, the second stage of Algorithm~\ref{alg:racing-two-types-general} fulfills equation~\eqref{eq:racing-bic-arm2} and is BIC for agents of type 1. 

Note that we restrict the priors of type 1 and type 2 such that $\delta_\tau^1 < \delta_\tau^2$. Then, with the same constant $\tau$, the BIC conditions for agents of type 2 is also satisfied, and we achieve a fully BIC algorithm.
\end{proof}

\typespecifictwoarmsgeneral*

\begin{proof}
The regret of our algorithm, as given by Lemma~\eqref{lemma:ex-post-2-arm} is 
\begin{equation}
\label{eq:ex-post-2-arm}
    R(T) \leq L_2 \rho + O(\sqrt{T\log(T/\delta)}) 
\end{equation}
where $L_2$ is the number of arm 2 samples collected in the sampling stage, $\rho$ is the number of phases in the sampling stage and $\delta$ is the accuracy guarantee of our estimate $\hat{\theta}$.\\
Let $L_1$ be the number of samples needed to make agents of type 1 follow our recommendation for arm 2. Half of the population is agents of type 1 and the other half is agents of type 2. We can derive type-specific regret for each type of agents using our algorithm conditioned on which arm is the best arm overall.
\begin{enumerate}
    \item If arm 1 is the best arm overall:\\
    Type 1 regret: Since agents of type 1 only take arm 1 until the algorithm has collected at least $L_1$ samples of arm 2, they accumulate no regret throughout the sampling stage and the first part of the racing stage when the algorithm is only BIC for agents of type 2. Hence, the regret for type 1 is then just the regret accumulated in the second part of the racing stage. 
    \begin{align}
        R_1 &\leq 0.5(2hq - L_1 + L_2)\Delta \\
        &\leq O(\log(T/\delta))
    \end{align}
    Type 2 regret: Since our algorithm guarantees that agents of type 2 will always follow our recommendation, the regret of agents of type 2 is derived similarly to the ex-post regret in \cref{lemma:ex-post-2-arm}:
    \begin{equation}
        R_2 \leq 0.5L_2 + O(\sqrt{T\log(T/\delta)})    
    \end{equation}
    \item If arm 2 is the best arm overall:\\
    Type 1 regret: Since agents of type 1 only start taking our recommendation for arm 2 during the second part of the racing stage, the regret of type 1 is then the regret accumulated by all agents of type 1 in the sampling stage, the first part of the racing stage and the regret accumulated after agents of type 1 start taking our recommendation for arm 2. 
    \begin{align}
        R_1 &\leq 0.5L_2 \rho \Delta + (L_1 - L_2)h\Delta\\
        & \hspace{0.4cm}+ \left(\frac{147456 (\log(3T/\delta) + 3\log(2T(2+\Upsilon^2)))}{\Delta^2} - L_1\right)h\Delta\\
        &\leq 0.5L_2 \rho + O\left(\frac{\log(T/\delta)}{\tau^2\Prob_{\cP_1}[G \geq \tau]^2}\right) + O(\sqrt{T\log(T/\delta)})
    \end{align}
    Type 2 regret: Similar to the case where arm 1 is the best arm overall, the regret for agents of type 2 can be derived from the ex-post regret in Lemma~\eqref{lemma:ex-post-2-arm}
    \begin{align}
        R_2 \leq 0.5 L_2 \rho + O(\sqrt{T\log(T/\delta)})
    \end{align}
\end{enumerate}
\end{proof}

\subsection{Ex-Post Regret} The ex-post regret conditional on $\neg\cC$ is at most $T(\delta + \delta')$.

Assume that $\cC$ holds. Let $\Delta = |\theta^1 - \theta^2|$. Observe that since $\cC$ holds, we have $\Delta \leq |\hat{G}_q| + s_q$ where $s_q$ is the decision threshold of phase $q$. Before the stopping criteria is invoked, we also have $|\hat{G}_q| \leq s_q$. 
Hence, we have: 
\begin{align*}
     \Delta \leq 2 s_q &= 384\sqrt{\frac{\log(3T/\delta) + 3\log(2T(2+\Upsilon^2))}{q}}\\
     \Rightarrow \frac{\Delta}{384\sqrt{\log(3T/\delta) + 3\log(2T(2+\Upsilon^2))}} &\leq \frac{1}{\sqrt{q}}\\
     \Rightarrow q &\leq \frac{147456 (\log(3T/\delta) + 3\log(2T(2+\Upsilon^2)))}{\Delta^2}
\end{align*}

In the racing stage, we recommend each arm $h$ times in a single phase. In the first part of the racing stage, only agents of type 2 are fully compliant; agents of type 1 only take arm 1. If arm 1 is best, then the worst-case regret occurs when an agent of type 2 appears every round arm 2 is recommended. Thus, the regret of single phase is at most $h\Delta$ if arm 1 is best. If arm 2 is best, then the worst case occurs when no agent of type 2 appears when arm 2 is recommended. In this case, we get no samples of arm 2 and the regret is at most $2h\Delta$. In the second part of the racing stage, all agents are fully compliant. Thus, the regret in a single phase here is simply $h\Delta$. Thus, in any phase of the racing stage, the regret is always less than or equal to $2h\Delta$.

The racing stage runs from phase $L_2$ until the stopping criterion. Thus, the total regret for the racing stage \cref{alg:racing-two-types-general} is bounded as such:
\begin{align}
    R_{\text{racing}} &\leq \left(\frac{147456 (\log(3T/\delta) + 3\log(2T(2+\Upsilon^2)))}{\Delta^2} - L_2\right)2h\Delta \nonumber \\
    &\leq \frac{294912h(\log(3T/\delta) + 3\log(2T(2+\Upsilon^2)))}{\Delta}.
\end{align}

After the stopping criterion is invoked, we have found the best arm and we no longer accumulate any regret.
 
Observe that the ex-post regret for each round $t$ of the entire algorithm (both the sampling stage and the racing stage) is at most that of the racing stage plus $\Delta$ per each round of the sampling stage. Alternatively, we can also upper bound the regret by $\Delta$ per each round of the algorithm. Therefore, we can derive the ex-post regret for the entire algorithm:
If arm 1 is the best arm, then the total regret of both \cref{alg:sampling-two-types-general} and \cref{alg:racing-two-types-general} is:
\begin{align}
    R(T) &\leq \min \left \{L_2\Delta + \frac{294912h(\log(3T/\delta)+3\log(2T(2+\Upsilon^2)))}{\Delta}, T\Delta \right \}\\
    &\leq L_2 + O(\sqrt{T\log(T/\delta)}).
\end{align}
If arm 2 is the best arm, then the total regret of both
\cref{alg:sampling-two-types-general} and \cref{alg:racing-two-types-general} is:
\begin{align}
    R(T) &\leq \min \left \{L_2\rho\Delta + \frac{294912h(\log(3T/\delta)+3\log(2T(2+\Upsilon^2)))}{\Delta}, T\Delta \right \}\\
    &\leq L_2\rho + O(\sqrt{T\log(T/\delta)}).
\end{align}

\section{Gaussian Example Proof}
Recall \cref{ex:gaussian}:
\gaussian*
\begin{proof}
We analyze this example for the sampling stage and the racing stage separately. 
\begin{itemize}
    \item The sampling stage:\\
    Suppose that, in the sampling stage, an agent of type 1 is recommended arm 2. This means that either $\E_{\cP_2}[\theta^2 - \theta^1 | z_t = e_2] \geq 0$ or the agent is in the exploration set Q. Since the agent knows that they are not type 2 and knows that the prior is over the prior of type 2, the recommendation is not enough to make them take arm 2:
    \begin{equation}
        \E_{\cP_1}[\theta^2 - \theta^1 | z_t = e_2] < 0.
    \end{equation}
    Let $\xi_2$ denote the event where the mean reward $\bar{y}^1_t$ of arm 1 from phase 1 is much smaller than the prior mean reward $\mu^2_2$, i.e.
    \begin{equation}
        \xi_2 := \left\{ \E_{\cP_2}[\theta^1 | y^1_1, \dots, y^1_{L_2}] < \mu^2_2 \right\}.
    \end{equation}
    Now, suppose that an agent of type 2 is recommended arm 2. They know that this either means that event $\xi_2$ has happened and $\E_{\cP_2}[\theta^2 - \theta^1 | z_t = e_2] \geq 0$ or that the agent is in the exploration group $Q$. They know that the social planner has chosen some exploration probability $\rho$ such that 
    \begin{equation}
        \rho \geq 1 + \frac{4(\mu_2^1 - \mu_2^2)}{\Prob_{\cP_i}[\xi_i]}.
    \end{equation}
    
   The social planner needs to calculate the probability of event $\xi_2$, i.e.
    \begin{equation}
        \Prob_{\cP_2}[\xi_2] = \Prob_{\cP_2}[\E_{\cP_2}[\theta^1 | y^1_1, \dots, y^1_{L_2}] < \mu^2_2].
    \end{equation}
    In the worst case, the baseline reward $g(u_t) = -\Upsilon$ for all $L_2$ rounds of phase 1. Assume this worst case, the reward for pulling arm 1 is 
    \begin{align}
        y^1_t = \theta^1 - \Upsilon + \epsilon_t
    \end{align}
    Let $\hat{y}^1_t = y^1_t + \Upsilon = \theta^1 + \epsilon^1_t$. In this case, the expected posterior 
    \begin{equation}
        \E_{\cP_2}[\theta^1|y^1_1, \dots, y^1_{L_2}] = \E_{\cP_2}[\theta^1|\hat{y}^1_1, \dots, \hat{y}^1_{L_2}]
    \end{equation}
    Under this assumption, the error $\epsilon_t \sim \cN(0, \rho_{1.2}^2)$ and $\theta^1 = \mu^1_2 + \zeta^1_2$ for $\zeta^1_2 \sim \cN(0, \sigma^2_{1,2})$. Thus, the reward $\hat{y}^1_t \sim \cN(\theta^1, \rho^2_{1,2})$ and the expected posterior 
    \begin{equation}
        \E_{\cP_2}[\theta^1|\hat{y}^1_1, \dots, \hat{y}^1_{L_2}] \sim \cN\left(\mu^1_2,\ \sigma^2_{1,2}\frac{L_2 \sigma^2_{1,2}}{\rho^2_{1,2} + L_2 \sigma^2_{1,2}}\right)
    \end{equation}
    Let the z-score $\zeta^2 := (\mu^2_2 - \mu^1_2)\left(\sigma^2_{1,2}\frac{L_2 \sigma^2_{1,2}}{\rho^2_{1,2} + L_2 \sigma^2_{1,2}}\right)^{-1/2}$. Then, we have
    \begin{align}
        \Prob_{\cP_2}[\E_{\cP_2}[\theta^1|\hat{y}^1_1, \dots, \hat{y}^1_{L_2}] \leq \mu^2_2] = \phi(\zeta^2) = \int_{-\infty}^{\zeta^2} \frac{1}{\sqrt{2\pi}} \exp\left(\frac{-1}{2}u^2\right) du.
    \end{align}
    Furthermore, for any sequence of samples $y^1_1, \dots, y^1_{L_2}$ from phase 1, the expected posterior 
    \begin{equation}
        \E_{\cP_2}[\theta^1|y^1_1, \dots, y^1_{L_2}] \leq \E_{\cP_2}[\theta^1|\hat{y}^1_1, \dots, \hat{y}^1_{L_2}].
    \end{equation}
    Hence, 
    \begin{align*}
        \Prob[\xi_2] &= \Prob_{\cP_1}[\E_{\cP_1}[\theta^1| y^1_1, \dots, y^1_{L_2}] \leq \mu^2_2] \geq \Prob_{\cP_1}[\E_{\cP_1}[\theta^1|\hat{y}^1_1, \dots, \hat{y}^1_{L_2}] \leq \mu^2_2]\\
        &= \int_{-\infty}^{\zeta^2} \frac{1}{\sqrt{2\pi}} \exp\left(\frac{-1}{2}u^2\right) du.
    \end{align*}
    Since $\mu^2_1 - \mu^1_1 < \mu^2_2 - \mu^2_1$, we have $\zeta_1 < \zeta_2$ and hence $\Prob[\xi_1] < \Prob[\xi_2]$. Therefore, the minimum number of phases in the sampling stage needed to convince agents of type 1 is greater than that of type 2, i.e. $\rho' > \rho$. We would need to run the sampling stage for longer if we wanted to make agents of type 1 also comply to the algorithm's recommendation for arm 2.
    \item The racing stage:
    In the first racing stage, only agents of type 2 comply with our recommendation for arm 2. Hence, when an agent of type 1 receives a recommendation for arm 2, this recommendation is not enough to convince them to follow our recommendation for arm 2. Hence, we have 
    \begin{equation}
        \E_{\cP_1}[\theta^2 - \theta^1 | z_t = e_2] = \E_{\cP_1}[\theta^2 - \theta^1] < 0.
    \end{equation}
    When an agent of type 2 receives a recommendation for arm 2, they would think that either arm 2 is definitely the best arm or the two arms are still racing against each other. Agents of type 2 know that the racing stage only starts when the social planner has collected sufficient samples of arm 2 in the sampling stage:
    \begin{equation}
        L_2 \geq \frac{589824(\log(3T/\delta) + 3\log(2T(2+\Upsilon^2)))}{\tau^2 (\Prob_{\cP_2}[\theta^2 - \theta^1 \geq \tau]^2)}
    \end{equation}
    and 
    \begin{equation}
        \delta < \delta_{\tau, 2} = \frac{\tau \Prob_{\cP_2}[\theta^2 - \theta^1 \geq \tau]}{2\tau \Prob_{\cP_2}[\theta^2 - \theta^1 \geq \tau] + 2}
    \end{equation}
    The constant that the social planner needs to calculate is then $\tau \Prob_{\cP_2}[\theta^2 - \theta^1 > \tau]$ for some fixed constant $\tau \in (0,1)$.\\
    Assume that we have Gaussian priors. Hence, we have 
    \begin{equation}
        \theta^2 - \theta^1 \sim \cN(\mu^2_2 - \mu^1_2, \sigma^2_{1.2} + \sigma^2_{2,2})
    \end{equation}
    Let $\zeta_2 = \frac{\mu^2_2 - \mu^1_2 - \tau}{\sqrt{\sigma^2_{1,2} + \sigma^2_{1,2}}}$. Then, 
    \begin{align}
        \Prob_{\cP_2}[\theta^2 - \theta^1 > \tau] &= 1 - \Prob_{\cP_2}[\theta^2 - \theta^1 < \tau]\\
        &= 1 - \phi(\zeta_2)\\
        &= \int^\infty_{\zeta_2} \frac{1}{\sqrt{2\pi}} \exp\left(\frac{-1}{2} u^2\right) du
    \end{align}
    During the first racing stage, the algorithm collects more samples of arm 2, until we have enough samples to also make agents of type 1 comply with our recommendation for arm 2.\\
    When an agent of type 1 receives a recommendation for arm 2 during the second racing stage, they know that the number of arm 2 samples is at least
    \begin{equation}
        L_1 \geq \frac{589824(\log(3T/\delta) + 3\log(2T(2+\Upsilon^2)))}{\tau^2 (\Prob_{\cP_1}[\theta^2 - \theta^1 \geq \tau]^2)}
    \end{equation}
    Similar to the first racing stage, the social planner also needs to calculate the prior-dependent constant $\tau (\Prob_{\cP_1}[\theta^2 - \theta^1 \geq \tau]$.\\
    We have 
    \begin{equation}
        \theta^2 - \theta^1 \sim \cN(\mu^2_1 - \mu^1_1, \sigma^2_{1,1} + \sigma^2_{2,1})
    \end{equation}
    Let $\zeta_1 = \frac{\mu^2_1 - \mu^1_1 - \tau}{\sqrt{\sigma^2_{1,1} + \sigma^2_{2,1}}}$. Then, 
    \begin{align}
        \Prob_{\cP_1}[\theta^2 - \theta^1 > \tau] &= 1 - \Prob_{\cP_1}[\theta^2 - \theta^2 < \tau]\\
        &= 1 - \phi(\zeta_1)\\
        &= \int^\infty_{\zeta_1} \frac{1}{\sqrt{2\pi}} \exp\left(\frac{-1}{2} u^2\right) du
    \end{align}
    Also, we have 
    \begin{equation}
        \delta < \delta_{\tau, 1} =  \frac{\tau \Prob_{\cP_1}[\theta^2 - \theta^1 > \tau]}{2\tau \Prob_{\cP_1}[\theta^2 - \theta^1 > \tau] + 2}
    \end{equation}
    When an agent of type 2 receives a recommendation for arm 2, they would still comply since there are sufficient samples of arm 2 collected by the social planner (similar to the first racing stage).\\
    Since agents of type 1 prefer arm 1 more compared to agents of type 2, for a fixed constant $\tau \in (0,1)$, we have $\tau \Prob_{\cP_1}[\theta^2 - \theta^1 > \tau] < \tau\Prob_{\cP_2}[\theta^2 - \theta^1 > \tau]$. Hence, 
    \begin{equation}
        \delta_{\tau, 1} =  \frac{\tau \Prob_{\cP_1}[\theta^2 - \theta^1 > \tau]}{2\tau \Prob_{\cP_1}[\theta^2 - \theta^1 > \tau] + 2} < \frac{\tau \Prob_{\cP_2}[\theta^2 - \theta^1 > \tau]}{2\tau \Prob_{\cP_2}[\theta^2 - \theta^1 > \tau] + 2} = \delta_{\tau,2}
    \end{equation}
    Therefore, the social planner can pick $\delta < \delta_{\tau,1} < \delta_{\tau,2}$ in the second racing stage and satisfies both types' incentive-compatibility requirement.\\ 
    If we want to have a fully incentive-compatible algorithm in both the sampling stage and the racing stage, then we would need to collect at least $L_1$ samples of arm 2 in the samplings stage with the exploration probability $1/\rho'$ where 
    \begin{equation}
        \rho' \geq 1 + \frac{4(\mu_1^1 - \mu_1^2)}{\Prob[\xi_1]}
    \end{equation}
    Similar to how we derive the probability of $\xi_2$, we have the expected posterior 
    \begin{equation}
        \E_{\cP_1}[\theta^1|\hat{y}^1_1, \dots, \hat{y}^1_{L_2}] \sim \cN\left(\mu^1_1,\ \sigma^2_{1,1}\frac{L_2 \sigma^2_{1,1}}{\rho^2_{1,1} + L_2 \sigma^2_{1,1}}\right)
    \end{equation}
    Let the z-score $\zeta^1 := (\mu^2_1 - \mu^1_1)\left(\sigma^2_{1,1}\frac{L_2 \sigma^2_{1,1}}{\rho^2_{1,1} + L_2 \sigma^2_{1,1}}\right)^{-1/2}$. Then, we have
    \begin{equation}
        \Prob_{\cP_1}[\E_{\cP_1}[\theta^1|\hat{y}^1_1, \dots, \hat{y}^1_{L_2}] \leq \mu^2_1] = \phi(\zeta^1) = \int_{-\infty}^{\zeta^1} \frac{1}{\sqrt{2\pi}} \exp\left(\frac{-1}{2}u^2\right) du
    \end{equation}
     It is possible to modify the prior of type 1 such that the sampling stage of the fully BIC algorithm must be arbitrarily longer than the sampling stage of our partially BIC algorithm. In an extreme instance, the minimum length of the sampling stage for the fully BIC algorithm could be so long that it is impossible to make the algorithm incentive-compatible for agents of type 1 within the time horizon $T$. Suppose we have $\Prob_{\cP_1}[\theta^2 - \theta^1 > \tau] < \frac{1}{\sqrt{T}}$ for some $\tau \in (0, 1)$, then the number of arm 2 samples needed to make agents of type 1 comply in the racing stage is:
    \begin{align*}
        L_1 &\geq \frac{589824(\log(3T/\delta) + 3\log(2T(2+\Upsilon^2)))}{\tau^2 \left(\frac{1}{T} \right)}\\
        &= O(T)
    \end{align*}
    Hence, a fully incentive-compatible algorithm would not finish the sampling stage before the time horizon is up. Therefore, the regret accumulated for each type of agents would be linear.\\
    On the other hand, our algorithm only relies on agents of type 2 to take our recommendation during the sampling stage and the racing stage. Hence, if we have $\frac{1}{\sqrt{\log(T)}} > \Prob_{\cP_2}[\theta^2 - \theta^1 > \tau] > \frac{1}{\sqrt{T}} > \Prob_{\cP_1}[\theta^2 - \theta^1 > \tau]$, then the number of arm 2 samples needed to make agents of type 2 comply in the racing stage is:
    \begin{align*}
        L_2 &\geq \frac{589824(\log(3T/\delta) + 3\log(2T(2+\Upsilon^2)))}{\tau^2 (\Prob_{\cP_2}[\theta^2 - \theta^1 \geq \tau]^2)}\\
        &= O(\log(T))
    \end{align*}  
    Also, if we have the probability that for agents of type 2, the sample average of arm 1 in the first phase of the sampling stage is sufficiently smaller than the prior-mean reward of arm 2, ($\Prob[\xi_2]$) is larger than $\frac{1}{\sqrt{\log(T)}}$, then the number of phases in the sampling stage is:
    \begin{align*}
        \rho &> 1 + \frac{4(\mu^1_2 - \mu^2_2)}{\Prob[\xi_2]}\\
        &= O(\sqrt{\log(T)})
    \end{align*}
    Then, we would still achieve sub-linear regret for each type with our algorithm, while a fully incentive-compatible algorithm would stay in the sampling stage and achieve linear regret:
\end{itemize}
\begin{table}[ht!]
\centering
    \begin{tabular}{c|c|c|c|}
        \multicolumn{2}{c}{} & \multicolumn{2}{c}{Type}\\\cline{3-4}
         \multicolumn{1}{c}{} &  & Type 1 & Type 2 \\\cline{2-4}
         Best Arm & Arm 1 & $O(\log(T))$ & $O(\log(T))+O(\log(T))$ \\\cline{2-4}
         & Arm 2 & $O(\log(T)^{3/2}) + O(\sqrt{T\log(T)})$ & $O(\log(T)^{3/2}) + O(\sqrt{T\log(T)})$ \\\cline{2-4}
    \end{tabular}
    \caption{Example: Type-Specific Regret for Two Arms \& Two Types with Partially-BIC Algorithm}
    \label{tab:type-specific-regret-example}
\end{table}
\end{proof}

\newpage

\textbf{Beta-binomial racing stage}:
In the first part of the racing stage, only agents of type 2 comply with our recommendation for arm 2. Hence, when an agent of type 1 receives a recommendation for arm 2, this recommendation is not enough to convince them to follow our recommendation for arm 2. Hence, we have 
\begin{equation}
    \E_{\cP_1}[\theta^2 - \theta^1 | z_t = e_2] = \E_{\cP_1}[\theta^2 - \theta^1] < 0.
\end{equation}
When an agent of type 2 receives a recommendation for arm 2, they would think that either arm 2 is definitely the best arm or the two arms are still racing against each other. Agents of type 2 know that the racing stage only starts when the social planner has collected sufficient samples of arm 2 in the sampling stage:
\begin{equation}
    L_2 \geq \frac{589824(\log(3T/\delta) + 3\log(2T(2+\Upsilon^2)))}{\tau^2 (\Prob_{\cP_2}[\theta^2 - \theta^1 \geq \tau]^2)}
\end{equation}
and 
\begin{equation}
    \delta < \delta_{\tau, 2} = \frac{\tau \Prob_{\cP_2}[\theta^2 - \theta^1 \geq \tau]}{2\tau \Prob_{\cP_2}[\theta^2 - \theta^1 \geq \tau] + 2}
\end{equation}
The constant that the social planner needs to calculate is then $\tau \Prob_{\cP_2}[\theta^2 - \theta^1 > \tau]$ for some fixed constant $\tau \in (0,1)$.\\

Suppose that the agents have beta prior distributions on the mean rewards of each arm, i.e. 
\[ \theta^1 \sim \text{Beta}(\alpha_1^i,\beta_1^i) \ \text{ and } \ \theta^2 \sim \text{Beta}(\alpha_2^i,\beta_2^i)\] for each prior $i\in\{1,2\}$. Thus, for a given type $i$, the prior on the difference between arm 2 and arm 1 is given as:
\[\theta^2-\theta^1\sim\text{Beta}(\alpha_2^i,\beta_2^i)*\left(-\text{Beta}(\alpha_1^i,\beta_1^i)\right),\]
which has the probability density function
\begin{align*}
    &-\int_{-\infty}^\infty \frac{\Gamma(\alpha_1^i+\beta_1^i)}{\Gamma(\alpha_1^i)\Gamma(\beta_1^i)} \frac{\Gamma(\alpha_2^i+\beta_2^i)}{\Gamma(\alpha_2^i)\Gamma(\beta_2^i)}(\theta^2-\theta^1-x)^{\alpha_1^i-1}(1-\theta^2+\theta^1+x)^{\beta_1^i-1}x^{\alpha_2^i-1}(1-x)^{\beta_2^i-1} \ dx\\
    &= \frac{-\Gamma(\alpha_1^i+\beta_1^i)}{\Gamma(\alpha_1^i)\Gamma(\beta_1^i)} \frac{\Gamma(\alpha_2^i+\beta_2^i)}{\Gamma(\alpha_2^i)\Gamma(\beta_2^i)} \int_{-1}^1 (\theta^2-\theta^1-x)^{\alpha_1^i-1}(1-\theta^2+\theta^1+x)^{\beta_1^i-1}x^{\alpha_2^i-1}(1-x)^{\beta_2^i-1} \ dx,
\end{align*} 

where the gamma function $\Gamma(z) = \int_0^\infty x^{z-1}\e^{-x}\ dx$ and the integral in the last line is restricted to the interval $[-1,1]$ since both beta distributions are supported on $[0,1]$.

Then, for prior $i$, the probability that the difference $G:=\theta^2-\theta^1$ is greater than $\tau$ is given by:
\begin{align*}
    \Prob_{\cP_i}[G\geq\tau] = \int_\tau^1\frac{-\Gamma(\alpha_1^i+\beta_1^i)}{\Gamma(\alpha_1^i)\Gamma(\beta_1^i)} \frac{\Gamma(\alpha_2^i+\beta_2^i)}{\Gamma(\alpha_2^i)\Gamma(\beta_2^i)} \int_{-1}^1 (G-x)^{\alpha_1^i-1}(1-G+x)^{\beta_1^i-1}x^{\alpha_2^i-1}(1-x)^{\beta_2^i-1} \ dx\,dG\\
    =\frac{-\Gamma(\alpha_1^i+\beta_1^i)}{\Gamma(\alpha_1^i)\Gamma(\beta_1^i)} \frac{\Gamma(\alpha_2^i+\beta_2^i)}{\Gamma(\alpha_2^i)\Gamma(\beta_2^i)} \int_\tau^1\int_{-1}^1 (G-x)^{\alpha_1^i-1}(1-G+x)^{\beta_1^i-1}x^{\alpha_2^i-1}(1-x)^{\beta_2^i-1} \ dx\,dG\\
\end{align*}

It is possible to modify the prior of type 1 such that the sampling stage of the fully BIC algorithm must be arbitrarily longer than the sampling stage of our partially BIC algorithm. In an extreme instance, the minimum length of the sampling stage for the fully BIC algorithm could be so long that it is impossible to make the algorithm incentive-compatible for agents of type 1 within the time horizon $T$. Suppose we have $\Prob_{\cP_1}[\theta^2 - \theta^1 > \tau] < \frac{1}{\sqrt{T}}$ for some $\tau \in (0, 1)$, then the number of arm 2 samples needed to make agents of type 1 comply in the racing stage is:
    \begin{align*}
        L_1 &\geq \frac{589824(\log(3T/\delta) + 3\log(2T(2+\Upsilon^2)))}{\tau^2 \left(\frac{1}{T} \right)}\\
        &= O(T)
    \end{align*}
    Hence, a fully incentive-compatible algorithm would not finish the sampling stage before the time horizon is up. Therefore, the regret accumulated for each type of agents would be linear.\\
    On the other hand, our algorithm only relies on agents of type 2 to take our recommendation during the sampling stage and the racing stage. Hence, if we have $\frac{1}{\sqrt{\log(T)}} > \Prob_{\cP_2}[\theta^2 - \theta^1 > \tau] > \frac{1}{\sqrt{T}} > \Prob_{\cP_1}[\theta^2 - \theta^1 > \tau]$, then the number of arm 2 samples needed to make agents of type 2 comply in the racing stage is:
    \begin{align*}
        L_2 &\geq \frac{589824(\log(3T/\delta) + 3\log(2T(2+\Upsilon^2)))}{\tau^2 (\Prob_{\cP_2}[\theta^2 - \theta^1 \geq \tau]^2)}\\
        &= O(\log(T))
    \end{align*}  
    Also, if we have the probability that for agents of type 2, the sample average of arm 1 in the first phase of the sampling stage is sufficiently smaller than the prior-mean reward of arm 2, ($\Prob[\xi_2]$) is larger than $\frac{1}{\sqrt{\log(T)}}$, then the number of phases in the sampling stage is:
    \begin{align*}
        \rho &> 1 + \frac{4(\mu^1_2 - \mu^2_2)}{\Prob[\xi_2]}\\
        &= O(\sqrt{\log(T)})
    \end{align*}
    Then, we would still achieve sub-linear regret for each type with our algorithm, while a fully incentive-compatible algorithm would stay in the sampling stage and achieve linear regret:
\begin{table}[ht!]
\centering
    \begin{tabular}{c|c|c|c|}
        \multicolumn{2}{c}{} & \multicolumn{2}{c}{Type}\\\cline{3-4}
         \multicolumn{1}{c}{} &  & Type 1 & Type 2 \\\cline{2-4}
         Best Arm & Arm 1 & $O(\log(T))$ & $O(\log(T))+O(\log(T))$ \\\cline{2-4}
         & Arm 2 & $O(\log(T)^{3/2}) + O(\sqrt{T\log(T)})$ & $O(\log(T)^{3/2}) + O(\sqrt{T\log(T)})$ \\\cline{2-4}
    \end{tabular}
    \caption{Example: Type-Specific Regret for Two Arms \& Two Types with Partially-BIC Algorithm}
    \label{tab:type-specific-regret-example}
\end{table}
